# Supplementary material for: Towards R-learner with Continuous Treatments
Source: arXiv:2208.00872 source file (2025-04-17)
Supplement: Supplementary file 1 [file supp.pdf]

# Supplementary material for “Towards R-learner of conditional average treatment effects with a continuous treatment: T-identification, estimation, and inference”

BY YICHI ZHANG

*Department of Statistics, North Carolina State University, 5109 SAS Hall, 2311 Stinson Drive,  
Raleigh, North Carolina 27695, U.S.A.*  
yzhan239@ncsu.edu

5

DEHAN KONG

*Department of Statistical Sciences, University of Toronto, 700 University Avenue,  
Toronto, Ontario M5G 1Z5, Canada*  
dehan.kong@utoronto.ca

10

SHU YANG

*Department of Statistics, North Carolina State University, 5109 SAS Hall, 2311 Stinson Drive,  
Raleigh, North Carolina 27695, U.S.A.*  
syang24@ncsu.edu

15

## SUMMARY

The supplementary material contains a generalized cross validation-based method for tuning parameter selection, generalized S- and X-learning algorithms, simulation details, and technical details and proofs of theoretical results in the main text.

## S1. GENERALIZED CROSS VALIDATION-BASED TUNING PARAMETER SELECTION

20

Parameters  $K$  and  $\rho$  for our sieve-type  $\ell_2$ -penalized R-learner (Algorithm ??) control the bias-variance tradeoff. An essential problem in practice is how to select the optimal  $K$  and  $\rho$  based on samples and minimize the finite-sample error. For sieve-type estimators, many data-driven methods have been considered to select the optimal number of basis functions, including AIC, BIC, cross validation, Lepski's method, Mallows criterion. We refer interested readers to [Ichimura & Todd \(2007\)](#); [Hansen \(2014\)](#) for reviews.

25

In this section, we adapt the generalized cross validation ([Golub et al., 1979](#)) as the parameter selection method for our sieve-type  $\ell_2$ -penalized R-learner. The generalized cross validation is known to be efficient and valid in many model selection problems. In comparison to ad-hoc cross validation methods that have been popularly studied for sieve-type estimators ([Belloni et al., 2015, 2019](#)), the generalized cross validation is preferable under our framework as it permits a closed-form solution and avoids introducing additional computational complexity.

30

For given samples  $\{Z_i\}_{i=1}^n$ , we first set the candidate pool for relative parameters  $K$  and  $\rho$

$$\mathcal{L} = \{(K, \rho) \mid K = K_1, \dots, K_{n_1}, \rho = \rho_1, \dots, \rho_{n_2}\}.$$

Following the convention and without loss of generality, we assume that for each  $K = K_a$  with  $a \in [n_1]$ , the corresponding basis function  $\Psi(x, t)$  is determined. We then select the optimal  $(K, \rho)$  from  $\mathcal{L}$  by the generalized cross validation. Recalling that in Algorithm ??, we split the full data into  $\mathcal{J}$

---

**Algorithm S1. Generalized S-learner and X-learner for continuous treatments**


---

*Step 1.* Obtain  $\hat{\mu}(x, t) = \hat{E}(Y \mid X = x, T = t)$  over all  $\{Z_i\}_{i=1}^n$  via a flexible machine learning algorithm;

*Step 2.* S- and X-learners proceed as follows.

- (S-learner). Obtain  $\hat{\tau}_{SL}(x, t) = \hat{\mu}(Y \mid X = x, T = t) - \hat{\mu}(Y \mid X = x, T = 0)$ ;
- (X-learner). Construct pseudo-individual treatment effect  $D_i = Y_i - \hat{\mu}(X_i, 0)$ , based on which fit

$$\hat{\tau}_{XL}(x, t) = \hat{E}(D \mid X = x),$$

via a flexible machine learning algorithm.

---

35 folds  $\mathcal{S}_1, \dots, \mathcal{S}_{\mathcal{J}}$  with sample sizes  $n_1, \dots, n_{\mathcal{J}}$ , respectively. Without loss of generality, we assume  $\mathcal{S}_j = \{Z_{1+\sum_{l=1}^{j-1} n_l}, \dots, Z_{\sum_{l=1}^j n_l}\}$  for each  $j = 1, \dots, \mathcal{J}$ .

Given specific  $(K, \rho) = (K_a, \rho_b) \in \mathcal{L}$ , we define the following quantities:

$$\begin{aligned} Y &= (Y_1, \dots, Y_n)^T \\ \hat{m} &= \{\hat{m}^{(1)}(X_1), \dots, \hat{m}^{(\mathcal{J})}(X_n)\}^T \\ \Lambda &= \{\Psi(X_1, T_1) - \hat{\Gamma}^{(1)}(X_1), \dots, \Psi(X_n, T_n) - \hat{\Gamma}^{(\mathcal{J})}(X_n)\} \\ \hat{\tau} &= \{\hat{\phi}^T \Psi(X_1, T_1) - \hat{\phi}^T \hat{\Gamma}^{(1)}(X_1), \dots, \hat{\phi}^T \Psi(X_n, T_n) - \hat{\phi}^T \hat{\Gamma}^{(\mathcal{J})}(X_n)\}^T, \end{aligned}$$

for all  $j \in [\mathcal{J}]$ . Based on Algorithm ??, we then write

$$\hat{\tau} = \underbrace{n^{-1} \Lambda^T \hat{G}_n^{-1} \Lambda}_{S_{(K_a, \rho_b)}} (Y - \hat{m}), \quad (\text{S1})$$

40 where  $S_{(K_a, \rho_b)}$  is the so-called smoothing matrix of the generalized cross-validation for a particular parameter group  $(K_a, \rho_b)$ ; see, e.g., Wasserman (2006, Section 5.3). Following Wasserman (2006), the corresponding empirical error criterion for the generalized cross-validation is

$$\text{Error}(K_a, \rho_b) = \frac{1}{n} \sum_{i=1}^n \left[ \frac{Y_i - \hat{m}^{(j_i)}(X_i) - \{\hat{\phi}^T \Psi(X_i, T_i) - \hat{\phi}^T \hat{\Gamma}^{(j_i)}(X_i)\}}{1 - \text{tr}\{S_{(K_a, \rho_b)}\}/n} \right]^2, \quad (\text{S2})$$

where  $j_i$  is the splitting fold of  $i$ th sample. Finally, we choose the optimal  $(K, \rho)$  among  $\mathcal{L}$  that minimizes (S2).

## S2. GENERALIZED S- AND X-LEARNERS

45 Künzel et al. (2019) described two meta-learners for conditional average treatment effect estimation under the binary-treatment scenario; namely, the S- and X-learners. Algorithm S1 extends S- and X-learners to the continuous-treatment case.

## S3. SIMULATION DETAILS FOR FIG.??

We simulate two data examples with one binary-treatment setting and one continuous-treatment setting, 50 respectively. In both examples, the sample size is  $n = 1000$ .

- (A binary-treatment setting) Generate a single covariate  $X_i \sim \text{Uniform}(0, 1)$ , a binary treatment  $T_i \sim \text{Bernoulli}(0.5)$ , and  $Y_i = \sin(2X_i) + X_i^2 + \tau(X_i, T_i) + \varepsilon_i$  with  $\tau(X_i, 0) = 0$ ,  $\tau(X_i, 1) = \tau(X_i) = \sin(2\pi r_i + \pi/2) + 1$ ,  $r_i = |X_i - 0.5|$ , and  $\varepsilon_i \mid X_i, T_i \sim \mathcal{N}(0, 0.3^2)$ .

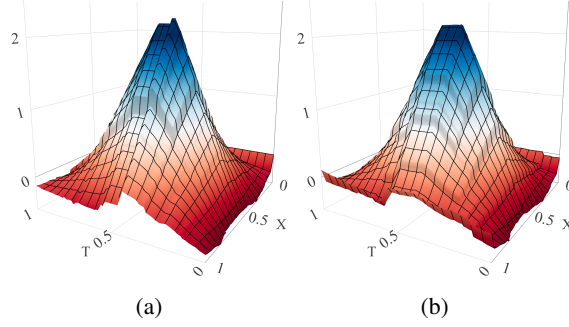

Fig. S1: When the treatment is continuous, the generalized S-learner (Panel a) and the generalized X-learner (Panel b) roughly captures  $\tau(x, t)$  (Fig. ??b). However, their performances are not as good as the proposed R-learner (Fig. ??d).

- (A continuous-treatment setting) Generate a single covariate  $X_i \sim \text{Uniform}(0, 1)$ , a continuous treatment  $T_i \sim \text{Uniform}(0, 1)$ , and  $Y_i = \sin(2X_i) + X_i^2 + \tau(X_i, T_i) + \varepsilon_i$  with  $\tau(X_i, T_i) = I(r'_i \leq 0.5) \{ \sin(2\pi r'_i + \pi/2) + 1 \}$ ,  $r'_i$  the Euclidian distance between  $(X_i, T_i)$  and  $(0.5, 0.5)$ , and  $\varepsilon_i | X_i, T_i \sim \mathcal{N}(0, 0.3^2)$ . Here  $I(\cdot)$  is the indicator function.

Both settings can be seen as completely randomized experiments. For the binary-treatment setting, we approximate  $\tau(x, t = 1) = \tau(x)$ , with a 5-dimensional B-spline basis  $\psi(x)$  such that  $\tau(x) \approx \phi^T \psi(x)$ . The  $\psi(\cdot)$  has equally-spaced knots over  $[0, 1]$ ; see §S5.2 for more details of B-splines. We construct the empirical analogy of the binary-treatment R-loss  $L_b(h)$  in (??), with  $h(x) = \phi^T \psi(x)$  and the true nuisance functions. We then estimate  $\hat{\tau}(x) = \hat{\phi}_b^T \psi(x)$  as the minimum of this empirical R-loss.

For the continuous-treatment setting, we use a 25-dimensional tensor-productive B-spline function  $\Psi(x, t)$  to approximate  $\tau(x, t)$ , where  $\Psi(x, t) = \psi(t) \otimes \psi(x)$  and  $\psi(\cdot)$  is defined in the same way as before. Specifically, the empirical analogy of our generalized R-loss  $L_c(h)$  in (??) is constructed with  $h(x, t) = \phi^T \Psi(x, t)$  and the true nuisance functions. The simple generalized R-learner  $\hat{\tau}_{\text{naive}}(x, t) = \hat{\phi}_c^T \Psi(x, t)$  is the minimum of this empirical generalized R-loss.

We also apply our proposed estimator in Algorithm ?? with sieve approximation on the data generated under the continuous-treatment setting. For simplicity, we do not impose sample splitting, i.e., set  $\mathcal{J} = 1$ . We use the same B-spline basis functions  $\Psi(x, t)$  as the simple generalized R-learner  $\hat{\tau}_{\text{naive}}(x, t)$ . Nuisance functions are trained via strategy (i) based on the SUPERLEARNER, which is considered in the simulation study in §??. The  $\rho$  is set to be 0.05.

Finally, we assess the generalized S- and X-learners defined in Algorithm S1. All regression procedures in Algorithm S1 are carried out using SUPERLEARNER (Van der Laan et al., 2007), which combines random forest, XGboost, Bayesian Additive Regression Trees, adaptive polynomial splines, adaptive regression splines, single-layer neural networks, linear regression, and recursive partitioning-based regression trees. We show the results of  $\hat{\tau}_{SL}(x, t)$  and  $\hat{\tau}_{XL}(x, t)$  in Figure S1. Comparing Figure ?? and Figure S1, the proposed R-learner  $\hat{\tau}(x, t)$  is the best among all comparative approaches.

#### S4. ADDITIONAL SIMULATION RESULTS FOR §??

We include the additional simulation results in Figure S2. Across all different settings, our proposed estimators present superior performance with small estimation errors, and the empirical coverage rates are closed to the nominal level 90% after undersmoothing. With larger  $n$ , our proposed estimators have smaller estimation variances, which is consistent with our theoretical results for consistency.

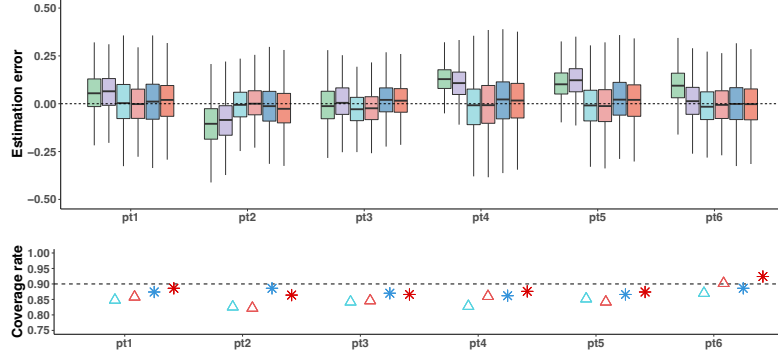(a)  $n = 2000$  and  $T$  is generated from the Beta distribution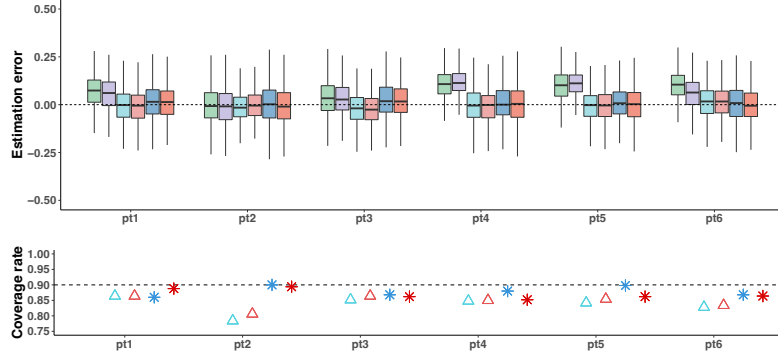(b)  $n = 4000$  and  $T$  is generated from the uniform distribution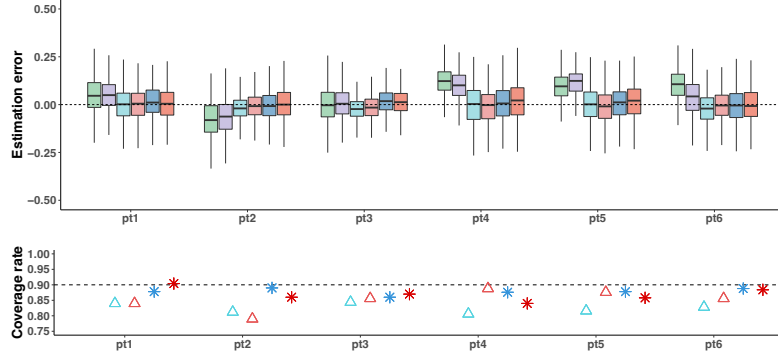(c)  $n = 4000$  and  $T$  is generated from the Beta distribution

Fig. S2: From top to bottom, different subfigures report simulation results under different settings. In each subfigure, different colors represent simulation results of different methods. The top panel shows the box-plots of pointwise errors for all comparative estimators, and the bottom panel shows the empirical coverage rates for the proposed estimators excluding S- and X-learners for which confidence intervals are not available. Different methods are labeled in different colors and/or shapes: S-learner (Green), X-learner (purple), proposed R-learner with the nuisance function estimated by Strategy (i) (light blue/triangle) or (ii) (light red/triangle) under Scenario (A) and with the nuisance function estimated by Strategy (i) (dark blue/star) or (ii) (dark red/star) under Scenario (B).

## S5. PROOFS OF PROPOSITIONS AND THEOREMS

Before delving into the main proofs, we first simplify the setting for theoretical analysis, define some shorthand notation, and state some regularization conditions in §S5.1. We briefly review some technical details of B-spline functions in §S5.2. We list useful lemmas in §S5.3 and give the proofs for our main propositions and theorems in the remaining of the section. 85

## S5.1. Preliminaries

**Simplification of the sample-splitting procedure:** Recall  $\hat{\phi}$  and  $\hat{\sigma}$  are constructed based on the double machine learning framework, with  $K$ -fold sample splitting. During the proof, we consider a simple 2-fold training scenario such that,  $\hat{\phi}$  and  $\hat{\sigma}$  are fit based on  $n$  i.i.d. samples, while the nuisance functions  $\hat{\Gamma}$ ,  $\hat{m}$  and  $\hat{\mu}$  are all trained via another independent  $n$  i.i.d. samples. In the sense of the asymptotic theoretical analysis considered in this paper, such simplification does not lose generality, and it has been popularly employed by the splitting-based estimators (Nie & Wager, 2021; Kennedy, 2020; Kennedy et al., 2020). 90

**Notation:** For simplicity, we occasionally omit some function arguments during the proof. For any function of random variable  $h(W)$ , we may use  $h$  to represent it. Similarly, we denote  $h(W_i)$  by  $h_i$ . For random variable  $W$ , we denote  $P\{\hat{f}(W)\} = \int_{w \in \mathbb{W}} \hat{f}(w) dP(w)$  as the expectation for  $W$  treating  $\hat{f}$  as a fixed function or matrix. Thus if  $\hat{f}$  is sample-based,  $P\{\hat{f}(W)\}$  is a random variable or random matrix. The constants in the form of  $C, C_1, C_2, \dots$  can change the meanings in different proofs. We also write “wpa1” as a short notation of “with probability approaching 1”. For two matrices  $A$  and  $B$ , we write  $A \succeq B$ , if  $A - B$  is positive definitive. We use  $\|A\|_2$  to represent the spectral norm of  $A$ . 100

We now introduce some basic matrix notation involved in our main proof,

$$\begin{aligned} Q_n &= E\{\Psi(X, T)\Psi^T(X, T)\}, \\ R_n &= E[\{\Psi(X, T) - \Gamma(X)\}\{\Psi(X, T) - \Gamma(X)\}^T], \\ G_n &= R_n + \rho Q_n. \end{aligned}$$

It is easy to see both  $R_n$  and  $G_n$  are positive semi-definitive matrices. Let the singular value decompositions of  $R_n$  and  $G_n$  be 105

$$\begin{aligned} R_n &= (U \ U_\perp) \begin{pmatrix} \Sigma & \\ & 0 \end{pmatrix} \begin{pmatrix} U^T \\ U_\perp^T \end{pmatrix}, \\ G_n &= (\tilde{U} \ \tilde{U}_\perp) \begin{pmatrix} \tilde{\Sigma} & \\ & \tilde{\Sigma}_\perp \end{pmatrix} \begin{pmatrix} \tilde{U}^T \\ \tilde{U}_\perp^T \end{pmatrix}, \end{aligned} \tag{S3}$$

where  $\Sigma = \text{diag}(\sigma_1, \dots, \sigma_\zeta)$  such that  $\zeta = \text{rank}(R_n)$  and  $\sigma_1 \geq \dots \geq \sigma_\zeta$ ;  $\tilde{\Sigma} = \text{diag}(\tilde{\sigma}_1, \dots, \tilde{\sigma}_\zeta)$ ,  $\tilde{\Sigma}_\perp = \text{diag}(\tilde{\sigma}_{\zeta+1}, \dots, \tilde{\sigma}_K)$  and  $\tilde{\sigma}_1 \geq \dots \geq \tilde{\sigma}_K$ . Similarly, we write the empirical versions of  $Q_n$  and  $R_n$  as,

$$\begin{aligned} \hat{Q}_n &= P_n\{\Psi(X, T)\Psi^T(X, T)\}, \\ \hat{R}_n &= P_n[\{\hat{\Psi}(X, T) - \hat{\Gamma}(X)\}\{\hat{\Psi}(X, T) - \hat{\Gamma}(X)\}^T] \end{aligned}$$

Recalling the definition of  $\hat{G}_n$ , we then have  $\hat{G}_n = \hat{R}_n + \rho \hat{Q}_n$ . We also define,

$$\begin{aligned} \bar{G}_n &= P[\{\Psi(X, T) - \hat{\Gamma}(X)\}\{\Psi(X, T) - \hat{\Gamma}(X)\}^T] + \rho Q_n \\ \bar{R}_n &= P[\{\Psi(X, T) - \hat{\Gamma}(X)\}\{\Psi(X, T) - \hat{\Gamma}(X)\}^T]. \end{aligned}$$

Finally, we write the SVD form of  $\hat{G}_n$ , 110

$$\hat{G}_n = (\hat{U} \ \hat{U}_\perp) \begin{pmatrix} \hat{\Sigma} & \\ & \hat{\Sigma}_\perp \end{pmatrix} \begin{pmatrix} \hat{U}^T \\ \hat{U}_\perp^T \end{pmatrix},$$

where  $\hat{\Sigma} = \text{diag}(\hat{\sigma}_1, \dots, \hat{\sigma}_\zeta)$ ,  $\hat{\Sigma}_\perp = \text{diag}(\hat{\sigma}_{\zeta+1}, \dots, \hat{\sigma}_K)$ , and  $\hat{\sigma}_1 \geq \dots \geq \hat{\sigma}_K$ .

**True coefficient vector  $\phi^*$ :** For our theoretical analysis, we need  $\hat{\phi}$  converging to some target vector. We choose the least squares approximation coefficients of  $\tilde{\tau}(X, T)$  as this target vector. In particular, consider the population-level least squares approximation,

$$\phi^* = \arg \min_{\phi \in \mathbb{R}^K} E[\{\tilde{\tau}(X, T) - \phi^\top \Psi(X, T)\}^2].$$

With simple algebra, one has

$$\phi^* = Q_n^{-1} E[\tilde{\tau}(X, T) \Psi(X, T)]. \quad (\text{S4})$$

For the tensor product of B-spline basis, Huang et al. (2003); Belloni et al. (2015) have shown the  $\mathcal{L}^\infty$  norm approximation power of least-square approximation  $(\phi^*)^\top \Psi(X, T)$ , when  $\tilde{\tau}(X, T)$  is in the  $p$ -smooth Hölder class. The following proposition is a direct application of Huang et al. (2003); Belloni et al. (2015)'s general results; see, e.g., the Appendix of Huang et al. (2003), and Belloni et al. (2015, Proposition 3.1 & Example 3.8).

**PROPOSITION S1.** Suppose  $\tilde{\tau} \in \Lambda(p, c, \mathbb{X} \times \mathbb{T})$  for some  $p, c > 0$ , and Assumptions S1, S4 hold. We have  $\|\tilde{\tau} - (\phi^*)^\top \Psi\|_{\mathbb{X} \times \mathbb{T}} \lesssim K^{-p/(d+1)}$ .

**Regularization conditions:** We summarize the regularity conditions for our asymptotic results as follows.

*Assumption S1.* Assume the basis  $\Psi(x, t) \in \mathbb{R}^K$  takes the tensor-product form,

$$\Psi(x, t) = \psi(t) \otimes \psi(x^{(1)}) \otimes \cdots \otimes \psi(x^{(d)}).$$

Here  $\psi(\cdot) = [\psi^{(1)}(\cdot), \dots, \psi^{(k)}(\cdot)]^\top \in \mathbb{R}^k$  is a vector of the B-spline functions for a single variable over  $[0, 1]$ ; thus  $K = k^{d+1}$ . The splines in  $\psi(\cdot)$  are of degree  $r \geq \lceil p \rceil$ . The generation intervals (see §S5.2) of  $\psi(\cdot)$  are  $I_1 = [0, s_1), I_2 = [s_1, s_2), \dots, I_m = [s_m, 1]$  with  $0 \leq s_1 \leq \dots \leq s_m \leq 1$ ,  $m \geq 2$  and  $k = r + m$ . Finally, we assume there exists a  $\kappa > 0$  not dependent on  $n$ , such that for any  $n \in \mathbb{Z}^+$ ,

$$\frac{\max_{0 \leq m_0 \leq m} (s_{m_0+1} - s_{m_0})}{\min_{0 \leq m_0 \leq m} (s_{m_0+1} - s_{m_0})} \leq \kappa. \quad (\text{S5})$$

*Assumption S2.*  $\mathbb{X} \times \mathbb{T} \subseteq \mathbb{R}^{d+1}$  is compact. Without loss of generality and for simplicity, we let  $\mathbb{X} = [0, 1]^d$  and  $\mathbb{T} = [0, 1]$ .

*Assumption S3.* For some  $0 < a_1 \leq a_2 < 1$ , one has  $n^{a_1} \lesssim K \lesssim n^{a_2}$ .

*Assumption S4.* There exists some fixed constants  $0 < c_f < C_f < +\infty$ , such that  $c_f \leq \inf_{x \in \mathbb{X}} f(x) \leq \sup_{x \in \mathbb{X}} f(x) \leq C_f$ .

*Assumption S5.* (i)  $0 < \inf_{(x,t) \in \mathbb{X} \times \mathbb{T}} \text{Var}(Y | X = x, T = t) \leq \sup_{(x,t) \in \mathbb{X} \times \mathbb{T}} \text{Var}(Y | X = x, T = t) < +\infty$ ; (ii)  $\sup_{x \in \mathbb{X}} \text{Var}(Y | X = x) < +\infty$ ; (iii)  $\sup_{x \in \mathbb{X}} |E(Y | X = x)| < +\infty$ .

*Assumption S6.* (i)  $\|\hat{m} - m\|_{\mathbb{X}} = o_P(1)$ ; (ii)  $\|\hat{\Gamma}^\top \phi^* - \Gamma^\top \phi^*\|_{\mathbb{X}} = o_P(1)$ .

For the ease of exposition, we use the same univariate B-spline function  $\psi(\cdot)$  for all variables  $X^{(1)}, \dots, X^{(d)}$  and  $T$  in Assumption S1. We note the theoretical results remain the same when dimension  $k$  and  $I_1, \dots, I_m$  vary for each variable, as long as the dimensions of all univariate B-splines are on the same asymptotic order and their mesh ratios given in (S5) are bounded by a uniform constant  $\kappa > 0$ . Overall the Assumption S1 is mild; see, e.g., Douglas et al. (1975); Huang et al. (2003). Assumption S2 is a common assumption for the sieve-type estimator (Newey, 1997; Huang et al., 2003; Belloni et al., 2015; Shi et al., 2020). Assumption S3 mildly controls the growing speed of the basis number, so that we can approximate  $\tau(X, T)$  nonparametrically. Assumption S4 is a standard condition for sieve method (Huang et al., 2003; Chen & Christensen, 2015). Assumption S5 contains some weak moment conditions; Similar assumptions are often employed in sieve estimation and causal inference literature (Chen & Christensen,

2015; Cui et al., 2020). Assumption S6 states that the nuisance functions  $\hat{m}(x)$  and  $\hat{\Gamma}^T(x)\phi^*$  are both uniformly consistent estimators for their true counterparts. Assumption S6 (i) has previously been considered by Kennedy et al. (2017) for the doubly robust average treatment effect estimation with continuous treatments. Moreover, one sufficient condition that makes Assumption S6 (ii) hold is that  $\hat{\Gamma}(x)$  is estimated by the generalized propensity score  $\hat{\omega}(t | x)$ , and  $\hat{\omega}(t | x)$  satisfies a similar uniform consistency as  $\hat{m}(x)$ ,

$$\|\hat{\omega} - \omega\|_{\mathbb{X} \times \mathbb{T}} = o_P(1). \quad (\text{S6})$$

Condition (S6) has previously been considered by Kennedy et al. (2017) as a regularization condition. Proposition S2 formalizes the justification that Condition (S6) is a sufficient condition for Assumption S6 (ii).

**PROPOSITION S2.** Suppose  $\tilde{\tau} \in \Lambda(p, c, \mathbb{X} \times \mathbb{T})$  for some  $p, c > 0$ , and Assumptions S1, S2, S4 hold. When  $\hat{\Gamma}(x) = E_{\hat{\omega}}\{\Psi(X, T) | X = x\}$ , then we have Assumption S6 (ii) holds, whenever (S6) holds.

*Proof of Proposition S2.* By Proposition S1, we have  $\|\tilde{\tau} - \{\phi^*\}^T \Psi\|_{\mathbb{X} \times \mathbb{T}} \lesssim 1$ . Also,  $\|\tilde{\tau}\|_{\mathbb{X} \times \mathbb{T}} \leq C$  for some  $C > 0$  due to  $\tilde{\tau} \in \Lambda(p, c, \mathbb{X} \times \mathbb{T})$ . We thus have

$$\begin{aligned} \|\{\phi^*\}^T \Psi\|_{\mathbb{X} \times \mathbb{T}} &\leq \|\tilde{\tau} - \{\phi^*\}^T \Psi\|_{\mathbb{X} \times \mathbb{T}} + \|\tilde{\tau}\|_{\mathbb{X} \times \mathbb{T}} \\ &\lesssim 1. \end{aligned} \quad (\text{S7})$$

On the other hand, we note that

$$\begin{aligned} \hat{\Gamma}^T(x)\phi^* - \Gamma^T(x)\phi^* &= E_{\hat{\omega}}\{\Psi^T(X, T)\phi^* | X = x\} - E_{\omega}\{\Psi^T(X, T)\phi^* | X = x\} \\ &= \int_{\mathbb{T}} \Psi^T(x, t)\phi^* \{\hat{\omega}(t | x) - \omega(t | x)\} dt. \end{aligned}$$

Thus we have

$$\begin{aligned} \|\hat{\Gamma}^T\phi^* - \Gamma^T\phi^*\|_{\mathbb{X}} &= \sup_{x \in \mathbb{X}} \left| \int_{\mathbb{T}} \Psi^T(x, t)\phi^* \{\hat{\omega}(t | x) - \omega(t | x)\} dt \right| \\ &\leq \|\hat{\omega} - \omega\|_{\mathbb{X} \times \mathbb{T}} \cdot \sup_{x \in \mathbb{X}} \int_{\mathbb{T}} |\Psi^T(x, t)\phi^*| dt \\ &\leq \|\hat{\omega} - \omega\|_{\mathbb{X} \times \mathbb{T}} \cdot \int_{\mathbb{T}} \|\{\phi^*\}^T \Psi\|_{\mathbb{X} \times \mathbb{T}} dt \\ &\lesssim o_P(1), \end{aligned}$$

by (S7), whenever (S6) holds and  $\mathbb{T}$  is compact. This completes the proof.  $\square$

### S5.2. Brief review of the B-spline functions

We give some precise descriptions of how to construct  $\Psi(x, t)$  and the corresponding theoretical properties. We construct  $\psi(w) = [\psi^{(1)}(w), \dots, \psi^{(k)}(w)]^T$  for  $w \in [0, 1]$ . Define

$$N_j^{(1)}(w) = I(w \in I_j) \quad j = 1, \dots, m.$$

For  $r \geq 2$  and  $j = -(r-1), \dots, m$ , define

$$N_j^{(r)}(w) = \frac{w - s_j}{s_{j+r-1} - s_j} N_j^{(r-1)}(w) + \frac{s_{j+r} - w}{s_{j+r} - s_{j+1}} N_{j+1}^{(r-1)}(w), \quad (\text{S8})$$

where  $s_{-(r-1)} = \dots = s_{-1} = 0$ ,  $s_{m+1} = \dots = s_{m+r} = 1$ , and take  $1/0 = 0$  as the convention. We thus have the relationship  $k = r + m$ . We define  $\psi(w)$  by normalizing  $N_j^{(r)}(w)$  as,

$$\begin{aligned} \psi(w) &= [\psi^{(1)}(w), \dots, \psi^{(k)}(w)]^T \\ &= \sqrt{k} \cdot [N_{-(r-1)}^{(r)}(w), \dots, N_m^{(r)}(w)]^T. \end{aligned} \quad (\text{S9})$$

This constitutes the univariate B-spline function. Finally, we form the multivariate B-spline functions  $\Psi(x, t)$  by the tensor product of  $\psi(t), \psi(x^{(1)}), \dots, \psi(x^{(d)})$  as

$$\Psi(x, t) = \psi(t) \otimes \psi(x^{(1)}) \otimes \dots \otimes \psi(x^{(d)});$$

here  $x^{(1)}, \dots, x^{(d)}$  correspond to the coordinate-wise random variables  $X^{(1)}, \dots, X^{(d)}$  of  $X$ .

170 The following lemmas state some standard results for the B-spline functions, which will be useful in our theoretical analysis. In particular, letting  $1_k = (1, \dots, 1)^T \in \mathbb{R}^k$ , Lemma S1 shows that  $1_k^T \psi(w)$  will be a fixed constant for any  $w \in [0, 1]$ . Lemma S2 provides explicit properties of  $N_j^{(r)}(w)$ . Lemma S3 states asymptotic properties of  $\Psi(x, t)$ .

LEMMA S1. Given any fixed  $r \in Z^+$ , for the  $\{N_j^{(r)}(w)\}_{j=1}^m$  defined in (S8), we have

$$\sum_{j=-(r-1)}^m N_j^{(r)}(w) \equiv 1$$

for any  $w \in [0, 1]$ . Furthermore, for any  $w \in [0, 1]$ ,  $1_k^T \psi(w) \equiv \sqrt{k}$ .

*Proof of Lemma S1.* When  $r = 1$ , we have

$$\sum_{j=1}^m N_j^{(1)}(w) = \sum_{j=1}^m I(w \in I_j) = I(w \in [0, 1]) \equiv 1.$$

175 When  $r \geq 2$ , by (S8), one has

$$\begin{aligned} \sum_{j=-(r-1)}^m N_j^{(r)}(w) &= \frac{w - s_{-(r-1)}}{s_0 - s_{-(r-1)}} N_{-(r-1)}^{(r-1)}(w) + \left\{ \sum_{j=-(r-1)}^{m-1} \frac{s_{j+r} - w}{s_{j+r} - s_{j+1}} N_{j+1}^{(r-1)}(w) + \frac{w - s_{j+1}}{s_{j+r} - s_{j+1}} N_{j+1}^{(r-1)}(w) \right\} \\ &\quad + \frac{s_{m+r} - w}{s_{m+r} - s_{m+1}} N_{m+1}^{(r-1)}(w) \\ &= \sum_{j=-(r-1)}^{m-1} \frac{s_{j+r} - w}{s_{j+r} - s_{j+1}} N_{j+1}^{(r-1)}(w) + \frac{w - s_{j+1}}{s_{j+r} - s_{j+1}} N_{j+1}^{(r-1)}(w) \\ &= \sum_{j=-(r-1)-1}^m N_j^{(r-1)}(w), \end{aligned} \tag{S10}$$

where the first equality follows by  $s_0 - s_{-(r-1)} = s_{m+1} - s_{m+1} = 0$  and  $1/0 = 0$ . Thus we have  $\sum_{j=-(r-1)}^m N_j^{(2)}(w) = \sum_{j=0}^m N_j^{(1)}(w) = 1$  for any  $w \in [0, 1]$ . Finally, by (S10) and mathematical induction, one has  $\sum_{j=-(r-1)}^m N_j^{(r)}(w) \equiv 1$  for all  $w \in [0, 1]$  and  $r \geq 2$ . By (S9), we conclude that for any  $w \in [0, 1]$ ,

$$(1, \dots, 1) \cdot \psi(w) = \sqrt{k} \sum_{j=-(r-1)}^m N_j^{(r)}(w) = \sqrt{k},$$

180 which completes the proof.  $\square$

LEMMA S2. Given any fixed  $r \in Z^+$ , for the  $\{N_j^{(r)}(w)\}_{j=1}^m$  defined in (S8), we have

- (i)\* For any given  $j = -(r-1), \dots, m$ , we have  $N_j^{(r)}(w) = 0$  for all  $w \notin [s_j, s_{j+r}]$ .
- (ii)\* For any given  $j = -(r-1), \dots, m$ , we have  $N_j^{(r)}(w) > 0$  for all  $w \in (s_j, s_{j+r})$ .



(iii)\* For any given  $\ell = 0, \dots, m$ , when  $w \in [s_\ell, s_{\ell+1})$ , we have

$$\sum_{j=-(r-1)}^m \tilde{\beta}_j N_j^{(r)}(w) = \sum_{j=-(r-1)+\ell}^{\ell} \tilde{\beta}_j N_j^{(r)}(w),$$

for any  $(\tilde{\beta}_{-(r-1)}, \dots, \tilde{\beta}_m)^\top \in \mathbb{R}^{m+r}$ .

(iv)\* Under Assumption S1, we have  $\sup_{\substack{j=-(r-1), \dots, m \\ w \in [0,1]}} |N_j^{(r)}(w)| = \mathcal{O}(1)$  when  $m \rightarrow +\infty$ .

185

By (S9), we then have that  $\psi(w)$  satisfies the corresponding properties:

- (i) For any given  $\tilde{k} = 1, \dots, k$ , we have  $\psi^{(\tilde{k})}(w) = 0$  for all  $w \notin [s_{\tilde{k}-r}, s_{\tilde{k}}]$ .
- (ii) For any given  $\tilde{k} = 1, \dots, k$ , we have  $\psi^{(\tilde{k})}(w) > 0$  for all  $w \in (s_{\tilde{k}-r}, s_{\tilde{k}})$ .
- (iii) For any given  $\ell = 0, \dots, m$ , when  $w \in [s_\ell, s_{\ell+1})$ , we have

$$\sum_{\tilde{k}=1}^k \beta_{\tilde{k}} \psi^{(\tilde{k})}(w) = \sum_{\tilde{k}=\ell+1}^{\ell+r} \beta_{\tilde{k}} \psi^{(\tilde{k})}(w),$$

for any  $(\beta_1, \dots, \beta_k)^\top \in \mathbb{R}^k$ .

(iv) Under Assumption S1, we have  $\sup_{\substack{\tilde{k}=1, \dots, k \\ w \in [0,1]}} |\psi^{(\tilde{k})}(w)| = \mathcal{O}(\sqrt{k})$  when  $m \rightarrow +\infty$ .

190

*Proof of Lemma S2.* The results in (i)–(iv) follow from (i)\*–(iv)\* by recalling (S9) and the relationship  $j = k - r$ . So it suffices to show (i)\*–(iv)\*. The results in (i)\*, (ii)\* and (iii)\* are adapted from (1.6), (1.7) and (1.36) in Kunoth et al. (2018), respectively, with their  $B_{j+r, r-1, \xi}(w)$  being our notation  $N_j^{(r)}(w)$  and  $\xi = (s_{-(r-1)}, \dots, s_{m+r})$ . For the B-spline functions with regularization conditions assumed in Assumption S1, the (iv) and (iv)\* are standard results; see, e.g., Newey (1997); Belloni et al. (2015).  $\square$

195

LEMMA S3. Suppose  $\Psi(x, t)$  satisfies Assumption S1. When  $n \rightarrow +\infty$ , we have

- (i) (Uniform boundedness):  $\|\Psi\|_{\mathbb{X} \times \mathbb{T}} \lesssim \sqrt{K}$ .
- (ii) (Bounded spectrums): Let  $J_{X, T} = \int_{\mathbb{X} \times \mathbb{T}} \Psi(x, t) \Psi^\top(x, t) dx dt$ . One has  $\lambda_{\min}(J_{X, T})$  and  $\lambda_{\max}(J_{X, T})$  are bounded away from both 0 and  $+\infty$ . Similar upper and lower bounds also hold for  $J_T = \int_{\mathbb{T}} \psi(t) \psi^\top(t) dt$ .
- (iii) (Belonging to  $\mathcal{L}_P^2(X, T)$  space):  $\phi^\top \Psi$  is in  $\mathcal{L}_P^2(X, T)$  for any given  $n$  and  $\phi \in \mathbb{R}^K$ .

200

*Proof of Lemma S3.* These are standard results for B-splines under Assumption S1; see, e.g., Belloni et al. (2015); Chen & Christensen (2015).  $\square$

### S5.3. Technical lemmas

In this section, we present all the technical lemmas for the proofs of our main propositions and theorems.

205

LEMMA S4. Suppose Assumptions ??, S1, S2 and S4 hold. Let  $\text{span}(U_\perp)$  be the linear subspace in  $\mathbb{R}^K$  which is spanned by the column vectors in  $U_\perp$ , and  $\text{span}(U)$  is defined correspondingly. We have the following spectral properties of  $R_n$ .

- (i) We have  $\text{span}(U_\perp) = \{u \mid u^\top \Psi(x, t) \text{ is free of } t\}$ . Specifically, if  $u \in \text{span}(U_\perp)$ , we have  $u^\top \Psi(x, t) = u^\top \Gamma(x)$  for any  $(x, t) \in \mathbb{X} \times \mathbb{T}$ .
- (ii) Let  $f_j = (1, 0_{j-1}^\top, -1, 0_{k-j-1}^\top)^\top \in \mathbb{R}^k$  for  $j = 1, \dots, k-1$ , and  $F = [f_1, \dots, f_{k-1}]$ . The  $\text{span}(U)$  and  $\text{span}(U_\perp)$  can be represented as follows:
  - a.  $\text{span}(U) = \text{span}\{v_T \otimes v\}$  where (i)  $v_T = \tilde{\beta}^\top F$ ; (ii)  $\tilde{\beta}$  and  $v$  can be any vectors in  $\mathbb{R}^{k-1}$  and  $\mathbb{R}^{K/k}$ , respectively. Here  $\text{span}\{v_T \otimes v\}$  represents the linear subspace spanned by all vectors taking the form of  $v_T \otimes v$ .

215

b.  $\text{span}(U_\perp) = \{1_k \otimes v \mid v \text{ can be any vector in } \mathbb{R}^{K/k}\}.$

With the dimensions of  $\text{span}(U)$  and  $\text{span}(U_\perp)$  being specified, we can further conclude that

$$\zeta = K - K/k.$$

(iii) When  $\varpi(t \mid x)$  is free of  $x$ , i.e.,  $T$  is completely random, one has

$$\sigma_\zeta = \sigma_{K-K/k} \gtrsim 1.$$

(iv) Suppose  $\hat{\Gamma}(x)$  is trained via the methods according to Remark ???. We have  $U_\perp\{\Gamma(x) - \hat{\Gamma}(x)\} = 0$  for any  $x \in \mathbb{X}$ .

220 *Proof of Lemma S4.* We prove the four parts of Lemma S4, respectively.

**Proof of Lemma S4 (i)** By the basic property of singular value decomposition, we have  $u \in \text{span}(U_\perp)$  if and only if  $u^\top R_n u = 0$ . Then, if  $u \in \text{span}(U_\perp)$ , one has,

$$E\left[\{u^\top \Psi(X, T) - E[u^\top \Psi(X, T) \mid X]\}^2\right] = u^\top R_n u = 0, \quad (\text{S11})$$

which is equivalent to that

$$u^\top \Psi(X, T) = E\{u^\top \Psi(X, T) \mid X\} \quad (\text{S12})$$

a.s.. This implies that,

$$u^\top \Psi(x, t) = E\{u^\top \Psi(X, T) \mid X = x\}$$

holds almost everywhere on the Lebesgue measure over  $[0, 1]^{d+1}$ , since  $f(x, t) = f(x)f(x \mid t)$  is an upper and lower bounded density function over  $\mathbb{X} \times \mathbb{T} = [0, 1]^{d+1}$ , under Assumptions ??, S2 and S4. By the continuity of the B-spline function (§S5.2), we further have that

$$u^\top \Psi(x, t) = E\{u^\top \Psi(X, T) \mid X = x\}$$

225 holds for any  $(x, t) \in [0, 1]^{d+1}$ . In addition, since  $E\{u^\top \Psi(X, T) \mid X = x\}$  does not contain  $t$ , we conclude from (S12) that  $u^\top \Psi(x, t)$  now is a function dependent only on  $x$ , over  $(x, t) \in [0, 1]^{d+1}$ .

On the other hand, suppose  $u$  satisfies that  $u^\top \Psi(x, t)$  is a function only of  $x$  over  $[0, 1]^{d+1}$ . We then have,  $E\{u^\top \Psi(X, T) \mid X = x\} = u^\top \Psi(x, t)$  and thus

$$E\left[\{u^\top \Psi(X, T) - E\{u^\top \Psi(X, T) \mid X\}\}^2\right] = E\left[\{u^\top \Psi(X, T) - u^\top \Psi(X, T)\}^2\right] = 0,$$

which implies  $u^\top R_n u = 0$  and thus  $u \in \text{span}(U_\perp)$ . Summarizing the two sides of the equivalence shown above, the result (i) is hence proved.

230 **Proof of Lemma S4 (ii)** Let  $S_{U_\perp} = \{1_k \otimes v \mid v \text{ can be any vector in } \mathbb{R}^{K/k}\}$  and  $S_U = \text{span}\{v_T \otimes v\}$  where (i)  $v_T = \tilde{\beta}^\top F$ ; (ii)  $\tilde{\beta}$  and  $v$  can be any vectors in  $\mathbb{R}^{k-1}$  and  $\mathbb{R}^{K/k}$ , respectively. It is easy to verify  $S_{U_\perp}$  and  $S_U$  are both linear subspaces in  $\mathbb{R}^K$ . Specifically, let  $1_k \otimes v_1$  and  $1_k \otimes v_2$  be two arbitrary vectors in  $S_{U_\perp}$ . We note their linear combination takes the form of

$$c_1(1_k \otimes v_1) + c_2(1_k \otimes v_2) = 1_k \otimes (c_1 v_1 + c_2 v_2),$$

235 which is also in  $S_{U_\perp}$ . Similar arguments hold for  $S_U$  as well. In addition, by checking the definition, one can also see that  $\{f_{j_1} \otimes e_{j_2}, j_1 = 1, \dots, k-1, j_2 = 1, \dots, K/k\}$  and  $\{1_k \otimes e_{j_2}, j_2 = 1, \dots, K/k\}$  form basis of  $S_U$  and  $S_{U_\perp}$ , respectively. Here  $\{e_{j_2}\}_{j_2=1}^{K/k}$  are the standard basis of  $\mathbb{R}^{K/k}$ . Therefore,  $\dim(S_U) = K - K/k$ ,  $\dim(S_{U_\perp}) = K/k$ , and  $\dim(S_U) + \dim(S_{U_\perp}) = K$ ; here  $\dim(\cdot)$  is the dimension of the corresponding linear subspace.

We first show  $S_{U_\perp} = \text{span}(U_\perp)$ . Denote  $\Psi(x) = \psi(x^{(1)}) \otimes \cdots \otimes \psi(x^{(d)})$ . By Lemma S1 and the basic property of Kronecker product multiplication (e.g., Horn & Johnson, 1991), we observe for any  $v \in \mathbb{R}^{K/k}$ ,

240

$$\begin{aligned} \{1_k \otimes v\}^\top \Psi(x, t) &= \{1_k \otimes v\}^\top \{\psi(t) \otimes \Psi(x)\} \\ &= 1_k^\top \psi(t) \cdot v^\top \Psi(x) \\ &= \sqrt{k} v^\top \Psi(x), \end{aligned}$$

which is free of  $t$ , thus  $1_k \otimes v \in \text{span}(U_\perp)$  and

$$S_{U_\perp} \subseteq \text{span}(U_\perp).$$

Since both  $S_{U_\perp}$  and  $\text{span}(U_\perp)$  are linear subspaces, to show  $S_{U_\perp} = \text{span}(U_\perp)$ , it is left to show

$$\dim(S_{U_\perp}) = K/k \geq \dim\{\text{span}(U_\perp)\}. \quad (\text{S13})$$

Now for any  $f_{j_1} \otimes e_{j_2}$  as one basis function of  $S_U$ , we have for  $j_1 = 1, \dots, k-1$ ,

$$\{f_{j_1} \otimes e_{j_2}\}^\top \Psi(x, t) = \{\psi^{(1)}(t) - \psi^{(j_1+1)}(t)\} \cdot e_{j_2}^\top \Psi(x). \quad (\text{S14})$$

The above function depends on  $t$  and thus is not in  $\text{span}(U_\perp)$  by the result in (i). This is because by Lemma S2,  $\psi^{(1)}(t) = 0$  when  $t \in (s_{j_1}, s_{j_1+1})$ , while  $\psi^{(1)}(t) > 0$  when  $t \in (s_{j_1}, s_{j_1+1})$ , and thus

$$\psi^{(1)}(t) - \psi^{(j_1+1)}(t) < 0$$

when  $t \in (s_{j_1}, s_{j_1+1})$ . On the other hand, if  $j_1 < k-1$ , we have

$$\psi^{(1)}(t) = \psi^{(j_1+1)}(t) = 0$$

when  $t \in (s_{j_1+1}, 1)$ . If  $j_1 = k-1$ , we have  $\psi^{(1)}(t) = \psi^{(j_1+1)}(t) = 0$  when  $t \in (s_1, s_m)$ ; note here  $m \geq 2$  and  $s_m \geq s_1$  under Assumption S1. Therefore for any  $j_1 = 1, \dots, k-1$ , there exists some  $a, b \in [0, 1]$  such that  $\psi^{(1)}(t=a) - \psi^{(j_1+1)}(t=a) < 0$  while  $\psi^{(1)}(t=b) - \psi^{(j_1+1)}(t=b) = 0$ , which directly implies from (S14) that  $\{f_{j_1} \otimes e_{j_2}\}^\top \Psi(x, t)$  is a function that can change with  $T$ , for any given basis function  $f_{j_1} \otimes e_{j_2}$  of  $S_U$ . By results in (i), we know all  $K - K/k$  linearly independent vectors in  $\{f_{j_1} \otimes e_{j_2} \mid j_1 = 1, \dots, k-1, j_2 = 1, \dots, K/k\}$  are not in  $\text{span}(U_\perp)$ . By the basic property of the linear space, we conclude  $\dim\{\text{span}(U_\perp)\} \leq K - (K - K/k) = \dim(S_{U_\perp})$ , which verifies (S13) and thus shows

$$S_{U_\perp} = \text{span}(U_\perp)$$

Finally, observing that for any basis function  $f_{j_1} \otimes e_{j_2}$  of  $S_U$  and any vector  $1_k \otimes v \in S_{U_\perp} = \text{span}(U_\perp)$ , we have

$$(f_{j_1} \otimes e_{j_2})^\top \cdot 1_k \otimes v = (f_{j_1}^\top \cdot 1_k) \cdot (e_{j_2}^\top \cdot v) = 0,$$

as  $f_{j_1} \cdot 1_k = 1 - 1 = 0$  by definition. We thus have

245

$$S_U \perp \text{span}(U_\perp) \quad (\text{S15})$$

and  $S_U \oplus \text{span}(U_\perp) = \mathbb{R}^K$ , since  $\dim(S_U) + \dim\{\text{span}(U_\perp)\} = K - K/k + K/k = K$ ; here  $\oplus$  denotes the direct sum of two linear spaces. With same argument, we can also show that

$$\text{span}(U) \perp \text{span}(U_\perp) \quad (\text{S16})$$

and  $\text{span}(U) \oplus \text{span}(U_\perp) = \mathbb{R}^K$ . Since the orthogonal complement of  $\text{span}(U_\perp)$  in  $\mathbb{R}^K$  is unique, by (S15)–(S16), we conclude that,

$$\text{span}(U) = S_U,$$

which completes the proof. Since  $\dim\{\text{span}(U)\} = K - \dim\{\text{span}(U_\perp)\} = K - K/k$ , we know the number of column vectors in  $U$  is  $K - K/k$ , and thus  $\zeta = K - K/k$ .

**Proof of Lemma S4 (iii)** We first present the general Weyl's inequality of matrix eigenvalue perturbation, which will be frequently used in the paper. The proof can be found in (Horn & Johnson, 1991, Theorem 3.3.16)

250

**PROPOSITION S3 (GENERAL WEYL'S INEQUALITY).** *Let  $\mathcal{R}$  be any matrix in  $\mathbb{R}^{d_1 \times d_2}$  and  $\hat{\mathcal{R}}$  be its perturbed version such that  $\hat{\mathcal{R}} = \mathcal{R} + \mathcal{E}$ . For any  $i, j$  such that  $1 \leq i, j \leq \min\{d_1, d_2\}$  and  $i + j \leq \min\{d_1, d_2\} + 1$ , we have*

255

$$\sigma_{i+j-1}(\hat{\mathcal{R}}) - \sigma_i(\mathcal{R}) \leq \sigma_j(\mathcal{E}). \quad (\text{S17})$$

Specifically, for any  $i \leq \min\{d_1, d_2\}$ ,

$$|\sigma_i(\hat{\mathcal{R}}) - \sigma_i(\mathcal{R})| \leq \|\mathcal{E}\|_2. \quad (\text{S18})$$

We now get into our main proof. Note by the law of total expectation, we have

$$Q_n = R_n + E(\Gamma\Gamma^T);$$

see (S21) in what follows. For simplicity, we denote  $\gamma = E\{\psi(T) \mid X = x\}$ . Note  $\gamma$  is free of  $x$  as  $\varpi(t \mid x)$  is free of  $x$ . We thus also write  $\varpi(t \mid x) = \varpi(t)$  for abbreviation. By the basic property of Kronecker product (Schacke, 2004), we then have

260

$$\begin{aligned} E(\Gamma\Gamma^T) &= E\left[[E\{\psi(T) \mid X\} \otimes \Psi(X)] [E\{\psi(T) \mid X\} \otimes \Psi(X)]^T\right] \\ &= E\{\gamma\gamma^T \otimes \Psi(X)\Psi^T(X)\} \\ &= \gamma\gamma^T \otimes E\{\Psi(X)\Psi^T(X)\}. \end{aligned} \quad (\text{S19})$$

Since  $\gamma\gamma^T$  is a rank-one matrix, by e.g. Horn & Johnson (1991, Theorem 4.2.12) and (S19), we have

$$\begin{aligned} \text{rank}\{E(\Gamma\Gamma^T)\} &\leq 1 \cdot \text{rank}[E\{\Psi(X)\Psi^T(X)\}] \\ &\leq K/k, \end{aligned}$$

which implies  $\sigma_{K/k+1}\{E(\Gamma\Gamma^T)\} = 0$ . Taking  $\hat{\mathcal{R}} = Q_n$ ,  $\mathcal{R} = R_n$ ,  $\mathcal{E} = E(\Gamma\Gamma^T)$ ,  $j = K/k + 1$ , and  $i = K - K/k$  in Proposition S3, we have that,

$$\begin{aligned} \sigma_{K-K/k}(R_n) &\geq \sigma_K(Q_n) - \sigma_{K/k+1}\{E(\Gamma\Gamma^T)\} \\ &= \sigma_K(Q_n) \\ &\gtrsim 1, \end{aligned}$$

where the last inequality is because the smallest singular value of  $Q_n$  is bounded away from 0; see Lemma S5.

265

**Proof of Lemma S4 (iv)** By the result in (i), we have  $U_\perp \Psi(x, t)$  is free of  $t$ . We then have

$$\begin{aligned} U_\perp\{\Gamma(x) - \hat{\Gamma}(x)\} &= E\{U_\perp \Psi(X, T) \mid X = x\} - E_{\varpi}\{U_\perp \Psi(X, T) \mid X = x\} \\ &= U_\perp \Psi(x, t) - U_\perp \Psi(x, t) \\ &= 0. \end{aligned}$$

**LEMMA S5.** *Assumptions ??, S1, S4 hold. When  $n \rightarrow +\infty$ , we have following bounds.*

- (i) *The eigenvalues of  $Q_n$  are bounded away from 0 and  $+\infty$ , and  $\|R_n\|_2, \|E(\Gamma\Gamma^T)\|_2, \|E[E\{\psi(T) \mid X\}E\{\psi^T(T) \mid X\}]\|_2 \lesssim 1$ .*
- (ii) *If  $\tilde{\tau} \in \Lambda(p, c, \mathbb{X} \times \mathbb{T})$  for some  $p, c > 0$ , we have  $\|\phi^*\| \lesssim 1$ .*

270

*Proof of Lemma S5.* We prove the two parts of Lemma S5 in order.

**Proof of Lemma S5 (i)** First we note that by the forms of  $Q_n$ ,  $R_n$ ,  $E(\Gamma\Gamma^T)$ , and  $E[E\{\psi(T) \mid X\}E\{\psi^T(T) \mid X\}]$ , it is clear to see they are all symmetric and positive semi-definitive.

Let  $v \in \mathbb{R}^K$  be any vector with  $\|v\| = 1$ . One has

$$\begin{aligned}
\lambda_{\max}(Q_n) &= \sup_{\|v\|=1} |v^\top E[\Psi(T, X)\Psi(T, X)^\top] v| \\
&= \sup_{\|v\|=1} \int_{\mathbb{X} \times \mathbb{T}} \{v^\top \Psi(x, t)\}^2 f(t | x) f(x) dx dt \\
&\leq C_f/\epsilon \cdot \sup_{\|v\|=1} \int_{\mathbb{X} \times \mathbb{T}} \{v^\top \Psi(x, t)\}^2 dx dt \quad (\text{Assumptions S1 and S4}) \\
&\lesssim 1,
\end{aligned} \tag{S20}$$

where the last inequality follows by Lemma S3. Similarly, we have  $\lambda_{\min}(Q_n) \geq c_f/\epsilon \cdot \inf_{\|v\|=1} \int_{\mathbb{X} \times \mathbb{T}} \{v^\top \Psi(x, t)\}^2 dx dt \gtrsim 1$  also by Lemma S3 and the corresponding assumptions. 275

By the property of spectral norm (e.g., Golub & Van Loan, 2013), one has

$$\begin{aligned}
\|E(\Gamma\Gamma^\top)\|_2 &= \sup_{\|u\|=1} |u^\top E(\Gamma\Gamma^\top)u| \\
&= \sup_{\|u\|=1} \left| E\left[ \left\{ E\{u^\top \Psi(X, T) | X\} \right\}^2 \right] \right| \\
&\leq \sup_{\|u\|=1} \left| E\left[ E\{u^\top \Psi(X, T)\}^2 | X \right] \right| \\
&= \sup_{\|u\|=1} \left| E\{u^\top \Psi(X, T)\}^2 \right| \\
&= \|Q_n\|_2 \lesssim 1,
\end{aligned}$$

where the first inequality follows by Cauchy-Schwarz inequality and the last inequality follows by (S20). The  $\|E[E\{\psi(T) | X\}E\{\psi^\top(T) | X\}]\|_2$  can be bounded by similar arguments. This is because  $\|E(\Gamma\Gamma^\top)\|$  is actually the same type of matrix as  $E(\Gamma\Gamma^\top)$ , which only replaces the  $\Gamma(x) = E\{\Psi(X, T) | X = x\}$  with  $E\{\psi(T) | X = x\}$ . Finally, rewrite  $R_n$  as 280

$$\begin{aligned}
R_n &= E\{(\Psi - \Gamma)\{\Psi - \Gamma\}^\top\} \\
&= Q_n - E\{\Psi(X, T)\Gamma^\top(X)\} - E\{\Gamma(X)\Psi^\top(X, T)\} + E[\Gamma\Gamma^\top] \\
&= Q_n - E[\Gamma\Gamma^\top],
\end{aligned} \tag{S21}$$

where the last equality follows by  $E\{\Psi(X, T)\Gamma^\top(X)\} = E[E\{\Psi(X, T) | X\}\Gamma^\top(X)] = E(\Gamma\Gamma^\top)$  due to the law of total expectation, and similarly  $E\{\Gamma(X)\Psi^\top(X, T)\} = E(\Gamma\Gamma^\top)$ . Summarizing the above upper bounds, one has  $\|R_n\|_2 \leq \|Q_n\|_2 + \|E(\Gamma\Gamma^\top)\|_2 \lesssim 1$ .

Proof of Lemma S5 (ii) Recalling (S4), if  $\tilde{\tau} \in \Lambda(p, c, \mathbb{X} \times \mathbb{T})$  for some  $p, c > 0$ , we have  $\|\tilde{\tau}\|_{\mathbb{X} \times \mathbb{T}} \lesssim 1$  and thus 285

$$\begin{aligned}
\|\phi^*\| &\leq \|Q_n^{-1}\|_2 \|E[\tilde{\tau}(X, T)\Psi(X, T)]\| \\
&= \|Q_n^{-1}\|_2 \sup_{\|u\|=1} |E[\tilde{\tau}(X, T)u^\top \Psi(X, T)]| \\
&\leq \|\tilde{\tau}\|_{\mathbb{X} \times \mathbb{T}} \|Q_n^{-1}\|_2 \sup_{\|u\|=1} \sqrt{E[u^\top \Psi(X, T)]^2} \\
&\lesssim 1,
\end{aligned}$$

where the second inequality follows by Cauchy-Schwarz inequality, and the last inequality follows from the lower and upper bound of  $Q_n$ 's eigenvalues. □

LEMMA S6. Suppose Assumptions S1 and S5 hold. We have  $\|m(x)\|_{\mathbb{X}}, \|\hat{m}(x)\|_{\mathbb{X}}, \|\hat{\Gamma}(x)\|_{\mathbb{X}}/\sqrt{K}, \|\Gamma(x)\|_{\mathbb{X}}/\sqrt{K}$  are all bounded away from  $+\infty$  when  $n$  grows, wpa1. 290

*Proof of Lemma S6.* By Assumption S5, we have  $\|m\|_{\mathbb{X}} = \sup_{x \in \mathbb{X}} |E(Y \mid X = x)| \lesssim 1$  as  $n \rightarrow +\infty$ . By Lemma S3 and the fact  $\|\cdot\|$  in convex,

$$\begin{aligned} \|\Gamma\|_{\mathbb{X}} &= \sup_{x \in \mathbb{X}} \|E\{\Psi(X, T) \mid X = x\}\| \\ &\leq \sup_{x \in \mathbb{X}} E\{\|\Psi(X, T)\| \mid X = x\} \\ &\leq \sup_{(x, t) \in \mathbb{X} \times \mathbb{T}} \|\Psi(x, t)\| \\ &\lesssim \sqrt{K}. \end{aligned}$$

Finally, recalling (??) and (??), by the triangle inequality we have

$$\|\hat{m}\|_{\mathbb{X}} \leq \|m\|_{\mathbb{X}} + \|\hat{m} - m\|_{\mathbb{X}} \lesssim 1 + o_P(1),$$

which implies  $\|\hat{m}\|_{\mathbb{X}} \lesssim 1$ , wpa1. Similar argument also yields  $\|\hat{\Gamma}\|_{\mathbb{X}}/\sqrt{K} \lesssim 1$  wpa1.  $\square$

LEMMA S7. Suppose Assumptions ??, S1, S4 hold, and also (??) holds. When  $n \rightarrow +\infty$ , we have  $\|\bar{G}_n - G_n\|_2 = o_P(r_\gamma^2)$ , and  $\|\bar{R}_n\|_2 \lesssim 1$  wpa1.

*Proof of Lemma S7.* First we decompose,

$$\begin{aligned} \bar{G}_n - G_n &= P\{(\hat{\Gamma} - \Psi)(\hat{\Gamma} - \Psi)^T\} + \rho Q_n - E\{(\Gamma - \Psi)(\Gamma - \Psi)^T\} - \rho Q_n \\ &= \bar{R}_n - R_n \\ &= P\{(\hat{\Gamma} - \Psi)(\hat{\Gamma} - \Psi)^T\} - P\{(\Gamma - \Psi)(\Gamma - \Psi)^T\} \\ &= P\{(\hat{\Gamma} - \Gamma)(\hat{\Gamma} - \Gamma)^T\} + P\{(\hat{\Gamma} - \Gamma)(\Gamma - \Psi)^T\} + P\{(\Gamma - \Psi)(\hat{\Gamma} - \Gamma)^T\} \\ &\quad + E\{(\Gamma - \Psi)(\Gamma - \Psi)^T\} - E\{(\Gamma - \Psi)(\Gamma - \Psi)^T\} \\ &= P\{(\hat{\Gamma} - \Gamma)(\hat{\Gamma} - \Gamma)^T\}. \end{aligned} \tag{S22}$$

Note here  $P\{(\hat{\Gamma} - \Gamma)(\Gamma - \Psi)^T\} = P\{(\Gamma - \Psi)(\hat{\Gamma} - \Gamma)^T\} = 0$  as

$$\begin{aligned} &P[\{\hat{\Gamma}(X) - \Gamma(X)\}\{\Gamma(X) - \Psi(X, T)\}^T] \\ &= P[\{\hat{\Gamma}(X) - \Gamma(X)\} \cdot E[\{\Gamma(X) - \Psi(X, T)\}^T \mid X]] \\ &= P[\{\hat{\Gamma}(X) - \Gamma(X)\}\{\Gamma(X) - \Gamma(X)\}^T] \\ &= 0, \end{aligned}$$

where the first equality follows by the law of total expectation. Thus  $\|\bar{G}_n - G_n\|_2 = \|P\{(\hat{\Gamma} - \Gamma)(\hat{\Gamma} - \Gamma)^T\}\|_2 = o_P(r_\gamma^2)$  follows from (??). In addition, by Lemma S5 and (S22), one has  $\|\bar{R}_n\|_2 \leq \|R_n\|_2 + \|\bar{G}_n - G_n\|_2 \lesssim 1 + o_P(1) \lesssim 1$  wpa1 since  $r_\gamma \lesssim 0$ .  $\square$

LEMMA S8. Suppose the general settings of Theorem ?? hold. We have

- (i)  $\|\hat{Q}_n - Q_n\|_2 = \mathcal{O}_P(\sqrt{K \log n/n})$ ,  $\|\hat{G}_n - G_n\|_2 = \mathcal{O}_P(\sqrt{K \log n/n})$ , and we also have  $\|\hat{Q}_n\|_2 \lesssim 1$  and  $\|P_n(\Gamma \Gamma^T)\|_2 \lesssim 1$ , wpa1;
- (ii)  $\|\hat{G}_n^{-1} - G_n^{-1}\|_2 = \mathcal{O}_P(\rho^{-2} \sqrt{K \log n/n})$ ;
- (iii)  $\|\hat{\Sigma}^{-1}\|_2 \lesssim \beta_n^{-1}$ ,  $\|\hat{\Sigma}_\perp^{-1}\|_2 \lesssim \rho^{-1}$ ,  $\|\hat{U}_\perp^T U\|_2 \lesssim \rho \beta_n^{-1}$ ,  $\sigma_{\min}(\tilde{U}^T U) \rightarrow 1$ ;
- (iv)  $\|\Sigma^{-1}\|_2 \lesssim \beta_n^{-1}$ ,  $\|\hat{\Sigma}^{-1}\|_2 \lesssim \beta_n^{-1}$ ,  $\|\hat{\Sigma}_\perp^{-1}\|_2 \lesssim \rho^{-1}$ , wpa1, and  $\|\hat{U}_\perp^T U\|_2 = \mathcal{O}_P(\beta_n^{-1} \sqrt{K \log n/n})$ .
- (v) Recall  $\hat{A}_n, \hat{B}_n$  in Algorithm ??, and let  $A_n = \tilde{U} \tilde{\Sigma}^{-1} \tilde{U}^T$ ,  $B_n = E[\{\Psi(X, T) - \Gamma(X)\}\{\Psi(X, T) - \Gamma(X)\}^T \{Y - \mu(X, T)\}^2]$  be their population counterparts. Further assuming the conditions in the confidence interval part of Theorem ?? hold, we have  $\|\hat{A}_n\|_2, \|\hat{B}_n\|_2, \|A_n\|_2, \|B_n\|_2$  are all constantly bounded wpa1. In addition, we have,

$$\|\hat{A}_n - A_n\|_2 = o_P(1), \quad \|\hat{B}_n - B_n\|_2 = o_P(1).$$

*Proof of Lemma S8.* During the proofs, we will frequently use several classic matrix concentration and perturbation results. For the completeness, we first present these results and then get into the main proof.

PROPOSITION S4 (RUDELSON'S MATRIX LLN (RUDELSON, 1999)). Let  $\mathcal{R}_1, \dots, \mathcal{R}_n \in \mathbb{R}^{d \times d}$  be i.i.d. random matrices with  $d \geq 2$ . Suppose  $\mathcal{R} = E(\mathcal{R}_i)$  and  $\|\mathcal{R}_i\|_2 \leq C$  a.s., for any  $i \in [n]$ , then

$$E\|P_n(\mathcal{R}) - \mathcal{R}^*\|_2 \lesssim \frac{C \log d}{n} + \sqrt{\frac{C\|\mathcal{R}\|_2 \log d}{n}}.$$

PROPOSITION S5 (WEYL'S INEQUALITY (WEYL, 1912)). Let  $\hat{\mathcal{R}}$  and  $\mathcal{R}$  be  $d \times d$  symmetric matrices. We have for any  $i \in [d]$ , 315

$$\lambda_i(\mathcal{R}) + \lambda_d(\hat{\mathcal{R}} - \mathcal{R}) \leq \lambda_i(\hat{\mathcal{R}}) \leq \lambda_i(\mathcal{R}) + \lambda_1(\hat{\mathcal{R}} - \mathcal{R}).$$

Therefore, if  $\hat{\mathcal{R}} - \mathcal{R}$  is positive semi-definitive or  $\hat{\mathcal{R}} \succeq \mathcal{R}$ , one has  $\lambda_i(\mathcal{R}) \leq \lambda_i(\hat{\mathcal{R}})$  for any  $i \in [n]$ .

PROPOSITION S6 (DAVIS-KAHAN THEOREM (DAVIS & KAHAN, 1970)). Let symmetric matrix  $\hat{\mathcal{R}} \in \mathbb{R}^{d \times d}$  be the perturbed version of a symmetric matrix  $\mathcal{R} \in \mathbb{R}^{d \times d}$  such that

$$\hat{\mathcal{R}} = \mathcal{R} + \mathcal{E}.$$

Define their singular value decompositions 320

$$\begin{aligned}\hat{\mathcal{R}} &= \hat{\mathcal{U}} \hat{\mathcal{S}} \hat{\mathcal{U}}^\top + \hat{\mathcal{U}}_\perp \hat{\mathcal{S}}_\perp \hat{\mathcal{U}}_\perp^\top, \\ \mathcal{R} &= \mathcal{U} \mathcal{S} \mathcal{U}^\top + \mathcal{U}_\perp \mathcal{S}_\perp \mathcal{U}_\perp^\top,\end{aligned}$$

where  $\hat{\mathcal{U}}$  and  $\hat{\mathcal{S}}$  correspond to the top- $r$  singular vectors and top- $r$  singular values of  $\hat{\mathcal{R}}$ , respectively; similar notation also holds for  $\mathcal{R}$ . We then have

$$\|\hat{\mathcal{U}}_\perp^\top \mathcal{U}\|_2 \leq \frac{\|\hat{\mathcal{U}}^\top \mathcal{E}\|_2}{\sigma_r(\hat{\mathcal{R}}) - \sigma_{r+1}(\mathcal{R})}.$$

Proof of Lemma S8 (i) By definition one has

$$\hat{G}_n - \bar{G}_n = \left[ P_n\{(\Psi - \hat{\Gamma})(\Psi - \hat{\Gamma})^\top\} - P\{(\Psi - \hat{\Gamma})(\Psi - \hat{\Gamma})^\top\} \right] + \rho(\hat{Q}_n - Q_n) \quad (\text{S23})$$

Recalling that by Lemma S6 and Lemma S7, we have wpa1,

$$\begin{aligned}\|\Psi - \hat{\Gamma}\|_{\mathbb{X} \times \mathbb{T}}^2 &\leq (\|\Psi\|_{\mathbb{X} \times \mathbb{T}} + \|\hat{\Gamma}\|_{\mathbb{X}})^2 \\ &\lesssim K, \\ \text{and } \|P\{(\Psi - \hat{\Gamma})(\Psi - \hat{\Gamma})^\top\}\|_2 &\lesssim 1.\end{aligned} \quad (\text{S24})$$

Now we first condition on given  $\hat{\Gamma}(\cdot)$  which satisfies (S24) as  $n \rightarrow +\infty$ . Since  $\hat{\Gamma}(\cdot)$  is trained separately, one has  $\{(\Psi_i - \hat{\Gamma}_i)(\Psi_i - \hat{\Gamma}_i)^\top\}_{i=1}^n$  are i.i.d. now random matrices and 325

$$P\left[(\Psi_i - \hat{\Gamma}_i)(\Psi_i - \hat{\Gamma}_i)^\top - P\{(\Psi - \hat{\Gamma})(\Psi - \hat{\Gamma})^\top\}\right] = 0.$$

By (S24), we also have

$$\begin{aligned}\|(\Psi_i - \hat{\Gamma}_i)(\Psi_i - \hat{\Gamma}_i)^\top\|_2 &\leq \sup_{x \in \mathbb{X}} \|\Psi(x) - \hat{\Gamma}(x)\|^2 \\ &= \|\Psi - \hat{\Gamma}\|_{\mathbb{X} \times \mathbb{T}}^2 \\ &\lesssim K.\end{aligned}$$

By taking  $\mathcal{R}_i = (\Psi_i - \hat{\Gamma}_i)(\Psi_i - \hat{\Gamma}_i)^\top$  in Proposition S4 and given  $\hat{\Gamma}(\cdot)$ , one has

$$\begin{aligned} \|P_n\{(\Psi - \hat{\Gamma})(\Psi - \hat{\Gamma})^\top\} - P\{(\Psi - \hat{\Gamma})(\Psi - \hat{\Gamma})^\top\}\|_2 &\lesssim \frac{K \log K}{n} + \sqrt{\frac{K \log K}{n}} \\ &\lesssim \sqrt{\frac{K \log n}{n}}, \end{aligned} \quad (\text{S25})$$

as  $(K \log K)/n \rightarrow 0$  under Assumption S3. Since the conditioned event (S24) happens wpa1, we can directly uncondition it and (S25) implies

$$\|P_n\{(\Psi - \hat{\Gamma})(\Psi - \hat{\Gamma})^\top\} - P\{(\Psi - \hat{\Gamma})(\Psi - \hat{\Gamma})^\top\}\|_2 = \mathcal{O}_P\left(\sqrt{\frac{K \log n}{n}}\right).$$

Similarly, we can show

$$\|\hat{Q}_n - Q_n\|_2 = \mathcal{O}_P(\sqrt{K \log n/n}).$$

Note this also implies  $\|\hat{Q}_n - Q_n\|_2 \rightarrow 0$  wpa1, since  $\sqrt{K \log n/n}$  vanishes under Assumption S3. Thus we further have

$$\|\hat{Q}_n\|_2 \leq \|Q_n\|_2 + \|\hat{Q}_n - Q_n\|_2 \lesssim \|Q_n\|_2 \lesssim 1,$$

wpa1, by Lemma S5. Similarly, we can also show  $\|P_n(\Gamma \Gamma^\top)\|_2 \lesssim 1$ .

In summary, by (S23) and the bounds derived above, one has

$$\begin{aligned} \|\hat{G}_n - \bar{G}_n\|_2 &\leq \|P_n\{(\Psi - \hat{\Gamma})(\Psi - \hat{\Gamma})^\top\} - P\{(\Psi - \hat{\Gamma})(\Psi - \hat{\Gamma})^\top\}\|_2 + \rho \|\hat{Q}_n - Q_n\|_2 \\ &= \mathcal{O}_P(\sqrt{K \log n/n}) \end{aligned}$$

whenever  $\rho \gtrsim 1$ . Finally, by the triangle inequality, one has

$$\|\hat{G}_n - G_n\|_2 \leq \|\hat{G}_n - \bar{G}_n\|_2 + \|\bar{G}_n - G_n\|_2 = \mathcal{O}_P(\sqrt{K \log n/n}), \quad (\text{S26})$$

follows from Lemma S7, whenever  $r_\gamma^2 \gtrsim \sqrt{K \log n/n}$ .

Proof of Lemma S8 (ii) We first show  $\hat{G}_n$  is invertible wpa1. By definition, we write

$$\hat{G}_n = P_n\{(\hat{\Psi} - \hat{\Gamma})(\hat{\Psi} - \hat{\Gamma})^\top\} + \rho \hat{Q}_n \succeq \rho \hat{Q}_n, \quad (\text{S27})$$

as both  $P_n\{(\hat{\Psi} - \hat{\Gamma})(\hat{\Psi} - \hat{\Gamma})^\top\}$  and  $\hat{Q}_n$  are positive semi-definitive matrices. Then (S27) and Proposition S5 imply that

$$\lambda_{\min}(\hat{G}_n) \geq \lambda_{\min}(\rho \hat{Q}_n) = \rho \lambda_{\min}(\hat{Q}_n). \quad (\text{S28})$$

Recall  $\|\hat{Q}_n - Q_n\|_2 \rightarrow 0$  wpa1. By (S18) in Proposition S3 with  $\hat{\mathcal{R}} = \hat{Q}_n$  and  $\mathcal{R} = Q_n$ , one has  $\lambda_{\min}(\hat{Q}_n) \geq \lambda_{\min}(Q_n) - \|\hat{Q}_n - Q_n\|_2 \gtrsim 1$  wpa1. Thus by  $\lambda_{\min}(\hat{Q}_n) \gtrsim 1$  and (S28) we conclude that,

$$\lambda_{\min}(\hat{G}_n) \gtrsim \rho, \quad (\text{S29})$$

wpa1, thus  $\hat{G}_n$  is invertible wpa1. On the other hand, recalling (S3), one has  $\lambda_{\min}(G_n) \geq \rho \lambda_{\min}(Q_n) \gtrsim \rho$  by Lemma S3. Now wpa1, we can decompose,

$$\hat{G}_n^{-1} - G_n^{-1} = G_n^{-1}(G_n - \hat{G}_n)\hat{G}_n^{-1}, \quad (\text{S30})$$

which combining with (S29) implies, wpa1,

$$\begin{aligned} \|\hat{G}_n^{-1} - G_n^{-1}\|_2 &\leq \|G_n^{-1}\|_2 \|G_n - \hat{G}_n\|_2 \|\hat{G}_n^{-1}\|_2 \\ &= \lambda_{\min}^{-1}(\hat{G}_n) \lambda_{\min}^{-1}(G_n) \|G_n - \hat{G}_n\|_2 \\ &\lesssim \rho^{-2} \|\hat{G}_n - G_n\|_2. \end{aligned} \quad (\text{S31})$$



Finally by (S26) and (S31), we conclude  $\|\hat{G}_n^{-1} - G_n^{-1}\|_2 = \mathcal{O}_P(\rho^{-2}\sqrt{K\log n/n})$ .

**Proof of Lemma S8 (iii)** Recall  $G_n = R_n + \rho Q_n$ . By definition, it is easy to see both  $R_n$  and  $\rho Q_n$  are positive semi-definitive matrices. Thus we have  $G_n \succeq R_n$ , and by Proposition S5,

$$\sigma_\zeta(G_n) \geq \sigma_\zeta(R_n) = \beta_n, \quad (\text{S32})$$

which implies that,

$$\|\tilde{\Sigma}^{-1}\|_2 = \sigma_\zeta^{-1}(G_n) \leq \beta_n^{-1}. \quad (\text{S33})$$

On the other hand, since  $G_n \succeq \rho Q_n$ , we have

$$\sigma_{\min}(G_n) \geq \rho \sigma_{\min}(Q_n) \gtrsim \rho, \quad (\text{S34})$$

also by Lemma S5. Therefore,  $G_n$  is invertible and  $\|\tilde{\Sigma}_\perp^{-1}\|_2 = \sigma_{\min}^{-1}(G_n) \lesssim \rho^{-1}$ . Finally, by taking  $\hat{\mathcal{R}} = G_n$ ,  $\mathcal{R}_n = R_n$ , and  $\mathcal{E} = \rho Q_n$  in Proposition S6, we have

$$\begin{aligned} \|\tilde{U}_\perp^T U\|_2 &\leq \frac{\rho \|Q_n\|_2}{\sigma_\zeta(G_n) - \sigma_{\zeta+1}(R_n)} \\ &\lesssim \rho \beta_n^{-1}, \end{aligned} \quad (\text{S35})$$

recalling that  $\|Q_n\|_2 \lesssim 1$ ,  $\sigma_\zeta(G_n) \gtrsim \beta_n$ , and  $\sigma_{\zeta+1}(R_n) = 0$  due to Lemma S4 and the fact that  $R_n$  is rank- $\zeta$ . Finally Cai & Zhang (2018, Lemma 1) implies

$$\sigma_{\min}^2(\tilde{U}^T U) = 1 - \|\tilde{U}_\perp^T U\|_2^2. \quad (\text{S36})$$

Under the settings of Theorem ??, one has  $\rho \prec \sqrt{K\log n/n} \prec \beta_n$ . Then by  $\rho \prec \beta_n$  and (S35)-(S36), we have  $\sigma_{\min}^2(\tilde{U}^T U) \rightarrow 1$  as  $n \rightarrow +\infty$ .

**Proof of Lemma S8 (iv)** Recalling definition (??), one has  $\|\Sigma^{-1}\|_2 = \sigma_\zeta^{-1} = \beta_n^{-1}$ . By taking  $\hat{\mathcal{R}} = \hat{G}_n$  and  $\mathcal{R} = G_n$  in Proposition S3, one has

$$\begin{aligned} |\hat{\sigma}_\zeta - \sigma_\zeta(G_n)| &\leq \|\hat{G}_n - G_n\|_2 \\ &= \mathcal{O}_P(\sqrt{K\log n/n}). \end{aligned} \quad (\text{S37})$$

On the other hand, recalling (S32) and (S34), we have

$$\sigma_\zeta(G_n) \gtrsim \beta_n + \rho,$$

which combining with (S37), implies

$$\hat{\sigma}_\zeta \asymp \beta_n + \rho,$$

wpa1, under the assumed condition  $\beta_n + \rho \succ \sqrt{K\log n/n}$ . This implies

$$\|\hat{\Sigma}^{-1}\|_2 = \hat{\sigma}_\zeta^{-1} \lesssim (\beta_n + \rho)^{-1} \quad (\text{S38})$$

wpa1. By (S29), we have  $\|\hat{\Sigma}_\perp^{-1}\|_2 = \lambda_{\min}^{-1}(\hat{G}_n) \lesssim \rho^{-1}$  wpa1.

By taking  $\hat{\mathcal{R}} = \hat{G}_n$  and  $\mathcal{R} = R_n$  in Proposition S6, we have

$$\begin{aligned} \|\hat{U}_\perp^T U\|_2 &\leq \frac{\|\hat{G}_n - R_n\|_2}{\lambda_\zeta(\hat{G}_n) - \lambda_{\zeta+1}(R_n)} \\ &\leq \frac{\|\hat{G}_n - G_n\|_2 + \rho \|Q_n\|_2}{\hat{\sigma}_\zeta} \\ &= \mathcal{O}_P\{(\beta_n + \rho)^{-1}(\sqrt{K\log n/n} + \rho)\}, \end{aligned}$$

360 recalling that  $\hat{\sigma}_\zeta \asymp \beta_n + \rho$ ,  $\|Q_n\|_2 \lesssim 1$ , and  $\|\hat{G}_n - G_n\|_2 = \mathcal{O}_P(\sqrt{K\log n/n})$ . The final results follow, after taking the assumed condition  $\rho \prec \sqrt{K\log n/n} \prec \beta_n$  into account.

Proof of Lemma S8 (v) First when  $\beta_n \asymp 1$ , clearly we have

$$\|A_n\|_2 \leq \|\tilde{U}\|_2^2 \|\tilde{\Sigma}^{-1}\|_2 \lesssim \beta_n^{-1} \lesssim 1, \quad (\text{S39})$$

by (S33). On the other hand, we have

$$\begin{aligned} \hat{A}_n - A_n &= (\hat{U}\hat{\Sigma}\hat{U}^\top)^{-1} - (\tilde{U}\tilde{\Sigma}\tilde{U}^\top)^{-1} \\ &= (\hat{U}\hat{\Sigma}\hat{U}^\top)^{-1}(\tilde{U}\tilde{\Sigma}\tilde{U}^\top - \hat{U}\hat{\Sigma}\hat{U}^\top)(\tilde{U}\tilde{\Sigma}\tilde{U}^\top)^{-1}, \end{aligned}$$

and thus

$$\begin{aligned} \|\hat{A}_n - A_n\|_2 &\leq \|\hat{\Sigma}^{-1}\|_2 \|\tilde{\Sigma}^{-1}\|_2 \|\tilde{U}\tilde{\Sigma}\tilde{U}^\top - \hat{U}\hat{\Sigma}\hat{U}^\top\|_2 \\ &\lesssim \|\tilde{U}\tilde{\Sigma}\tilde{U}^\top - \hat{U}\hat{\Sigma}\hat{U}^\top\|_2, \end{aligned}$$

365 by (S33) and (S38). In addition, one has

$$\begin{aligned} \|\tilde{U}\tilde{\Sigma}\tilde{U}^\top - \hat{U}\hat{\Sigma}\hat{U}^\top\|_2 &\leq 2\|\hat{G}_n - G_n + \tilde{U}_\perp \tilde{\Sigma}_\perp \tilde{U}_\perp^\top\|_2 \\ &\leq 2\|\hat{G}_n - G_n\|_2 + 2\|\tilde{U}_\perp \tilde{\Sigma}_\perp \tilde{U}_\perp^\top\|_2 \\ &= \mathcal{O}_P(\sqrt{K \log n/n} + \rho) \\ &= o_P(1), \end{aligned} \quad (\text{S40})$$

where the last two equalities are by the previous derived bounds, and the conditions that  $K \lesssim n^{a_2}$  and  $\rho \rightarrow 0$  for some  $a_2 < 1$ . The first inequality of (S40) follows by that  $\hat{G}_n$  can be seen as a perturbed version of  $\tilde{U}\tilde{\Sigma}\tilde{U}^\top$  such that

$$\hat{G}_n = \tilde{U}\tilde{\Sigma}\tilde{U}^\top + (\hat{G}_n - G_n + \tilde{U}_\perp \tilde{\Sigma}_\perp \tilde{U}_\perp^\top).$$

Thus as the best rank- $\zeta$  approximation of  $\hat{G}_n$ , the  $\tilde{U}\tilde{\Sigma}\tilde{U}^\top$  satisfies the first inequality of (S40) by Eckart–  
370 Young–Mirsky theorem (Eckart & Young, 1936) such that,

$$\begin{aligned} \|\hat{G}_n - \tilde{U}\tilde{\Sigma}\tilde{U}^\top\|_2 &\leq \|\hat{G}_n - \tilde{U}\tilde{\Sigma}\tilde{U}^\top\|_2 \\ &= \|\hat{G}_n - G_n + \tilde{U}_\perp \tilde{\Sigma}_\perp \tilde{U}_\perp^\top\|_2, \end{aligned}$$

and thus  $\|\tilde{U}\tilde{\Sigma}\tilde{U}^\top - \hat{U}\hat{\Sigma}\hat{U}^\top\|_2 \leq \|\tilde{U}\tilde{\Sigma}\tilde{U}^\top - \hat{G}_n\|_2 + \|\hat{G}_n - \hat{U}\hat{\Sigma}\hat{U}^\top\|_2 \leq 2\|\hat{G}_n - G_n + \tilde{U}_\perp \tilde{\Sigma}_\perp \tilde{U}_\perp^\top\|_2$ .  
Summarizing the results above we have

$$\|\hat{A}_n - A_n\|_2 = o_P(1),$$

and thus by (S39),  $\|\hat{A}_n\|_2 \leq \|A_n\|_2 + \|\hat{A}_n - A_n\|_2 \lesssim 1$  wpa1.

We note  $\|\mu\|_{\mathbb{X} \times \mathbb{T}} < +\infty$  under Assumption S5 (iii). By the new condition that

$$\|\hat{\mu} - \mu\|_{\mathbb{X} \times \mathbb{T}} = o_P(1), \quad (\text{S41})$$

we have wpa1,

$$\begin{aligned} \|\hat{\mu}\|_{\mathbb{X} \times \mathbb{T}} &\leq \|\mu\|_{\mathbb{X} \times \mathbb{T}} + \|\hat{\mu} - \mu\|_{\mathbb{X} \times \mathbb{T}} \\ &\lesssim 1. \end{aligned} \quad (\text{S42})$$

Under our simplified two-fold training setting such that one fold trains nuisance functions and one fold trains the proposed estimator and  $\hat{\sigma}$ , we can write  $\hat{B}_n$  as

$$\hat{B}_n = \frac{1}{n} \sum_{i=1}^n \{Y_i - \hat{\mu}(X_i, T_i)\}^2 \{\Psi(X_i, T_i) - \hat{\Gamma}(X_i)\} \{\Psi(X_i, T_i) - \hat{\Gamma}(X_i)\}^\top.$$

We also define

$$\bar{B}_n = P \left[ \{Y - \hat{\mu}(X, T)\}^2 \{\Psi(X, T) - \hat{\Gamma}(X)\} \{\Psi(X, T) - \hat{\Gamma}(X)\}^\top \right].$$

Similar to (S24) and (S25), we show the convergence of  $\hat{B}_n$  by matrix concentration. It is easy to see  $P(\hat{B}_n) = \bar{B}_n$ , with  $\hat{\Gamma}(X)$  trained separately. Based on Assumption S5, Lemma S7 and (S41), we have, wpa1,

$$\begin{aligned}
\|\bar{B}_n\|_2 &= \sup_{\|\ell\|=1} P\left[\{Y - \hat{\mu}(X, T)\}^2 [\ell^\top \{\Psi(X, T) - \hat{\Gamma}(X)\}]^2\right] \\
&\leq \sup_{\|\ell\|=1} P\left[2\{Y - \mu(X, T)\}^2 + 2\{\mu(X, T) - \hat{\mu}(X, T)\}^2 [\ell^\top \{\Psi(X, T) - \hat{\Gamma}(X)\}]^2\right] \\
&= \sup_{\|\ell\|=1} P\left[2\text{Var}(Y \mid X, T) + 2\{\mu(X, T) - \hat{\mu}(X, T)\}^2 [\ell^\top \{\Psi(X, T) - \hat{\Gamma}(X)\}]^2\right] \\
&\leq \left\{ \sup_{(x,t) \in \mathbb{X} \times \mathbb{T}} 2\text{Var}(Y \mid X = x, T = t) + 2\|\hat{\mu} - \mu\|_{\mathbb{X} \times \mathbb{T}} \right\} \sup_{\|\ell\|=1} P\left[[\ell^\top \{\Psi(X, T) - \hat{\Gamma}(X)\}]^2\right] \\
&\lesssim \sup_{\|\ell\|=1} P\left[[\ell^\top \{\Psi(X, T) - \hat{\Gamma}(X)\}]^2\right] \\
&= \|P\{(\Psi - \hat{\Gamma})(\Psi - \hat{\Gamma})^\top\}\|_2 \\
&\lesssim 1,
\end{aligned}$$

where the last inequality follows by (S24). By Proposition S4, one has

$$\|\hat{B}_n - \bar{B}_n\|_2 = \mathcal{O}_P\left(\sqrt{\frac{K \log n}{n}}\right) = o_P(1).$$

In addition, we have

$$\begin{aligned}
\bar{B}_n - B_n &= P\left[\{Y - \hat{\mu}(X, T)\}^2 - \{Y - \mu(X, T)\}^2\} \{\Psi(X, T) - \hat{\Gamma}(X)\} \{\Psi(X, T) - \hat{\Gamma}(X)\}^\top\right] \\
&\quad + P\left[\{Y - \mu(X, T)\}^2 \{\Psi(X, T) - \Gamma(X)\} \{\Gamma(X) - \hat{\Gamma}(X)\}^\top\right] \\
&\quad + P\left[\{Y - \mu(X, T)\}^2 \{\Gamma(X) - \hat{\Gamma}(X)\} \{\Psi(X, T) - \hat{\Gamma}(X)\}^\top\right] \\
&= \Delta_{B,1} + \Delta_{B,2} + \Delta_{B,3}.
\end{aligned}$$

We bound the spectral norms of three terms on the right-hand side of above display, respectively. We have

$$\Delta_{B,1} = P\left[\{2Y - \hat{\mu}(X, T) - \mu(X, T)\} \{\mu(X, T) - \hat{\mu}(X, T)\} \{\Psi(X, T) - \hat{\Gamma}(X)\} \{\Psi(X, T) - \hat{\Gamma}(X)\}^\top\right],$$

and thus wpa1,

$$\begin{aligned}
\|\Delta_{B,1}\|_2 &= \sup_{\|\ell\|=1} P\left[\{2Y - \hat{\mu}(X, T) - \mu(X, T)\} \{\mu(X, T) - \hat{\mu}(X, T)\} [\ell^\top \{\Psi(X, T) - \hat{\Gamma}(X)\}]^2\right] \\
&= \sup_{\|\ell\|=1} P\left[\{2E(Y \mid X, T) - \hat{\mu}(X, T) - \mu(X, T)\} \{\mu(X, T) - \hat{\mu}(X, T)\} [\ell^\top \{\Psi(X, T) - \hat{\Gamma}(X)\}]^2\right] \\
&\leq \left\{ \|\mu\|_{\mathbb{X} \times \mathbb{T}} + \|\hat{\mu}\|_{\mathbb{X} \times \mathbb{T}} \right\} \|\mu - \hat{\mu}\|_{\mathbb{X} \times \mathbb{T}} \cdot \sup_{\|\ell\|=1} P\left[[\ell^\top \{\Psi(X, T) - \hat{\Gamma}(X)\}]^2\right] \\
&= o_P(1),
\end{aligned}$$

where the last inequality follows by the moment conditions in Assumption S5, (S42),  $\|\mu - \hat{\mu}\|_{\mathbb{X} \times \mathbb{T}} = o_P(1)$ , and (S24). With similar arguments, we can further show

$$\begin{aligned}
\|\Delta_{B,2}\|_2 &= \sup_{\|\ell\|=1} \left| P \left[ \{Y - \mu(X, T)\}^2 [\ell^\top \{\Psi(X, T) - \Gamma(X)\}] [\ell^\top \{\Gamma(X) - \hat{\Gamma}(X)\}] \right] \right| \\
&\leq \sup_{\|\ell\|=1} P \left[ \{Y - \mu(X, T)\}^2 \left| [\ell^\top \{\Psi(X, T) - \Gamma(X)\}] [\ell^\top \{\Gamma(X) - \hat{\Gamma}(X)\}] \right| \right] \\
&\leq \sup_{(x,t) \in \mathbb{X} \times \mathbb{T}} \text{Var}(Y \mid X = x, T = t) \sup_{\|\ell_1\|=1} P \left[ \ell_1^\top \{\Psi(X, T) - \Gamma(X)\} \right]^2 \sup_{\|\ell_2\|=1} P \left[ \ell_2^\top \{\Gamma(X) - \hat{\Gamma}(X)\} \right]^2 \\
&\leq \sup_{(x,t) \in \mathbb{X} \times \mathbb{T}} \text{Var}(Y \mid X = x, T = t) \|R_n\|_2 \|P[\{\Gamma(X) - \hat{\Gamma}(X)\} \{\Gamma(X) - \hat{\Gamma}(X)\}^\top]\|_2 \\
&= o_P(1),
\end{aligned}$$

where the second inequality follows by Cauchy–Schwarz inequality, and the last equality follows by (??). Similarly, we can also show  $\|\Delta_{B,3}\|_2 = o_P(1)$  and  $\|B_n\|_2 \lesssim 1$ . Summarizing all results above, we conclude wpa1,

$$\begin{aligned}
\|\hat{B}_n - B_n\|_2 &\leq \|\hat{B}_n - \bar{B}_n\|_2 + \|\Delta_{B,1}\|_2 + \|\Delta_{B,2}\|_2 + \|\Delta_{B,3}\|_2 \\
&= o_P(1),
\end{aligned}$$

and furthermore  $\|\hat{B}_n\|_2 \leq \|B_n\|_2 + \|\hat{B}_n - B_n\|_2 \lesssim 1$  wpa1.  $\square$

LEMMA S9. Suppose the general settings of Theorem ?? hold. Define  $\Delta_{1,1}$ – $\Delta_{1,5}$  in (S91) through (S92).

- (i) Suppose  $\ell_n \in \mathbb{R}^K$  is a vector that can depend on  $\{(X_i, T_i)\}_{i=1}^n$  when  $n$  grows, and  $\|\ell_n\| = 1$  for any  $n > 0$ . We have  $\|\Delta_{1,1}\| = \mathcal{O}_P(\sqrt{K/n})$  and  $|\ell_n^\top \Delta_{1,1}| = \mathcal{O}_P(1/\sqrt{n})$ ;
- 395 (ii) Suppose  $\ell_n \in \mathbb{R}^K$  is a vector that depends only on  $n$ , and  $\|\ell_n\| = 1$  for any  $n > 0$ . We have  $\|\Delta_{1,2}\| = \mathcal{O}_P(K^{-p/(d+1)})$  and  $|\ell_n^\top \Delta_{1,2}| = \mathcal{O}_P(K^{-p/(d+1)})$ ;
- (iii) Suppose  $\ell_n \in \mathbb{R}^K$  is a vector that depends only on  $n$ , and  $\|\ell_n\| = 1$  for any  $n > 0$ . We have  $\|\Delta_{1,3}\| = \mathcal{O}_P(r'_\gamma \sqrt{K/n})$  and  $|\ell_n^\top \Delta_{1,3}| = \mathcal{O}_P(r_\gamma / \sqrt{n})$ ;
- (iv) Suppose  $\ell_n \in \mathbb{R}^K$  is a vector that depends only on  $n$ , and  $\|\ell_n\| = 1$  for any  $n > 0$ . We have  $\|\Delta_{1,4}\| = \mathcal{O}_P(r_m \sqrt{K/n} + r_\gamma \sqrt{K/n})$  and  $|\ell_n^\top \Delta_{1,4}| = \mathcal{O}_P(1/\sqrt{n})$ ;
- 400 (v) Suppose  $\ell_n \in \mathbb{R}^K$  is a vector that depends only on  $n$ , and  $\|\ell_n\| = 1$  for any  $n > 0$ . We have  $\|\Delta_{1,5}\| = \mathcal{O}_P(r_m r_\gamma + r_\gamma^2 + r'_\gamma r_m \sqrt{K/n} + r'_\gamma r_\gamma \sqrt{K/n})$  and  $|\ell_n^\top \Delta_{1,5}| = \mathcal{O}_P(r_\gamma / \sqrt{n} + r_m r_\gamma + r_\gamma^2)$ .

*Proof of Lemma S9.* We first present the following concentration result which will be repeatedly used during the proof. This proposition can be simply proved by high-order Markov inequality.

PROPOSITION S7. Given  $n$ , let  $v_1, \dots, v_n$  are i.i.d. copies of random vector  $v \in \mathbb{R}^d$ . Suppose  $E(\|v\|^2) \leq A_n$ , where  $A_n > 0$  is allowed to diverge. We have for any  $J > 0$ ,

$$pr\left\{\|P_n(v) - E(v)\| > J\sqrt{d/n}\right\} \leq \frac{4A_n}{J^2 d}.$$

*Proof of Proposition S7.* By the second-order Markov's inequality, we have for any  $J > 0$ ,

$$pr\left\{\|P_n(v) - E(v)\| > J\sqrt{d/n}\right\} \leq \frac{n}{J^2 d} E\{\|P_n(v) - E(v)\|^2\}. \quad (\text{S43})$$

Now we bound  $E\{\|P_n(v) - E(v)\|^2\}$ . We can write

$$\begin{aligned}
E\{\|P_n(v) - E(v)\|^2\} &= E\left[\left\|\frac{1}{n} \sum_{i=1}^n \{v_i - E(v)\}\right\|^2\right] \\
&= \frac{1}{n^2} E\left[\left\|\sum_{i=1}^n \{v_i - E(v)\}\right\|^2\right] \\
&= \frac{1}{n} E\{\|v_i - E(v)\|^2\} \\
&\leq \frac{2}{n} E(\|v\|^2) + \|E(v)\|^2 \\
&\leq \frac{4}{n} E(\|v\|^2) \\
&\leq \frac{4A_n}{n}.
\end{aligned} \tag{S44}$$

The third equality in the above display follows because

$$\begin{aligned}
\frac{1}{n^2} E\left[\left\|\sum_{i=1}^n \{v_i - E(v)\}\right\|^2\right] &= \sum_{k=1}^d \frac{1}{n^2} E\left[\sum_{i=1}^n \{v_i^{(k)} - E(v^{(k)})\}\right]^2 \\
&= \sum_{k=1}^d \frac{1}{n^2} \text{Var}\left(\sum_{i=1}^n v_i^{(k)}\right) \\
&= \sum_{k=1}^d \frac{1}{n} \text{Var}(v^{(k)}) \\
&= \frac{1}{n} E\{\|v_i - E(v)\|^2\},
\end{aligned}$$

where we define  $v_i^{(k)}, v^{(k)}$  as the  $k$ th coordinates of  $v_i, v$ , respectively; the second equality follows by  $E(\sum_{i=1}^n v_i^{(k)}) = nE(v^{(k)})$ ; the third equality follows by  $v_1^{(k)}, \dots, v_n^{(k)}$  are independent and identically distributed. Combining (S43) and (S44) yields the desired result.  $\square$

Given  $n$  samples, during the following proof we will frequently condition on the following event  $\mathcal{E}_n$ : the nuisance functions  $(\hat{m}, \hat{\Gamma})$  are already obtained from the separate data set for nuisance function training (see §S5.1), and  $(\hat{m}, \hat{\Gamma})$  satisfies the following conditions:

- $\|\hat{m}\|_{\mathbb{X}}$  and  $\|\hat{\Gamma}\|_{\mathbb{X}}/\sqrt{K}$  are bounded by some fixed constant  $C > 0$ ;
- All of the following quantities: (i)  $r_{\gamma}^{-1} \|\hat{\Gamma} - \Gamma\|_{\mathbb{X}}/\sqrt{K}$ ; (ii)  $r_m^{-1} \|\hat{m} - m\|_{\mathcal{L}_P^2}$ ; (iii)  $r_{\gamma}^{-1} \|P[\{\hat{\Gamma}(X) - \Gamma(X)\}\{\hat{\Gamma}(X) - \Gamma(X)\}^T]\|_2^{1/2}$ ; (iv)  $\|\hat{m} - m\|_{\mathbb{X}}$ ; (v)  $\|\hat{\Gamma}^T \phi^* - \Gamma^T \phi^*\|_{\mathbb{X}}$  are bounded by  $e_n$ , where  $e_n$  is a sequence vanishing to zero, when  $n \rightarrow +\infty$ .  $\square$

By Lemma S6, Assumption S6, and rates (??)–(??), we can choose some fixed  $C_1 > 0$  and a deterministic positive sequence  $e_n \rightarrow 0$ , such that  $\mathcal{E}_n$  happens wpa1 when  $n \rightarrow +\infty$ . For simplicity, during the following proof, we use  $\text{pr}_n(\cdot)$  to represent the probability that condition on  $\mathcal{E}_n$ . Note that since nuisance functions are trained separately from the samples involved in this proof, the expectation in this proof conditional on obtained nuisance functions can be simply represented by  $P(\cdot)$ .

Now we prove (i)–(iv) sequentially.

Proof of Lemma S9 (i) For simplicity, let  $m_{i,1} = \{Y_i - \mu(T_i, X_i)\} \{\Psi(T_i, X_i) - \Gamma(X_i)\}$ . Thus  $\Delta_{1,1} = P_n(m_{i,1})$ . We have

$$\begin{aligned} E(m_{i,1}) &= E[\{Y - \mu(X, T)\} \{\Psi(X, T) - \Gamma(X)\}] \\ &= E[\{E(Y | X, T) - \mu(X, T)\} \{\Psi(X, T) - \Gamma(X)\}] \\ &= 0, \end{aligned} \tag{S45}$$

where the second equality follows by the law of total expectation. On the other hand,

$$\begin{aligned} E(\|m_{i,1}\|^2) &= E[\{Y - \mu(X, T)\}^2 \|\Psi(X, T) - \Gamma(X)\|^2] \\ &= E\{\text{Var}(Y | X, T) \|\Psi(X, T) - \Gamma(X)\|^2\} \\ &\leq \sup_{(x,t) \in \mathbb{X} \times \mathbb{T}} \text{Var}(Y | X = x, T = t) \cdot E\{\|\Psi(X, T) - \Gamma(X)\|^2\}. \end{aligned}$$

Under Assumption S5, one has  $\sup_{(x,t) \in \mathbb{X} \times \mathbb{T}} \text{Var}(Y | X = x, T = t) \lesssim 1$ . On the other hand,

$$E\{\|\Psi(X, T) - \Gamma(X)\|^2\} \leq 2\|\Psi\|_{\mathbb{X} \times \mathbb{T}}^2 + 2\|\Gamma\|_{\mathbb{X}}^2 \lesssim K$$

430 by Lemma S6. Thus  $E(\|m_{i,1}\|^2) \lesssim K$ . Let  $v_i = m_{i,1}$  in Claim S7. With results above, we have for any fixed  $J = J_0 > 0$

$$\begin{aligned} \text{pr}(\|\Delta_{1,1}\| > J_0 \sqrt{K/n}) &= \text{pr}(\|P_n(m_{i,1})\| > J_0 \sqrt{K/n}) \\ &\leq \frac{C_1 K}{J_0^2 K} = \frac{C_1}{J_0^2} \end{aligned}$$

where  $C_1$  is some fixed constant independent with  $n$  and  $J_0$ . Therefore, when  $J_0$  is sufficiently large, the right-hand side of the above display can be arbitrarily small, and thus  $\|\Delta_{1,1}\| = \mathcal{O}_P(\sqrt{K/n})$ .

Now we bound  $|\ell_n^\top \Delta_{1,1}|$ . We first condition on  $\{(X_i, T_i)\}_{i=1}^n$ . We note that given  $\{(X_i, T_i)\}_{i=1}^n$ ,  $\{\ell_n^\top m_{i,1}\}_{i=1}^n$  are independent random variables since  $\{Y_i\}_{i=1}^n$  are independent and  $\ell_n$  depends only on  $n$  and  $\{(X_i, T_i)\}_{i=1}^n$ . Furthermore, they are mean-zero, 435

$$\begin{aligned} E[\ell_n^\top m_{i,1} | \{(X_i, T_i)\}_{i=1}^n] &= E(\tilde{\ell}_n^\top m_{i,1} | X_i, T_i) \\ &= \{E(Y | X_i, T_i) - \mu(X_i, T_i)\} \{\tilde{\ell}_n^\top \Psi(X_i, T_i) - \tilde{\ell}_n^\top \Gamma(X_i)\} \\ &= 0. \end{aligned}$$

Here we use  $\tilde{\ell}_n$  to denote  $\ell_n$  given specific  $\{(X_i, T_i)\}_{i=1}^n$ . Then the conditional variance for each  $\ell_n^\top m_{i,n}$  is

$$\begin{aligned} \text{Var}[\ell_n^\top m_{i,n} | \{(X_i, T_i)\}_{i=1}^n] &= E\{(\tilde{\ell}_n^\top m_{i,n})^2 | X_i, T_i\} \\ &= E[\{Y_i - \mu(T_i, X_i)\}^2 \{\tilde{\ell}_n^\top \Psi(T_i, X_i) - \tilde{\ell}_n^\top \Gamma(X_i)\}^2 | X_i, T_i] \\ &\leq \text{Var}(Y | X_i, T_i) \cdot \{\tilde{\ell}_n^\top \Psi(T_i, X_i) - \tilde{\ell}_n^\top \Gamma(X_i)\}^2 \\ &\leq [2\{\tilde{\ell}_n^\top \Psi(T_i, X_i)\}^2 + 2\{\tilde{\ell}_n^\top \Gamma(X_i)\}^2] \sup_{(x,t) \in \mathbb{X} \times \mathbb{T}} \text{Var}(Y | X = x, T = t) \\ &\leq C_2 [\{\tilde{\ell}_n^\top \Psi(T_i, X_i)\}^2 + \{\tilde{\ell}_n^\top \Gamma(X_i)\}^2] \quad (\text{Assumption S5}) \end{aligned}$$

for some fixed  $C_2$  independent of  $n$  and  $\{(X_i, T_i)\}_{i=1}^n$ . Therefore, given  $\{(X_i, T_i)\}_{i=1}^n$ , we have that  $P_n(\ell_n^T m_{i,n})$  is mean zero and has variance,

440

$$\begin{aligned} \text{Var}\left[P_n(\ell_n^T m_{i,n}) \mid \{(X_i, T_i)\}_{i=1}^n\right] &= \text{Var}\left[\frac{1}{n} \sum_{i=1}^n \ell_n^T m_{i,n} \mid \{(X_i, T_i)\}_{i=1}^n\right] \\ &= \frac{1}{n^2} \sum_{i=1}^n \text{Var}\left[\ell_n^T m_{i,n} \mid \{(X_i, T_i)\}_{i=1}^n\right] \\ &\leq \frac{C_2}{n} \cdot \frac{1}{n} \sum_{i=1}^n \left[\{\tilde{\ell}_n^T \Psi(T_i, X_i)\}^2 + \{\tilde{\ell}_n^T \Gamma(X_i)\}^2\right]. \end{aligned}$$

By Chebyshev's inequality, given any  $\{(X_i, T_i)\}_{i=1}^n$ ,

$$|P_n(\ell_n^T m_{i,n})| = \mathcal{O}_P\left[n^{-1/2} \sqrt{\frac{1}{n} \sum_{i=1}^n \left[\{\tilde{\ell}_n^T \Psi(T_i, X_i)\}^2 + \{\tilde{\ell}_n^T \Gamma(X_i)\}^2\right]}\right] \quad (\text{S46})$$

Now we do not condition on specific  $\{(X_i, T_i)\}_{i=1}^n$ , and consider the following positive random variable, which has a constant upper bound wpa1,

$$\begin{aligned} \xi_1 &= \sqrt{\frac{1}{n} \sum_{i=1}^n \left[\{\ell_n^T \Psi(T_i, X_i)\}^2 + \{\ell_n^T \Gamma(X_i)\}^2\right]} \\ &= \sqrt{P_n\left[\{\ell_n^T \Psi(T, X)\}^2\right] + P_n\left[\{\ell_n^T \Gamma(X)\}^2\right]} \\ &\leq \sqrt{\sup_{\|\ell\|=1} P_n\left[\{\ell^T \Psi(T, X)\}^2\right] + \sup_{\|\ell'\|=1} P_n\left[\{\ell'^T \Gamma(X)\}^2\right]} \\ &= \sqrt{\|\hat{Q}_n\|_2 + \|P_n(\Gamma \Gamma^T)\|_2} \\ &\lesssim 1, \end{aligned} \quad (\text{S47})$$

where the last equality follows by Lemma S8. Combining (S46) and (S47), we directly uncondition the given  $\{(X_i, T_i)\}_{i=1}^n$ , and conclude  $|P_n(\ell_n^T m_{i,n})| = \mathcal{O}_P(1/\sqrt{n})$ .

**Proof of Lemma S9 (ii)** First, by definition, we observe

$$\begin{aligned} &\tau(X, T) - E\{\tau(X, T) \mid X\} - \{\Psi(X, T) - \Gamma(X)\}^T \phi^* \\ &= \tau(X, T) - E\{\tau(X, T) \mid X\} - E[\tau(X, T) - E\{\tau(X, T) \mid X\} \mid X] - \{\Psi(X, T) - \Gamma(X)\}^T \phi^* \\ &= \tilde{\tau}(X, T) - E\{\tilde{\tau}(X, T) \mid X\} - \{\Psi(X, T) - \Gamma(X)\}^T \phi^*. \end{aligned}$$

We now let

$$\begin{aligned} m_{i,2} &= [\tilde{\tau}(X_i, T_i) - E\{\tilde{\tau}(X, T) \mid X_i\} - \{\Psi(X_i, T_i) - \Gamma(X_i)\}^T \phi^*] \{\Psi(X_i, T_i) - \Gamma(X_i)\} \\ &= [\tau(X_i, T_i) - E\{\tau(X, T) \mid X_i\} - \{\Psi(X_i, T_i) - \Gamma(X_i)\}^T \phi^*] \{\Psi(X_i, T_i) - \Gamma(X_i)\}; \end{aligned}$$

thus  $\Delta_{1,2} = P_n(m_{i,2})$ . We then have

$$\begin{aligned}
E(m_{i,2}) &= E\left[\tilde{\tau}(X, T) - E\{\tilde{\tau}(X, T) \mid X\} - \{\Psi(X, T) - \Gamma(X)\}^\top \phi^* \mid \Psi(X, T)\right] \\
&\quad - E\left[\tilde{\tau}(X, T) - E\{\tilde{\tau}(X, T) \mid X\} - \{\Psi(X, T) - \Gamma(X)\}^\top \phi^* \mid \Gamma(X)\right] \\
&= E\left[\tilde{\tau}(X, T) - E\{\tilde{\tau}(X, T) \mid X\} - \{\Psi(X, T) - \Gamma(X)\}^\top \phi^* \mid \Psi(X, T)\right] \\
&\quad - E\left[\underbrace{\tilde{\tau}(X, T) - E\{\tilde{\tau}(X, T) \mid X\} - \{\Psi(X, T) - \Gamma(X)\}^\top \phi^*}_{=0} \mid \Gamma(X)\right] \\
&= E\left[E\{\Gamma^\top(X)\phi^* - \tilde{\tau}(X, T) \mid X\} \Psi(X, T)\right],
\end{aligned} \tag{S48}$$

by the law of total expectation. Therefore, by Lemma S5 and Proposition S1, we have

450

$$\begin{aligned}
\|E(\Delta_{1,2})\| &= \|E(m_{i,2})\| \\
&= \sup_{\|\ell\|=1} \left| E\left[E\{\Gamma^\top(X)\phi^* - \tilde{\tau}(X, T) \mid X\} \ell^\top \Psi(X, T)\right] \right| \\
&\leq \sqrt{E\left[E\{\Gamma^\top(X)\phi^* - \tilde{\tau}(X, T) \mid X\}^2\right]} \sup_{\|\ell\|=1} \sqrt{E\left[\ell^\top \Psi(X, T)\right]^2} \quad (\text{Cauchy-Schwarz inequality}) \\
&= \sqrt{E\left[E\{\Psi^\top(X, T)\phi^* - \tilde{\tau}(X, T) \mid X\}^2\right]} \|Q_n\|_2^{1/2} \\
&\leq \sup_{x \in \mathbb{X}} \left| E\{\Psi^\top(X, T)\phi^* - \tilde{\tau}(X, T) \mid X = x\} \right| \|Q_n\|_2^{1/2} \\
&\leq \sup_{x \in \mathbb{X}} \left| E\{\Psi^\top(X, T)\phi^* - \tilde{\tau}(X, T) \mid X = x\} \right| \|Q_n\|_2^{1/2} \\
&\leq \|\tilde{\tau} - \{\phi^*\}^\top \Psi\|_{\mathbb{X} \times \mathbb{T}} \|Q_n\|_2^{1/2} \\
&= \mathcal{O}(K^{-p/(d+1)}).
\end{aligned} \tag{S49}$$

Recalling  $\Psi_n^\top(T_i, X_i)\phi^*$  is a sieve approximation to  $\tilde{\tau}(T_i, X_i)$ , we then have

$$\begin{aligned}
&E(\|m_{i,2}\|^2) \\
&\leq \sup_{(x,t) \in \mathbb{X} \times \mathbb{T}} \left| \left[ \tilde{\tau}(X = x, T = t) - E\{\tilde{\tau}(X, T) \mid X = x\} - \{\Psi(X = x, T = t) - \Gamma(X = x)\}^\top \phi^* \right] \right|^2 \\
&\quad \cdot E(\|\Psi(X, T) - \Gamma(X)\|^2) \\
&\leq \left[ 2\|\tilde{\tau} - \Psi_n^\top \phi^*\|_{\mathbb{X} \times \mathbb{T}}^2 + \sup_{x \in \mathbb{X}} 2 \left| E\{\tilde{\tau}(X, T) - \Psi_n^\top(X, T)\phi^* \mid X = x\} \right|^2 \right] \cdot (2\|\Psi\|_{\mathbb{X} \times \mathbb{T}}^2 + 2\|\Gamma\|_{\mathbb{X}}^2) \\
&\leq \left( 2\|\tilde{\tau} - \Psi_n^\top \phi^*\|_{\mathbb{X} \times \mathbb{T}}^2 + \sup_{x \in \mathbb{X}} 2 \left| E(\|\tilde{\tau} - \Psi_n^\top \phi^*\|_{\mathbb{X} \times \mathbb{T}}^2 \mid X = x) \right| \right) \cdot (2\|\Psi\|_{\mathbb{X} \times \mathbb{T}}^2 + 2\|\Gamma\|_{\mathbb{X}}^2) \\
&\leq \left( 4\|\tilde{\tau} - \Psi_n^\top \phi^*\|_{\mathbb{X} \times \mathbb{T}}^2 \right) \cdot (2\|\Psi\|_{\mathbb{X} \times \mathbb{T}}^2 + 2\|\Gamma\|_{\mathbb{X}}^2) \\
&= \mathcal{O}(K^{1-2p/(d+1)}),
\end{aligned} \tag{S50}$$

by Lemma S3, Proposition S1 and Lemma S6. By taking  $v_i = m_{i,2}$ ,  $A_n = C_3 K^{1-2p/(d+1)}$ ,  $d = K$ , and  $J = C_3 K^{-p/(d+1)}$  in Claim S7, then for any  $c > 0$ , there exists large enough yet fixed  $C_3 > 0$  such that

$$\Pr\left\{\|\Delta_{1,2} - E(\Delta_{1,2})\| > C_3 K^{-p/(d+1)} \sqrt{K/n}\right\} \leq c.$$



Therefore  $\|\Delta_{1,2} - E(\Delta_{1,2})\| = \mathcal{O}_P(K^{-p/(d+1)}\sqrt{K/n}) = o_P(K^{-p/(d+1)})$ . Then by (S49), one has

$$\|\Delta_{1,2}\| \leq \|\Delta_{1,2} - E(\Delta_{1,2})\| + \|E(\Delta_{1,2})\| = \mathcal{O}_P(K^{-p/(d+1)})$$

When  $\ell_n$  depends only on  $n$  and  $\|\ell_n\| = 1$ , then similar to (S49), we have

455

$$\begin{aligned} |E(\ell_n^\top m_{i,2})| &= \left| E \left[ E \{ \Gamma^\top(X) \phi^* - \tilde{\tau}(X, T) \mid X \} \ell_n^\top \Psi(X, T) \right] \right| \\ &= \mathcal{O}(K^{-p/(d+1)}). \end{aligned} \quad (\text{S51})$$

Also, similar to (S50) and by Lemma S5, we have

$$\begin{aligned} &E(\ell_n^\top m_{i,2})^2 \\ &\leq \sup_{(x,t) \in \mathbb{X} \times \mathbb{T}} \left| \left[ \tilde{\tau}(x, t) - E\{\tilde{\tau}(X, T) \mid X = x\} - \{\Psi(x, t) - \Gamma(x)\}^\top \phi^* \right] \right|^2 \\ &\quad \cdot E \left[ \ell_n^\top \left\{ \Psi(X, T) - \Gamma(X) \right\} \right]^2 \\ &\leq \left( 4 \|\tilde{\tau} - \Psi_n^\top \phi^*\|_{\mathbb{X} \times \mathbb{T}}^2 \right) \cdot \left( \|Q_n\|_2 + \|E(\Gamma \Gamma^\top)\|_2 \right) \\ &= \mathcal{O}(K^{-2p/(d+1)}). \end{aligned}$$

Take  $v_i = \ell_n^\top m_{i,2}$ ,  $d = 1$ ,  $A_n = C_4 K^{-2p/(d+1)}$ ,  $J = 2\sqrt{C_4} K^{-p/(d+1)}/c$  in Proposition S7. We then have for any fixed  $c > 0$  and sufficiently large  $C_4 > 0$ ,

$$\text{pr} \left\{ |P_n(\ell_n^\top m_{i,2}) - E(\ell_n^\top m_{i,2})| > 2\sqrt{C_4}/c K^{-p/(d+1)} n^{-1/2} \right\} \leq c,$$

which combining with (S51) implies that  $|\ell_n^\top \Delta_{1,2}| = |P_n(\ell_n^\top m_{i,2})| \leq |P_n(\ell_n^\top m_{i,2}) - E(\ell_n^\top m_{i,2})| + |E(\ell_n^\top m_{i,2})| = \mathcal{O}_P(K^{-p/(d+1)} n^{-1/2}) + \mathcal{O}_P(K^{-p/(d+1)}) = \mathcal{O}_P(K^{-p/(d+1)})$ .

460

**Proof of Lemma S9 (iii)** We now condition on  $\mathcal{E}_n$  with well-conditioned  $(\hat{m}, \hat{\Gamma})$ . We let  $m_{i,3} = [Y_i - m(X_i) - \{\Psi(T_i, X_i) - \Gamma(X_i)\}^\top \phi^*] \{\Gamma(X_i) - \hat{\Gamma}(X_i)\}$  and thus  $\Delta_{1,3} = P_n(m_{i,3})$ . Recall the nuisance functions and proposed estimators are trained independently. The conditional expectations then can be bounded as follows

465

$$\begin{aligned} &P(m_{i,3}) \\ &= P \left[ [Y - m(X) - \{\Psi(X, T) - \Gamma(X)\}^\top \phi^*] \{\Gamma(X) - \hat{\Gamma}(X)\} \right] \\ &= P \left[ E[Y - m(X) - \{\Psi(X, T) - \Gamma(X)\}^\top \phi^* \mid X] \{\Gamma(X) - \hat{\Gamma}(X)\} \right] \\ &= 0, \end{aligned} \quad (\text{S52})$$

where the last equality follows by  $E(Y \mid X) = m(X)$  and  $E\{\Psi^\top(X, T) \phi^* \mid X\} = \Gamma^\top(X) \phi^*$ ; thus  $E(\Delta_{1,3}) = 0$ . We also have

$$\begin{aligned} &P(\|m_{i,3}\|^2) \\ &= P \left[ [Y - m(X) - \{\Psi(X, T) - \Gamma(X)\}^\top \phi^*]^2 \|\Gamma(X) - \hat{\Gamma}(X)\|^2 \right] \\ &\leq P \left[ [Y - m(X) - \{\Psi(X, T) - \Gamma(X)\}^\top \phi^*]^2 \|\Gamma - \hat{\Gamma}\|_{\mathbb{X}}^2 \right] \\ &= \mathcal{O}(1) \cdot \mathcal{O}(K r_\gamma'^2 e_n) \\ &= \mathcal{O}(K r_\gamma'^2 e_n), \end{aligned} \quad (\text{S53})$$

where the inequality follows by

$$\begin{aligned}
P\left[\left[Y - m(X) - \{\Psi(X, T) - \Gamma(X)\}^\top \phi^*\right]^2\right] &\leq 2E\left[\left\{Y - m(X)\right\}^2\right] + 2E\left[\left\{\{\Psi(X, T) - \Gamma(X)\}^\top \phi^*\right\}^2\right] \\
&= 2E\left\{\text{Var}(Y \mid X)\right\} + 2(\phi^*)^\top R_n \phi^* \\
&\leq 2E\left\{\text{Var}(Y \mid X)\right\} + 2\|\phi^*\|^2 \|R_n\|_2 \\
&= \mathcal{O}(1), \quad (\text{Assumptions S5 and Lemma S5})
\end{aligned} \tag{S54}$$

and last two equalities are by the event defined in  $\mathcal{E}_n$ . Let  $v_i = m_{i,3}$ ,  $d = K$ ,  $A_n = C_5 K r_\gamma'^2 e_n$ , and  $J = c_5 r_\gamma'$  in Proposition S7. We have when  $n \rightarrow +\infty$ ,

$$\begin{aligned}
\text{pr}_n\left(\|\Delta_{1,3}\| > c_5 r_\gamma' \sqrt{K/n}\right) &\leq \frac{4C_5 K r_\gamma'^2 e_n}{c_5^2 r_\gamma'^2 K} \\
&= 4C_5 e_n / c_5^2 \\
&\rightarrow 0,
\end{aligned} \tag{S55}$$

for some sufficiently large yet fixed  $C_5 > 0$  and any fixed  $c_5 > 0$ . We thus have, conditional on  $\mathcal{E}_n$ ,  $\|\Delta_{1,3}\| = o_P(r_\gamma' \sqrt{K/n})$ . Recall  $\mathcal{E}_n$  is a event happens wpa1. We thus can directly uncondition  $\mathcal{E}_n$  and have  $\|\Delta_{1,3}\| = o_P(r_\gamma' \sqrt{K/n})$ . To be more specific, for any fixed  $C_6 > 0$ , we have

$$\begin{aligned}
&\text{pr}\left(\|\Delta_{1,3}\| > c_5 r_\gamma' \sqrt{K/n}\right) \\
&= \text{pr}\left(\left\{\|\Delta_{1,3}\| > c_5 r_\gamma' \sqrt{K/n}\right\} \cap \mathcal{E}_n\right) + \text{pr}\left(\left\{\|\Delta_{1,3}\| > c_5 r_\gamma' \sqrt{K/n}\right\} \cap \mathcal{E}_n^c\right) \\
&\leq \text{pr}\left(\left\{\|\Delta_{1,3}\| > c_5 r_\gamma' \sqrt{K/n}\right\} \cap \mathcal{E}_n\right) + \text{pr}(\mathcal{E}_n^c) \\
&= \text{pr}_n\left(\|\Delta_{1,3}\| > c_5 r_\gamma' \sqrt{K/n}\right) \cdot \text{pr}(\mathcal{E}_n) + \text{pr}(\mathcal{E}_n^c) \\
&\rightarrow 0,
\end{aligned} \tag{S56}$$

by  $\text{pr}(\mathcal{E}_n^c) \rightarrow 0$ ,  $\text{pr}(\mathcal{E}_n) \leq 1$ , and (S55).

Now we bound  $|\ell_n^\top \Delta_{1,3}|$ . Similar to (S52), we have  $P(\ell_n^\top m_{i,3}) = 0$ . Similar to (S53), we have

475

$$\begin{aligned}
&P(\ell_n^\top m_{i,3})^2 \\
&= P\left[\left[Y - m(X) - \{\Psi(X, T) - \Gamma(X)\}^\top \phi^*\right]^2 \left[\ell_n^\top \{\Gamma(X) - \hat{\Gamma}(X)\}\right]^2\right] \\
&\leq 3P\left[\left\{Y - m(X)\right\}^2 \left[\ell_n^\top \{\Gamma(X) - \hat{\Gamma}(X)\}\right]^2\right] \\
&\quad + 3P\left[\left\{\{\Psi(X, T) - \Gamma(X)\}^\top \phi^* - [\tilde{\tau}(X, T) - E\{\tilde{\tau}(X, T) \mid X\}]\right\}^2 \left[\ell_n^\top \{\Gamma(X) - \hat{\Gamma}(X)\}\right]^2\right] \\
&\quad + 3P\left[\left\{[\tilde{\tau}(X, T) - E\{\tilde{\tau}(X, T) \mid X\}]\right\}^2 \left[\ell_n^\top \{\Gamma(X) - \hat{\Gamma}(X)\}\right]^2\right],
\end{aligned} \tag{S57}$$

by the triangle inequality. The first term in (S57) can be bounded by the law of total expectation,

$$\begin{aligned}
& P\left[\{Y - m(X)\}^2 [\ell_n^T \{\Gamma(X) - \hat{\Gamma}(X)\}]^2\right] \\
&= P\left[\text{Var}(Y \mid X) [\ell_n^T \{\Gamma(X) - \hat{\Gamma}(X)\}]^2\right] \\
&\leq \sup_{x \in \mathbb{X}} \text{Var}(Y \mid X = x) \cdot P\left[\ell_n^T \{\Gamma(X) - \hat{\Gamma}(X)\}\right]^2 \\
&\lesssim P\left[\ell_n^T \{\Gamma(X) - \hat{\Gamma}(X)\}\right]^2 \\
&\leq \sup_{\|\ell\|=1} P\left[\ell^T \{\Gamma(X) - \hat{\Gamma}(X)\}\right]^2 \\
&= \|P[\{\Gamma(X) - \hat{\Gamma}(X)\} \{\Gamma(X) - \hat{\Gamma}(X)\}^T]\|_2 \\
&= \mathcal{O}(r_\gamma^2 e_n^2),
\end{aligned} \tag{S58}$$

where the second inequality follows by Assumption S5 and  $\mathcal{E}_n$ . For the second term on the right-hand side of (S57), we first note

$$\begin{aligned}
& \sup_{(x,t) \in \mathbb{X} \times \mathbb{T}} \left| \tilde{\tau}(x,t) - E\{\tilde{\tau}(X,T) \mid X = x\} - \{\Psi(x,t) - \Gamma(x)\}^T \phi^* \right|^2 \\
&= \mathcal{O}(K^{-2p/(d+1)}),
\end{aligned}$$

by Proposition S1 similar to (S50). Then we have

$$\begin{aligned}
& P\left[\left\{\Psi(X,T) - \Gamma(X)\right\}^T \phi^* - [\tilde{\tau}(X,T) - E\{\tilde{\tau}(X,T) \mid X\}]\right]^2 [\ell_n^T \{\Gamma(X) - \hat{\Gamma}(X)\}]^2 \\
&\leq \sup_{(x,t) \in \mathbb{X} \times \mathbb{T}} \left| \tilde{\tau}(x,t) - E\{\tilde{\tau}(X,T) \mid x\} - \{\Psi(x,t) - \Gamma(x)\}^T \phi^* \right|^2 \cdot P\left[\ell_n^T \{\Gamma(X) - \hat{\Gamma}(X)\}\right]^2 \\
&= \mathcal{O}(K^{-2p/(d+1)} r_\gamma^2 e_n^2).
\end{aligned}$$

For the third term on the right-hand side of (S57), we note  $\|\tilde{\tau}\|_{\mathbb{X} \times \mathbb{T}} \lesssim 1$  as  $\tilde{\tau}$  is in the Hölder class, and thus  $\|E(\tilde{\tau} \mid \cdot)\|_{\mathbb{X}} \leq \sup_{x \in \mathbb{X}} E(\|\tilde{\tau}\|_{\mathbb{X} \times \mathbb{T}} \mid X = x) = \|\tilde{\tau}\|_{\mathbb{X} \times \mathbb{T}} \lesssim 1$ . Then we have

$$\begin{aligned}
& P\left[\left\{\tilde{\tau}(X,T) - E\{\tilde{\tau}(X,T) \mid X\}\right\}^2 [\ell_n^T \{\Gamma(X) - \hat{\Gamma}(X)\}]^2\right] \\
&\leq \|\tilde{\tau} - E\{\tilde{\tau}(X,T) \mid X = \cdot\}\|_{\mathbb{X} \times \mathbb{T}}^2 \cdot P\left[\ell_n^T \{\Gamma(X) - \hat{\Gamma}(X)\}\right]^2 \\
&\leq \left[2\|\tilde{\tau}\|_{\mathbb{X} \times \mathbb{T}}^2 + 2\|E\{\tilde{\tau}(X,T) \mid X = \cdot\}\|_{\mathbb{X}}^2\right] \cdot P\left[\ell_n^T \{\Gamma(X) - \hat{\Gamma}(X)\}\right]^2 \\
&\lesssim P\left[\ell_n^T \{\Gamma(X) - \hat{\Gamma}(X)\}\right]^2 \\
&= \mathcal{O}(r_\gamma^2 e_n^2),
\end{aligned}$$

similar to (S58). In summary, we have

$$P(\ell_n^T m_{i,3})^2 = \mathcal{O}(r_\gamma^2 e_n^2).$$

By taking  $v_i = \ell_n^T m_{i,3}$ ,  $d = 1$ ,  $A_n = C_6 r_\gamma^2 e_n^2$ ,  $J = c_6 r_\gamma$  in Proposition S7, we have

$$\text{pr}_n\left(|\ell_n^T \Delta_{1,3}| > c_6 r_\gamma / \sqrt{n}\right) \leq \frac{4C_6 r_\gamma^2 e_n^2}{r_\gamma^2 c_6^2} = 4C_6 e_n^2 / c_6^2 \rightarrow 0.$$

Thus similar to (S56), we can directly uncondition  $\mathcal{E}_n$  and conclude  $|\ell_n^T \Delta_{1,3}| = o_P(r_\gamma / \sqrt{n})$ .

Proof of Lemma S9 (iv) We still condition on  $\mathcal{E}_n$ . We let  $m_{i,4} = [m(X_i) - \hat{m}(X_i) - \{\Gamma(X_i) - \hat{\Gamma}(X_i)\}^\top \phi^*] \{\Psi(X_i, T_i) - \Gamma(X_i)\}$ , thus  $\Delta_{1,4} = P_n(m_{i,4})$ . By the law of total expectation we have,

$$\begin{aligned} & P[m_{i,4}] \\ &= P\left[[m(X) - \hat{m}(X) - \{\Gamma(X) - \hat{\Gamma}(X)\}^\top \phi^*] \{\Psi(X, T) - \Gamma(X)\}\right] \\ &= P\left[[m(X) - \hat{m}(X) - \{\Gamma(X) - \hat{\Gamma}(X)\}^\top \phi^*] P\{\Psi(X, T) - \Gamma(X) \mid X\}\right] \\ &= 0. \end{aligned} \tag{S59}$$

By the triangle inequality, we have

$$\begin{aligned} & P\|m_{i,4}\|^2 \\ &\leq 2P\left[\{m(X) - \hat{m}(X)\}^2 \|\Psi(X, T) - \Gamma(X)\|^2\right] + 2P\left[\{\{\Gamma(X) - \hat{\Gamma}(X)\}^\top \phi^*\}^2 \|\Psi(X, T) - \Gamma(X)\|^2\right] \\ &\leq 2\|\Psi - \Gamma\|_{\mathbb{X} \times \mathbb{T}}^2 \left[P\{m(X) - \hat{m}(X)\}^2 + \|\phi^*\|^2 P[\{\{\Gamma(X) - \hat{\Gamma}(X)\}^\top (\phi^* / \|\phi^*\|)\}^2]\right] \\ &\leq 2\|\Psi - \Gamma\|_{\mathbb{X} \times \mathbb{T}}^2 \left\{\|\hat{m} - m\|_{\mathcal{L}_{\mathcal{P}}}^2 + \|\phi^*\|^2 P[\{\hat{\Gamma}(X) - \Gamma(X)\} \{\hat{\Gamma}(X) - \Gamma(X)\}^\top]_2\right\} \\ &= \mathcal{O}(Kr_m^2 e_n^2 + Kr_\gamma^2 e_n^2), \end{aligned}$$

where the last equality follows by  $\mathcal{E}_n$ . By taking  $v_i = \ell_n^\top m_{i,4}$ ,  $d = K$ ,  $A_n = C_7(Kr_m^2 e_n^2 + Kr_\gamma^2 e_n^2)$ ,  $J =$   
490  $c_7 r_m + c_7 r_\gamma$  in Proposition S7, for some sufficiently large yet fixed  $C_7 > 0$  and any given  $c_7 > 0$ ,

$$\begin{aligned} & \text{pr}_n \left\{ \|\Delta_{1,4}\| > c_7(r_m + r_\gamma) \sqrt{K/n} \right\} \\ &\leq \frac{4C_7(Kr_m^2 e_n^2 + Kr_\gamma^2 e_n^2)}{c_7^2(r_m + r_\gamma)^2 K} \\ &\lesssim e_n^2 \\ &\rightarrow 0. \end{aligned}$$

which implies  $\|\Delta_{1,4}\| = o_P(r_m \sqrt{K/n} + r_\gamma \sqrt{K/n})$  by directly unconditioning  $\mathcal{E}_n$ , similar to (S56).

On the other hand, similar to (S59) one has  $P(\ell_n^\top m_{i,4}) = 0$ . Also we have

$$\begin{aligned} & P(\ell_n^\top m_{i,4})^2 \\ &= P\left[[m(X) - \hat{m}(X) - \{\Gamma(X) - \hat{\Gamma}(X)\}^\top \phi^*]^2 \{\ell_n^\top \Psi(X, T) - \ell_n^\top \Gamma(X)\}^2\right] \\ &\leq 2\left[\|m - \hat{m}\|_{\mathbb{X}}^2 + \|\{\Gamma - \hat{\Gamma}\}^\top \phi^*\|_{\mathbb{X}}^2\right] \cdot P\left[\ell_n^\top \Psi(X, T) - \ell_n^\top \Gamma(X)\right]^2 \\ &\leq 4e_n^2 \|R_n\|_2 \\ &= \mathcal{O}(e_n^2), \end{aligned}$$

where the second inequality is due to  $\mathcal{E}_n$ , and the last equality follows by Lemma S5 such that  $\|R_n\|_2 \lesssim 1$ . By taking  $v_i = \ell_n^\top m_{i,4}$ ,  $d = 1$ ,  $A_n = C_8 e_n^2$ , and  $J = c_8$  for some sufficiently large yet fixed  $C_8 > 0$  and any given  $c_8 > 0$ , we then have

$$\text{pr}_n \left( |\ell_n^\top \Delta_{1,4}| > c_8 1/\sqrt{n} \right) \leq \frac{4C_8 e_n^2}{c_8^2} \rightarrow 0,$$

which, after unconditioning  $\mathcal{E}_n$  similar to (S56), we have  $|\ell_n^\top \Delta_{1,4}| = o_P(1/\sqrt{n})$ .

**Proof of Lemma S9 (v)** We still condition on  $\mathcal{E}_n$ . Let  $m_{i,5} = [m(X_i) - \hat{m}(X_i) - \{\Gamma(X_i) - \hat{\Gamma}(X_i)\}^\top \phi^*] \{\Gamma(X_i) - \hat{\Gamma}(X_i)\}$ , and thus  $\Delta_{1,5} = P_n(m_{i,5})$ . First we have

$$\begin{aligned}
& \|P(m_{i,5})\| \\
&= \sup_{\|\ell\|=1} \left| P \left[ [m(X) - \hat{m}(X) - \{\Gamma(X) - \hat{\Gamma}(X)\}^\top \phi^*] \{\ell^\top \Gamma(X) - \ell^\top \hat{\Gamma}(X)\} \right] \right| \\
&\leq \sup_{\|\ell\|=1} \left| P \left[ \{m(X) - \hat{m}(X)\} \{\ell^\top \Gamma(X) - \ell^\top \hat{\Gamma}(X)\} \right] \right| \\
&+ \|\phi^*\| \sup_{\|\ell\|=1} \left| P \left[ [\{\Gamma(X) - \hat{\Gamma}(X)\}^\top \phi^* / \|\phi^*\|] \{\ell^\top \Gamma(X) - \ell^\top \hat{\Gamma}(X)\} \right] \right| \\
&\leq \|\hat{m} - m\|_{\mathcal{L}_P^2} \|P[\{\Gamma(X) - \hat{\Gamma}(X)\} \{\Gamma(X) - \hat{\Gamma}(X)\}^\top]\|_2^{1/2} \\
&+ \|\phi^*\| \sup_{\|\ell\|=1} \left| P \left[ (\phi^* / \|\phi^*\|)^\top \{\Gamma(X) - \hat{\Gamma}(X)\} \{\Gamma(X) - \hat{\Gamma}(X)\}^\top \ell \right] \right| \\
&\leq \|\hat{m} - m\|_{\mathcal{L}_P^2} \|P[\{\Gamma(X) - \hat{\Gamma}(X)\} \{\Gamma(X) - \hat{\Gamma}(X)\}^\top]\|_2^{1/2} + \|\phi^*\| \|P[\{\Gamma(X) - \hat{\Gamma}(X)\} \{\Gamma(X) - \hat{\Gamma}(X)\}^\top]\|_2 \\
&= \mathcal{O}(e_n^2 r_m r_\gamma + e_n^2 r_\gamma^2) \\
&= o(r_m r_\gamma + r_\gamma^2),
\end{aligned} \tag{S60}$$

where the second inequality follows by Cauchy–Schwarz inequality; the last equality follows by  $\mathcal{E}_n$ , and Proposition S1 such that  $\|\phi^*\| \lesssim 1$ . On the other hand,

$$\begin{aligned}
& P(\|m_{i,5}\|^2) \\
&\leq 2P[\{m(X) - \hat{m}(X)\}^2 \|\Gamma(X) - \hat{\Gamma}(X)\|^2] + 2P[\{\{\Gamma(X) - \hat{\Gamma}(X)\}^\top \phi^*\}^2 \|\Gamma(X) - \hat{\Gamma}(X)\|^2] \\
&\leq 2\|\Gamma - \hat{\Gamma}\|_\infty^2 \cdot [\|m - \hat{m}\|_{\mathcal{L}_P^2}^2 + \|\phi^*\|^2 \|P[\{\hat{\Gamma}_n(X) - \Gamma_n(X)\} \{\hat{\Gamma}_n(X) - \Gamma_n(X)\}^\top]\|_2^2] \\
&= \mathcal{O}(e_n^4 K r_\gamma'^2 r_m^2 + e_n^4 K r_\gamma'^2 r_\gamma^2).
\end{aligned}$$

Then by taking  $v_i = m_{i,5}$ ,  $d = K$ ,  $A_n = C_9 e_n^4 K r_\gamma'^2 r_m^2 + C_9 e_n^4 K r_\gamma'^2 r_\gamma^2$ , and  $J = c_9(r_\gamma' r_m + r_\gamma' r_\gamma)$  in Proposition S7, we have, for any fixed  $c_9 > 0$  and some sufficiently large yet fixed  $C_9 > 0$ ,

$$\begin{aligned}
\Pr_n \left\{ \|\Delta_{1,5} - P(m_{i,5})\| > c_9(r_\gamma' r_m + r_\gamma' r_\gamma) \sqrt{K/n} \right\} &\leq \frac{4C_9 e_n^4 K r_\gamma'^2 r_m^2 + 4C_9 e_n^4 K r_\gamma'^2 r_\gamma^2}{c_9^2 (r_\gamma' r_m + r_\gamma' r_\gamma)^2 K} \\
&\lesssim e_n^4 \\
&\rightarrow 0.
\end{aligned}$$

Thus under  $\mathcal{E}_n$ , we have

$$\begin{aligned}
\|\Delta_{1,5}\| &\leq \|P(m_{i,5})\| + \|\Delta_{1,5} - P(m_{i,5})\| \\
&= o_P(r_m r_\gamma + r_\gamma^2 + r_\gamma' r_m \sqrt{K/n} + r_\gamma' r_\gamma \sqrt{K/n}).
\end{aligned}$$

505 Similar to (S56), we can uncondition  $\mathcal{E}_n$ , and the same bound of  $\|\Delta_{1,5}\|$  still holds.

On the other hand, by (S60) we further have

$$\begin{aligned}
|P(\ell_n^\top m_{i,5})| &\leq \sup_{\|\ell\|=1} |P(\ell^\top m_{i,5})| \\
&= \|P(m_{i,5})\| \\
&= \mathcal{O}(e_n^2 r_m r_\gamma + e_n^2 r_\gamma^2) \\
&= o(r_m r_\gamma + r_\gamma^2).
\end{aligned}$$

In addition, under  $\mathcal{E}_n$ , we have

$$\begin{aligned}
P(\ell_n^T m_{i,5})^2 &= P\left[m(X) - \hat{m}(X) - \{\Gamma(X) - \hat{\Gamma}(X)\}^T \phi^*\right]^2 \{\ell_n^T \Gamma(X) - \ell_n^T \hat{\Gamma}(X)\}^2 \\
&\leq 2\left\{\|m - \hat{m}\|_{\mathbb{X}}^2 + \|(\Gamma - \hat{\Gamma})^T \phi^*\|_{\mathbb{X}}^2\right\} \cdot P\left\{\ell_n^T \Gamma(X) - \ell_n^T \hat{\Gamma}(X)\right\}^2 \\
&\lesssim e_n^2 \|P[\{\hat{\Gamma}(X) - \Gamma(X)\}\{\hat{\Gamma}(X) - \Gamma(X)\}^T]\|_2 \\
&= \mathcal{O}(e_n^2 r_\gamma^2).
\end{aligned}$$

Then by taking  $v_i = \ell_n^T m_{i,5}$ ,  $d = 1$ ,  $A_n = C_{10} e_n^2 r_\gamma^2$ , and  $J = c_{10}$  in Proposition S7, we have, for any fixed  $c_{10} > 0$  and some sufficiently large yet fixed  $C_{10} > 0$ ,

$$\Pr_n\left\{|\ell_n^T \Delta_{1,5} - P(\ell_n^T m_{i,5})| > c_{10} r_\gamma / \sqrt{n}\right\} \leq \frac{4C_{10} e_n^2 r_\gamma^2}{c_{10}^2 r_\gamma^2} \rightarrow 0.$$

Thus under  $\mathcal{E}_n$ ,  $|\ell_n^T \Delta_{1,5}| \leq |\ell_n^T \Delta_{1,5} - P(\ell_n^T m_{i,5})| + |P(\ell_n^T m_{i,5})| = o_P(r_\gamma / \sqrt{n} + r_m r_\gamma + r_\gamma^2)$ . Similar to (S56), we can then uncondition  $\mathcal{E}_n$ , and the same bound of  $|\ell_n^T \Delta_{1,5}|$  still holds.  $\square$

#### S5.4. Proof of Proposition ??

**Proof of Proposition ?? (i)** We first consider a more general minimization problem,

$$\begin{aligned}
q &= \arg \min_{h \in \mathcal{L}_p^2(X, T)} E\left\{Y - m(X) - h(X, T)\right\}^2 \\
&= \arg \min_{h \in \mathcal{L}_p^2(X, T)} E\left\{Y - E(Y | X) - h(X, T)\right\}^2.
\end{aligned} \tag{S61}$$

Treat  $Y - E(Y | X)$  as a random variable. Then based on the least-square form of (S61), we know (S61) is minimized, if and only if  $q(X, T)$  is the conditional mean of  $Y - E(Y | X)$  given  $X$  and  $T$  a.s., or equivalently,

$$q(X, T) = E\{Y - E(Y | X) | X, T\} \text{ a.s.} \tag{S62}$$

We show the above statement by contradiction. Suppose  $q(X, T)$  is not a.s.  $E\{Y - E(Y | X) | X, T\}$ . Then we have

$$q(X, T) = E\{Y - E(Y | X) | X, T\} + u(X, T) \text{ a.s.,} \tag{S63}$$

for some  $u(X, T) \neq 0$  with probability larger than 0. We then have

$$\begin{aligned}
&E\left\{Y - E(Y | X) - q(X, T)\right\}^2 \\
&= E\left[Y - E(Y | X) - E\{Y - E(Y | X) | X, T\} - u(X, T)\right]^2 \\
&= E\left[Y - E(Y | X) - E\{Y - E(Y | X) | X, T\}\right]^2 \\
&\quad - 2E\left[\left[Y - E(Y | X) - E\{Y - E(Y | X) | X, T\}\right]u(X, T)\right] + E\{u^2(X, T)\} \\
&= E\left[Y - E(Y | X) - E\{Y - E(Y | X) | X, T\}\right]^2 + E\{u^2(X, T)\} \\
&> E\left[Y - E(Y | X) - E\{Y - E(Y | X) | X, T\}\right]^2,
\end{aligned} \tag{S64}$$

where by the law of total expectation,

$$\begin{aligned}
& E\left[\left[Y - E(Y | X) - E\{Y - E(Y | X) | X, T\}\right]u(X, T)\right] \\
&= E\left[E\left[Y - E(Y | X) - E\{Y - E(Y | X) | X, T\} | X, T\right]u(X, T)\right] \\
&= E\{0 \cdot u(X, T)\} \\
&= 0.
\end{aligned}$$

Thus (S64) implies that  $q(X, T)$  satisfies (S61) if and only if (S62) holds. We then have

$$\begin{aligned}
q(X, T) &= E\{Y - E(Y | X) | X, T\} \\
&= E(Y | X, T) - E(Y | X) \\
&= E(Y | X, T) - E\{E(Y | X, T) | X\} \\
&= \tau(X, T) - E\{\tau(X, T) | X\}, \text{ a.s..}
\end{aligned} \tag{S65}$$

The last equality follows by  $\tau(X, T) = E(Y | X, T) - E(Y | X, T = 0)$  under Assumptions ?? and ?. Since  $\tau \in \mathcal{L}_{\mathcal{P}}^2(X, T)$ , it is easy to verify that  $q$  is also in  $\mathcal{L}_{\mathcal{P}}^2(X, T)$  based on (S65) and the Cauchy-Schwarz inequality,

525

$$\begin{aligned}
E[\tau(X, T) - E\{\tau(X, T) | X\}]^2 &\leq 2E\{\tau^2(X, T)\} + 2E[E\{\tau(X, T) | X\}]^2 \\
&\leq 2E\{\tau^2(X, T)\} + 2E[E\{\tau^2(X, T) | X\}] \\
&= 4E\{\tau^2(X, T)\} \\
&< +\infty.
\end{aligned}$$

Comparing (S61) and (??), if  $h \in \mathcal{L}_{\mathcal{P}}^2(X, T)$  is a minimum of  $L_c(h)$ ,  $h(X, T) - E\{h(X, T) | X\}$  must minimize the general problem in (S61), i.e.,

$$\begin{aligned}
h(X, T) - E\{h(X, T) | X\} &= q(X, T) \\
&= \tau(X, T) - E\{\tau(X, T) | X\} \quad \text{a.s.,}
\end{aligned}$$

which is equivalent to

$$h(X, T) = \tau(X, T) + [E\{h(X, T) | X\} - E\{\tau(X, T) | X\}] \quad \text{a.s.} \tag{S66}$$

by (S65). Thus any  $h \in \mathcal{L}_{\mathcal{P}}^2(X, T)$  minimizing (??) must satisfy

$$h(X, T) = \tau(X, T) + s(X) \quad \text{a.s.,}$$

for some  $s \in \mathcal{L}_{\mathcal{P}}^2(X)$  such that  $s(x) = E\{h(X, T) | X = x\} - E\{\tau(X, T) | X = x\}$ .

530

On the other hand, for arbitrary  $s \in \mathcal{L}_{\mathcal{P}}^2(X)$ , if  $h(X, T) = \tau(X, T) + s(X)$  a.s,  $h$  must satisfy

$$\begin{aligned}
h(X, T) - E\{h(X, T) | X\} &= \tau(X, T) - E\{\tau(X, T) | X\} \\
&= q(X, T), \quad \text{a.s.,}
\end{aligned}$$

recalling  $q$  is the solution of the general minimization problem (S61). It is also easy to see that  $h \in \mathcal{L}_{\mathcal{P}}^2(X, T)$  as both  $s$  and  $\tau$  have bounded  $\mathcal{L}_{\mathcal{P}}^2$  norms. Therefore,  $h$  is a minimum of  $L_c(h)$ .

Summarizing the above results, we conclude that the solution set in  $\mathcal{L}_{\mathcal{P}}^2(X, T)$  that minimizes  $L_c(h)$  is exactly  $\mathcal{S} = \{h | h(X, T) = \tau(X, T) + s(X) \text{ a.s., for any } s(x) \in \mathcal{L}_{\mathcal{P}}^2(X)\}$ .

535

**Heuristic proof of Proposition ?? (ii)** Before heading to the formal proof of Proposition ?? (ii), we first give an explanation about how (??) narrows  $\mathcal{S}$  to  $\mathcal{S}^\natural$ . This explanation also gives some intuitions for the formal proof.

Notice that any other solution  $h$  in  $\mathcal{S}$  but not in  $\mathcal{S}^\natural$ , satisfies that  $h(X, T) = \tau(X, T) + s(X)$  a.s., with some  $s(X)$  that is not a.s. zero, i.e.,  $\text{pr}[\Omega = \{X \text{ satisfies } s(X) \neq 0\}] > 0$ . Therefore, under the positivity

540

assumption such that  $\text{pr}(T = 0 \mid X = x) > \epsilon'$  for some fixed  $\epsilon' > 0$  and any  $x \in \mathbb{X}$ , we have

$$\begin{aligned} \text{pr}\{h(X, 0) = \tau(X, 0) + s(X) = s(X) \neq 0\} &\geq \text{pr}[\{T = 0\} \cap \Omega] = \text{pr}(T = 0 \mid \Omega)\text{pr}(\Omega) \\ &\geq \epsilon' \cdot \text{pr}(\Omega) > 0, \end{aligned} \quad (\text{S67})$$

which is in conflict with (??) such that  $h(X, 0) = 0$  with probability 1.

**Formal proof of Proposition ?? (ii)** Write the optimization problem (??) for the bianry treatment as

$$\arg \min_{h \in \{h \mid h(\cdot, 1) \in \mathcal{L}_{\mathcal{P}}^2(X) \text{ and } h(X, 0) = 0 \text{ a.s.}\}} E[Y - m(X) - \{T - e(X)\}h(X, 1)]^2. \quad (\text{S68})$$

Since the objective function above only involves  $h(\cdot, 1)$ , we consider a simplified problem

$$\arg \min_{h' \in \mathcal{L}_{\mathcal{P}}^2(X)} E[Y - m(X) - \{T - e(X)\}h'(X)]^2. \quad (\text{S69})$$

545 Let  $\mathcal{S}'$  be the solution set of (S69), and let  $\tilde{\mathcal{S}}^{\natural}$  be the solution set of (??) and thus is also the solution set of (S68). In the following, we show

$$\tilde{\mathcal{S}}^{\natural} = \{h \mid h(X, T) = \tau(X, T) \text{ a.s.}\} = \mathcal{S}^{\natural} \quad (\text{S70})$$

and thus finish the proof.

Comparing (S68) and (S69), we have that any  $h$  being a solution of (S68) must satisfy

$$h(X, 1) = h'(X) \text{ a.s..}$$

550 On the other hand, by the constraint of (S68), we also have  $h(X, 0) = 0$  a.s., when  $h \in \tilde{\mathcal{S}}^{\natural}$ . Therefore we have

$$\tilde{\mathcal{S}}^{\natural} \subseteq \mathcal{S}^{\natural\natural} = \{h \mid h(X, 1) = h'(X) \text{ a.s. for any } h' \in \mathcal{S}', \text{ and } h(X, 0) = 0 \text{ a.s.}\}. \quad (\text{S71})$$

It is also easy to check that if  $h \in \mathcal{S}^{\natural\natural}$ ,  $h(\cdot, 1)$  must minimize the objective function in (S68). Meanwhile, if  $h \in \mathcal{S}^{\natural\natural}$ , we also have  $h(\cdot, 1) \in \mathcal{L}_{\mathcal{P}}^2(X)$  as  $h' \in \mathcal{L}_{\mathcal{P}}^2(X)$  and  $h(X, 0) = 0$  a.s., thus  $h$  satisfies all the constraints and is a solution of (S68). So  $\mathcal{S}^{\natural\natural} \subseteq \tilde{\mathcal{S}}^{\natural}$ , and by (S71), we have

$$\tilde{\mathcal{S}}^{\natural} = \mathcal{S}^{\natural\natural} = \{h \mid h(X, 1) = h'(X) \text{ a.s. for any } h' \in \mathcal{S}', \text{ and } h(X, 0) = 0 \text{ a.s.}\}. \quad (\text{S72})$$

For simplicity, we denote  $\tau(x) = \tau(x, 1)$ . Therefore, we have  $\tau(\cdot) \in \mathcal{L}_{\mathcal{P}}^2(X)$  as  $\tau(\cdot, 1) \in \mathcal{L}_{\mathcal{P}}^2(X)$ . We first prove that,

$$\mathcal{S}' = \{h' \mid h'(X) = \tau(X) \text{ a.s.}\}. \quad (\text{S73})$$

Any  $h' \in \mathcal{L}_{\mathcal{P}}^2(X)$  can be written as  $h'(x) = \tau(x) + s'(x)$ , where  $s'(x) = \tau(x) - h'(x) \in \mathcal{L}_{\mathcal{P}}^2(X)$  since both  $h'(x)$  and  $\tau(x)$  are in  $\mathcal{L}_{\mathcal{P}}^2(X)$ . Then solving (S69) is equivalent to solving

$$\arg \min_{s' \in \mathcal{L}_{\mathcal{P}}^2(X)} E[Y - m(X) - \{T - e(X)\}\{s'(X) + \tau(X)\}]^2. \quad (\text{S74})$$

The above square loss function can be decomposed into

$$\begin{aligned} &E[Y - m(X) - \{T - e(X)\}\{s'(X) + \tau(X)\}]^2 \\ &= E\left[\left[Y - m(X) - \{T - e(X)\}\tau(X)\right] - [\{T - e(X)\}s'(X)]\right]^2 \\ &= E[Y - m(X) - \{T - e(X)\}\tau(X)]^2 \\ &\quad - 2E\left[\left[Y - m(X) - \{T - e(X)\}\tau(X)\right][\{T - e(X)\}s'(X)]\right] \\ &\quad + E[\{T - e(X)\}s'(X)]^2. \end{aligned} \quad (\text{S75})$$



For the second term on the right-hand side of (S75),

$$\begin{aligned}
& E\left[\left[Y - m(X) - \{T - e(X)\}\tau(X)\right]\left[\{T - e(X)\}s'(X)\right]\right] \\
&= E\left[E\left[Y - m(X) - \{T - e(X)\}\tau(X) \mid X, T\right]\left[\{T - e(X)\}s'(X)\right]\right] \\
&= E\left[0 \cdot \left[\{T - e(X)\}s'(X)\right]\right] \\
&= 0,
\end{aligned}$$

where the first equality follows by the law of total expectation, and the second inequality follows by

560

$$\begin{aligned}
& E\left[Y - m(X) - \{T - e(X)\}\tau(X) \mid X, T\right] \\
&= \mu(X, T) - m(X) - \{T - e(X)\}\tau(X) \\
&= E(Y \mid X, T) - E(Y \mid X) - \{T - \text{pr}(T = 1 \mid X)\}\{E(Y \mid X, T = 1) - E(Y \mid X, T = 0)\} \\
&= E(Y \mid X, T) - \{\text{pr}(T = 1 \mid X)E(Y \mid X, T = 1) + \text{pr}(T = 0 \mid X)E(Y \mid X, T = 0)\} \\
&\quad - \{T - \text{pr}(T = 1 \mid X)\}\{E(Y \mid X, T = 1) - E(Y \mid X, T = 0)\} \\
&= TE(Y \mid X, T = 1) + (1 - T)E(Y \mid X, T = 0) \\
&\quad - \text{pr}(T = 1 \mid X)E(Y \mid X, T = 1) - \{1 - \text{pr}(T = 1 \mid X)\}E(Y \mid X, T = 0) \\
&\quad - \{T - \text{pr}(T = 1 \mid X)\}\{E(Y \mid X, T = 1) - E(Y \mid X, T = 0)\} \\
&= TE(Y \mid X, T = 1) - TE(Y \mid X, T = 0) \\
&\quad - \text{pr}(T = 1 \mid X)E(Y \mid X, T = 1) + \text{pr}(T = 1 \mid X)E(Y \mid X, T = 0) \\
&\quad - \{T - \text{pr}(T = 1 \mid X)\}\{E(Y \mid X, T = 1) - E(Y \mid X, T = 0)\} \\
&= 0,
\end{aligned}$$

where the first equality follows by the definition of  $\mu(x, t)$ , the third equality follows by the law of total expectation, and the fourth equality follows by  $\text{pr}(T = 0 \mid X = x) = 1 - \text{pr}(T = 1 \mid X = x)$  and

$$\begin{aligned}
E(Y \mid X, T) &= I(T = 1)E(Y \mid X, T = 1) + I(T = 0)E(Y \mid X, T = 0) \\
&= TE(Y \mid X, T = 1) + (1 - T)E(Y \mid X, T = 0).
\end{aligned}$$

For the third term on the right-hand side of (S75), if  $s(X)$  is not 0 a.s.,

$$\begin{aligned}
& E\left[\{T - e(X)\}^2\{s'(X)\}^2\right] \\
&= E\left[E\left[\{T - e(X)\}^2 \mid X\right]\{s'(X)\}^2\right] \\
&> (\epsilon')^3 E\{s'(X)\}^2 \\
&> 0,
\end{aligned}$$

where the first equality follows by the law of total expectation, the first inequality follows by that  $E\left[\{T - e(X)\}^2 \mid X = x\right] \geq \text{pr}(T = 1 \mid X = x)E\left[\{1 - e(X)\}^2 \mid X = x, T = 1\right] \geq (\epsilon')^3$  for any  $x \in \mathbb{X}$  as  $e(x) \in (\epsilon', 1 - \epsilon')$ , and the last inequality is because  $E\{s'(X)\}^2 > 0$  when  $s'(X)$  is not 0 a.s..

Summarizing the above results, when  $s'(X)$  is not 0 a.s., we have

$$\begin{aligned}
& E\left[Y - m(X) - \{T - e(X)\}\{s'(X) + \tau(X)\}\right]^2 \\
&= E\left[Y - m(X) - \{T - e(X)\}\tau(X)\right]^2 \\
&\quad + E\left[\{T - e(X)\}s'(X)\right]^2 \\
&> E\left[Y - m(X) - \{T - e(X)\}\tau(X)\right]^2.
\end{aligned}$$

That is, (S74) is solved if and only if  $s'(X) = 0$  a.s., which is equivalent to that (S69) is solved if and only if  $h'(x)$  satisfies that  $h'(X) = \tau(X)$  a.s.. Thus (S73) is verified as desired. Combining (S72) and (S73),

we have

$$\tilde{\mathcal{S}}^{\natural} = \{h \mid h(X, 1) = \tau(X, 1) \text{ a.s., and } h(X, 0) = 0 \text{ a.s.}\}.$$

Now we aim at showing that, under the positivity assumption,

$$\{h \mid h(X, 1) = \tau(X, 1) \text{ a.s., and } h(X, 0) = 0 \text{ a.s.}\} = \{h \mid h(X, T) = \tau(X, T) \text{ a.s.}\}, \quad (\text{S76})$$

and thus show (S70) and finish the proof. First suppose  $h \in \{h \mid h(X, 1) = \tau(X, 1) \text{ a.s., and } h(X, 0) = 0 \text{ a.s.}\}$ . Then we have two subsets of  $\mathbb{X}$ ,  $\mathcal{X}_1, \mathcal{X}_2 \subseteq \mathbb{X}$  such that  $h(x, 1) = \tau(x, 1)$  when  $x \in \mathcal{X}_1$ ,  $h(x, 0) = 0$  when  $x \in \mathcal{X}_0$ , and  $\text{pr}(X \in \mathcal{X}_1) = \text{pr}(X \in \mathcal{X}_2) = 1$ . Thus we have when  $(x, t) \in \mathcal{X}_1 \cap \mathcal{X}_2 \times \{0, 1\}$ ,

$$h(x, t) = \tau(x, t).$$

On the other hand, since  $\text{pr}[(X, T) \in \mathcal{X}_1 \cap \mathcal{X}_2 \times \{0, 1\}] = \text{pr}(X \in \mathcal{X}_1 \cap \mathcal{X}_2) = 1$ , we have  $h(X, T) = \tau(X, T)$  a.s., which implies

$$\{h \mid h(X, 1) = \tau(X, 1) \text{ a.s., and } h(X, 0) = 0 \text{ a.s.}\} \subseteq \{h \mid h(X, T) = \tau(X, T) \text{ a.s.}\}. \quad (\text{S77})$$

Second, suppose  $h \in \{h \mid h(X, T) = \tau(X, T) \text{ a.s.}\}$ . Then there exists some  $\Omega_1 \in \mathbb{X} \times \mathbb{T}$  such that  $\text{pr}\{(X, T) \in \Omega_1\} = 1$ , and when  $(x, t) \in \Omega_1$  one has  $h(x, t) = \tau(x, t)$  and  $h(x, t) \neq \tau(x, t)$  otherwise. We now define two marginal sets,

$$\mathcal{X}_3^{(0)} = \{x \mid (x, 0) \in \Omega_1\}, \text{ and } \mathcal{X}_3^{(1)} = \{x \mid (x, 1) \in \Omega_1\}.$$

Now we prove  $\text{pr}(X \in \mathcal{X}_3^{(0)}) = \text{pr}(X \in \mathcal{X}_3^{(1)}) = 1$  by contradiction. Assume  $\text{pr}(X \in \mathcal{X}_3^{(0)}) < 1$ . We have

$$\begin{aligned} \text{pr}[(X, T) \in (\mathbb{X} \setminus \mathcal{X}_3^{(0)}) \times \{0\}] &= \text{pr}(X \in \mathbb{X} \setminus \mathcal{X}_3^{(0)}) \text{pr}(T = 0 \mid \text{given } X \in \mathbb{X} \setminus \mathcal{X}_3^{(0)}) \\ &\geq \{1 - \text{pr}(X \in \mathcal{X}_3^{(0)})\} \cdot \epsilon' \\ &> 0. \end{aligned} \quad (\text{S78})$$

By definition, we know  $(\mathbb{X} \setminus \mathcal{X}_3^{(0)}) \times \{0\} \cap \Omega_1 = \emptyset$ . Thus (S78) implies that with probability larger than 0, we have  $(X, T) \in (\mathbb{X} \times \mathbb{T}) \setminus \Omega_1$ , which is in conflict with  $\text{pr}\{(X, T) \in \Omega_1\} = 1$ . So we conclude  $\text{pr}(X \in \mathcal{X}_3^{(0)}) = 1$ . Recall that when  $x \in \mathcal{X}_3^{(0)}$ , we have  $(x, 0) \in \Omega_1$  and thus  $h(x, 0) = \tau(x, 0) = 0$ . We then have

$$h(X, 0) = 0 \text{ a.s.}$$

With the same argument, we can show  $\text{pr}(X \in \mathcal{X}_3^{(1)}) = 1$  and thus  $h(X, 1) = \tau(X, 1)$  a.s.. So we have  $h \in \{h \mid h(X, 1) = \tau(X, 1) \text{ a.s., and } h(X, 0) = 0 \text{ a.s.}\}$  and thus

$$\{h \mid h(X, T) = \tau(X, T) \text{ a.s.}\} \subseteq \{h \mid h(X, 1) = \tau(X, 1) \text{ a.s., and } h(X, 0) = 0 \text{ a.s.}\}. \quad (\text{S79})$$

Combining (S77) and (S79), we thus show (S76) and (S70) and thereby complete the proof.  $\square$

### S5.5. Proof of Theorem ??

With a basic decomposition, one has

$$\begin{aligned} L_c(h) &= E[\tau(X, T) - E\{\tau(X, T) \mid X\} - [h(X, T) - E\{h(X, T) \mid X\}]]^2 \\ &\quad + E[Y - m(X) - [\tau(X, T) - E\{\tau(X, T) \mid X\}]]^2 \\ &\quad + 2E[[\tau(X, T) - E\{\tau(X, T) \mid X\} - [h(X, T) - E\{h(X, T) \mid X\}]] [Y - m(X) - [\tau(X, T) - E\{\tau(X, T) \mid X\}]]]. \end{aligned} \quad (\text{S80})$$

Under Assumptions ?? and ?? and by the law of total expectation, one has

$$\begin{aligned} E\{Y - m(X) \mid X, T\} &= E(Y \mid X, T) - E(Y \mid X, T = 0) - \{E(Y \mid X) - E(Y \mid X, T = 0)\} \\ &= \tau(X, T) - [E\{E(Y \mid X, T) \mid X\} - E(Y \mid X, T = 0)] \\ &= \tau(X, T) - E\{E(Y \mid X, T) - E(Y \mid X, T = 0) \mid X\} \\ &= \tau(X, T) - E\{\tau(X, T) \mid X\}, \end{aligned}$$

and therefore,

$$\begin{aligned} &E\left[\left[\tau(X, T) - E\{\tau(X, T) \mid X\} - [h(X, T) - E\{h(X, T) \mid X\}]\right][Y - m(X) - [\tau(X, T) - E\{\tau(X, T) \mid X\}]]\right] \\ &= E\left[\left[\tau(X, T) - E\{\tau(X, T) \mid X\} - [h(X, T) - E\{h(X, T) \mid X\}]\right] \right. \\ &\quad \cdot \left. E[Y - m(X) - [\tau(X, T) - E\{\tau(X, T) \mid X\}] \mid X, T]\right] \\ &= E\left[\left[\tau(X, T) - E\{\tau(X, T) \mid X\} - [h(X, T) - E\{h(X, T) \mid X\}]\right] \right. \\ &\quad \cdot \underbrace{\left[E\{Y - m(X) \mid X, T\} - [\tau(X, T) - E\{\tau(X, T) \mid X\}]]}_{=0} \left. \right] \right] \\ &= 0. \end{aligned}$$

Combining (S80) with the above display, one has

$$\begin{aligned} L_c(h) &= E\left[\tau(X, T) - E\{\tau(X, T) \mid X\} - [h(X, T) - E\{h(X, T) \mid X\}]\right]^2 \\ &\quad + E\left[Y - m(X) - [\tau(X, T) - E\{\tau(X, T) \mid X\}]\right]^2. \end{aligned}$$

For simplicity, we define an operator  $\Pi(\cdot)$  for any  $h \in \mathcal{L}_{\mathcal{P}}^2(X, T)$  such that

$$\Pi(h)(x, t) = h(x, t) - E\{h(X, T) \mid X = x\}.$$

Therefore, we have,

$$\begin{aligned} L_{c, \ell_2}(h \mid \rho) &= L_c(h) + \rho \|h\|_{\mathcal{L}_{\mathcal{P}}^2}^2 \\ &= E\left[\tau(X, T) - E\{\tau(X, T) \mid X\} - [h(X, T) - E\{h(X, T) \mid X\}]\right]^2 \\ &\quad + E\left[Y - m(X) - [\tau(X, T) - E\{\tau(X, T) \mid X\}]\right]^2 \\ &\quad + \rho \|h\|_{\mathcal{L}_{\mathcal{P}}^2}^2 \\ &= E\left[\Pi(h)(X, T) - [\tau(X, T) - E\{\tau(X, T) \mid X\}]\right]^2 \\ &\quad + \rho \|h\|_{\mathcal{L}_{\mathcal{P}}^2}^2 \\ &\quad + E\left[Y - m(X) - [\tau(X, T) - E\{\tau(X, T) \mid X\}]\right]^2, \end{aligned}$$

595 which implies that  $\arg \min_{h \in \mathcal{L}_{\mathcal{P}}^2(X, T)} L_{c, \ell_2}(h \mid \rho)$  is equivalent to

$$\begin{aligned} &\arg \min_{h \in \mathcal{L}_{\mathcal{P}}^2(X, T)} E\left[\Pi(h)(X, T) - [\tau(X, T) - E\{\tau(X, T) \mid X\}]\right]^2 + \rho \|h\|_{\mathcal{L}_{\mathcal{P}}^2}^2 \\ &= \arg \min_{h \in \mathcal{L}_{\mathcal{P}}^2(X, T)} \mathcal{F}(h), \end{aligned} \tag{S81}$$

where we define  $\mathcal{F}(h) = E\left[\Pi(h)(X, T) - \tilde{\tau}(X, T)\right]^2 + \rho E\{h(X, T)\}^2$  and  $\tilde{\tau}(x, t) = \tau(x, t) - E\{\tau(X, T) \mid X = x\}$ .

600 Next, we prove  $L_{c, \ell_2}(h \mid \rho)$  has a unique minimum among  $\mathcal{L}_{\mathcal{P}}^2(X, T)$ . By above derivations, we only need to show the minimum of (S81) is unique. An argument similar to the proof of Lemma 1.1 in Tikhonov et al. (1995) can show that  $\mathcal{F}(h)$  has a unique solution. In particular, we first show  $\Pi(\cdot)$  is a self-adjoint

operator; see, e.g., [Rudin \(1991, §12.11\)](#) for the definition of a self-adjoint operator. For any  $h_1, h_2 \in \mathcal{L}_{\mathcal{P}}^2(X, T)$ , we have

$$\begin{aligned} \langle \Pi(h_1), h_2 \rangle_{\mathcal{L}_{\mathcal{P}}^2(X, T)} &= E \left[ \Pi(h_1)(X, T) h_2(X, T) \right] \\ &= E \left[ [h_1(X, T) - E\{h_1(X, T) \mid X\}] h_2(X, T) \right] \\ &= E \left[ h_1(X, T) h_2(X, T) \right] - E \left[ E\{h_1(X, T) \mid X\} h_2(X, T) \right] \\ &= E \left[ h_1(X, T) h_2(X, T) \right] - E \left[ E\{h_1(X, T) \mid X\} E\{h_2(X, T) \mid X\} \right], \end{aligned}$$

where  $\langle \cdot, \cdot \rangle_{\mathcal{L}_{\mathcal{P}}^2(X, T)}$  denotes the inner product of the Hilbert space  $\mathcal{L}_{\mathcal{P}}^2(X, T)$ , and the last equality follows by the law of total expectation. By symmetry, we can also show

$$\begin{aligned} \langle h_1, \Pi(h_2) \rangle_{\mathcal{L}_{\mathcal{P}}^2(X, T)} &= E \left[ h_1(X, T) h_2(X, T) \right] - E \left[ E\{h_1(X, T) \mid X\} E\{h_2(X, T) \mid X\} \right] \\ &= \langle \Pi(h_1), h_2 \rangle_{\mathcal{L}_{\mathcal{P}}^2(X, T)}, \end{aligned}$$

605 which by definition (e.g., [Rudin, 1991, §12.11](#)), implies that  $\Pi(\cdot)$  is a self-adjoint operator from  $\mathcal{L}_{\mathcal{P}}^2(X, T)$  to  $\mathcal{L}_{\mathcal{P}}^2(X, T)$ , i.e. the adjoint operator of  $\Pi(\cdot)$  is still  $\Pi(\cdot)$ . Then, similar to the proof of Lemma 1.1 in [Tikhonov et al. \(1995\)](#), we can denote the second-order Fréchet derivate of  $\mathcal{F}(h)$  by  $D^2\mathcal{F}(h)$  and have that

$$\begin{aligned} D^2\mathcal{F}(h) &= 2\Pi\{\Pi(h)\} + 2\rho h \\ &= 2\Pi(h) + 2\rho h \\ &= 2h - 2E\{h(X, T) \mid X = \cdot\} + 2\rho h, \end{aligned}$$

where the second equality follows by  $\Pi\{\Pi(\cdot)\} = \Pi(\cdot)$  after checking the definition. We now have

$$\begin{aligned} &\langle D^2\mathcal{F}(h), h \rangle_{\mathcal{L}_{\mathcal{P}}^2(X, T)} \\ &= 2 \left[ E\{h(X, T)\}^2 - E[h(X, T)E\{h(X, T) \mid X\}] \right] + 2\rho E\{h(X, T)\}^2 \\ &= 2 \left[ E\{h(X, T)\}^2 - E[E\{h(X, T) \mid X\}]^2 \right] + 2\rho E\{h(X, T)\}^2 \tag{S82} \\ &\geq 2\rho E\{h(X, T)\}^2 \\ &> 0, \end{aligned}$$

where the first equality follows by the law of expectation, the first inequality follows by  $E[E\{h(X, T) \mid X\}]^2 \leq E\{h(X, T)\}^2$  due to Cauchy-Schwarz inequality. (S82) implies that  $\mathcal{F}(h)$  is a strictly convex functional, and thus  $\mathcal{F}(h)$  has a unique minimum among  $\mathcal{L}_{\mathcal{P}}^2(X, T)$ ; see, e.g., [Zeidler \(2013\)](#). Thus (??) has a unique solution, namely,  $\tau_\rho$  in  $\mathcal{L}_{\mathcal{P}}^2(X, T)$ .

Now, we show that when  $\rho \rightarrow 0$ , one has  $\|\tau_\rho - \tilde{\tau}\|_{\mathcal{L}_{\mathcal{P}}^2} \rightarrow 0$ . Note  $\tilde{\tau} \in \mathcal{L}_{\mathcal{P}}^2(X, T)$  as both  $\tau$  and  $E\{\tau(X, T) \mid X = \cdot\}$  have bounded  $\mathcal{L}_{\mathcal{P}}^2$  norms. In particular,  $\tau \in \mathcal{L}_{\mathcal{P}}^2(X, T)$  by definition and, 615

$$\begin{aligned} E[E\{\tau(X, T) \mid X\}^2] &\leq E[E\{\tau^2(X, T) \mid X\}] \\ &= E[\tau^2(X, T)] \\ &< +\infty, \end{aligned}$$

by Cauchy-Schwarz inequality. Since  $\tau_\rho(X, T)$  minimizes  $\mathcal{F}(h)$ , we have

$$\begin{aligned} &\|\Pi(\tau_\rho) - [\tau(x, t) - E\{\tau(X, T) \mid X = \cdot\}]\|_{\mathcal{L}_{\mathcal{P}}^2}^2 + \rho \|\tau_\rho\|_{\mathcal{L}_{\mathcal{P}}^2}^2 \\ &\leq \|\Pi(\tilde{\tau}) - [\tau(x, t) - E\{\tau(X, T) \mid X = \cdot\}]\|_{\mathcal{L}_{\mathcal{P}}^2}^2 + \rho \|\tilde{\tau}\|_{\mathcal{L}_{\mathcal{P}}^2}^2 \tag{S83} \\ &= \rho \|\tilde{\tau}\|_{\mathcal{L}_{\mathcal{P}}^2}^2, \end{aligned}$$

by noticing that  $\Pi(\tilde{\tau})(x, t) = \tau(x, t) - E\{\tau(X, T) \mid X = x\} - [E\{\tau(X, T) \mid X = x\} - E\{\tau(X, T) \mid X = x\}] = \tau(x, t) - E\{\tau(X, T) \mid X = x\}$ . Because  $\|\Pi(\tilde{\tau}) - [\tau(x, t) - E\{\tau(X, T) \mid X = \cdot\}]\|_{\mathcal{L}_P^2}^2 > 0$ , we have

$$\rho \|\tau_\rho\|_{\mathcal{L}_P^2}^2 \leq \rho \|\tilde{\tau}\|_{\mathcal{L}_P^2}^2,$$

which is equivalent to

$$\begin{aligned} & E\{\tau_\rho(X, T)\}^2 \\ & \leq E\{\tau_\rho(X, T)\}^2 + E\{\tilde{\tau}(X, T) - \tau_\rho(X, T)\}^2 + 2E[\{\tilde{\tau}(X, T) - \tau_\rho(X, T)\}\tau_\rho(X, T)] \\ & = E\{\tau_\rho(X, T)\}^2 + E\{\tilde{\tau}(X, T) - \tau_\rho(X, T)\}^2 + 2E[\{\tilde{\tau}(X, T) - \tau_\rho(X, T)\}\{\tau_\rho(X, T) - \tilde{\tau}(X, T) + \tilde{\tau}(X, T)\}] \\ & = E\{\tau_\rho(X, T)\}^2 - E\{\tilde{\tau}(X, T) - \tau_\rho(X, T)\}^2 + 2E[\{\tilde{\tau}(X, T) - \tau_\rho(X, T)\}\tilde{\tau}(X, T)]. \end{aligned}$$

With simple algebra, we then deduce

$$\begin{aligned} E\{\tilde{\tau}(X, T) - \tau_\rho(X, T)\}^2 & \leq 2E[\{\tilde{\tau}(X, T) - \tau_\rho(X, T)\}\tilde{\tau}(X, T)] \\ & = 2E[\{\tilde{\tau}(X, T) - \tau_\rho(X, T) + E\{\tau_\rho(X, T) \mid X\}\}\tilde{\tau}(X, T)] \\ & \leq 2\|\tilde{\tau}\|_{\mathcal{L}_P^2} \left[ E[\{\tilde{\tau}(X, T) - \tau_\rho(X, T) + E\{\tau_\rho(X, T) \mid X\}\}^2] \right]^{1/2} \quad (\text{S84}) \\ & = 2\|\tilde{\tau}\|_{\mathcal{L}_P^2} \|\Pi(\tau_\rho) - [\tau(x, t) - E\{\tau(X, T) \mid X = \cdot\}]\|_{\mathcal{L}_P^2}, \end{aligned}$$

where the first equality follows by the law of total expectation such that

$$\begin{aligned} E[E\{\tau_\rho(X, T) \mid X\}\tilde{\tau}(X, T)] & = E\left[E\{\tau_\rho(X, T) \mid X\} \underbrace{E[\tau(X, T) - E\{\tau(X, T) \mid X\} \mid X]}_{=0}\right] \\ & = 0, \end{aligned}$$

and the second inequality follows by Cauchy-Schwarz inequality. Finally, by  $\|\tilde{\tau}\|_{\mathcal{L}_P^2} \lesssim 1$  as we alluded earlier and (S83), we conclude

$$\|\Pi(\tau_\rho) - [\tau(x, t) - E\{\tau(X, T) \mid X = \cdot\}]\|_{\mathcal{L}_P^2}^2 \leq \rho \|\tilde{\tau}\|_{\mathcal{L}_P^2}^2 = \mathcal{O}(\rho).$$

620 Combining with (S84) yields

$$\|\tau_\rho - \tilde{\tau}\|_{\mathcal{L}_P^2} = \mathcal{O}(\rho^{1/4}) = o(1),$$

when  $\rho \rightarrow 0$ , and thus  $\tau_\rho \rightarrow \tilde{\tau}$  under the  $\mathcal{L}_P^2$  norm.

Finally we show (??). Under Assumptions ?? and ??, one has  $\tau(x, t) = E(Y \mid X = x, T = t) - E(Y \mid X = x, T = 0)$  and thus,

$$\begin{aligned} \tilde{\tau}(x, t) & = E(Y \mid X = x, T = t) - E(Y \mid X = x, T = 0) \\ & \quad - E\{E(Y \mid X = x, T) - E(Y \mid X = x, T = 0) \mid X = x\} \\ & = E(Y \mid X = x, T = t) - E(Y \mid X = x). \end{aligned}$$

Then we have

$$\begin{aligned} & \tilde{\tau}(x, t) - \tilde{\tau}(x, 0) \\ & = E(Y \mid X = x, T = t) - E(Y \mid X = x) - E(Y \mid X = x, T = 0) + E(Y \mid X = x) \\ & = E(Y \mid X = x, T = t) - E(Y \mid X = x, T = 0) \\ & = \tau(x, t). \end{aligned}$$

S5.6. *Proof of Proposition ??*

First we note that when estimating  $\hat{\Gamma}(x)$  through  $\hat{\Gamma}(x) = E_{\hat{\omega}}\{\Psi(X, T) \mid X = x\}$ , we have

$$\begin{aligned}\hat{\Gamma}(x) &= E_{\hat{\omega}}\{\psi(T) \otimes \Psi(X) \mid X = x\} \\ &= E_{\hat{\omega}}\{\psi(T) \mid X = x\} \otimes \Psi(x),\end{aligned}$$

where we denote  $\Psi(x) = \psi(x^{(1)}) \otimes \cdots \otimes \psi(x^{(d)})$ . Correspondingly,  $\Gamma(x) = E_{\varpi}\{\psi(T) \mid X = x\} \otimes \Psi(x)$  and thus

$$\begin{aligned}\hat{\Gamma}(x) - \Gamma(x) &= [E_{\hat{\omega}}\{\psi(T) \mid X = x\} - E_{\varpi}\{\psi(T) \mid X = x\}] \otimes \Psi(x) \\ &= \left[ \int_{\mathbb{T}} \psi(t) \{\hat{\omega}(t \mid x) - \varpi(t \mid x)\} dt \right] \otimes \Psi(x) \\ &= \int_{\mathbb{T}} [\psi(t) \otimes \Psi(x)] \{\hat{\omega}(t \mid x) - \varpi(t \mid x)\} dt \\ &= \int_{\mathbb{T}} \Psi(x, t) \{\hat{\omega}(t \mid x) - \varpi(t \mid x)\} dt.\end{aligned}$$

On the other hand,

630

$$\begin{aligned}\sup_{x \in \mathbb{X}} \int_{\mathbb{T}} \{\hat{\omega}(t \mid x) - \varpi(t \mid x)\}^2 dt &= \sup_{x \in \mathbb{X}} \|\hat{\omega}(\cdot \mid x) - \varpi(\cdot \mid x)\|_{\mathcal{L}^2}^2 \\ &= o_P(r_{\varpi}^2).\end{aligned}$$

First we have,

$$\begin{aligned}&\|P[\{\hat{\Gamma}(X) - \Gamma(X)\}\{\hat{\Gamma}(X) - \Gamma(X)\}^T]\|_2 \\ &= \sup_{\|\ell\|=1} P[\ell^T \{\hat{\Gamma}(X) - \Gamma(X)\}]^2 \\ &= \sup_{\|\ell\|=1} P\left[\int_{\mathbb{T}} \ell^T \Psi(X, t) \{\hat{\omega}(t \mid X) - \varpi(t \mid X)\} dt\right]^2 \\ &\leq \sup_{\|\ell\|=1} P\left[\int_{\mathbb{T}} \{\ell^T \Psi(X, t)\}^2 dt \int_{\mathbb{T}} \{\hat{\omega}(t \mid X) - \varpi(t \mid X)\}^2 dt\right] \\ &\leq \sup_{x \in \mathbb{X}} \|\hat{\omega}(\cdot \mid x) - \varpi(\cdot \mid x)\|_{\mathcal{L}^2}^2 \cdot \sup_{\|\ell\|=1} P\left[\int_{\mathbb{T}} \{\ell^T \Psi(X, t)\}^2 dt\right] \\ &\leq \sup_{x \in \mathbb{X}} \|\hat{\omega}(\cdot \mid x) - \varpi(\cdot \mid x)\|_{\mathcal{L}^2}^2 \cdot \sup_{\|\ell\|=1} \left[\int_{\mathbb{X} \times \mathbb{T}} \{\ell^T \Psi(x, t)\}^2 dx dt\right] \cdot C_f \quad (\text{Assumption S4}) \\ &\lesssim \sup_{x \in \mathbb{X}} \|\hat{\omega}(\cdot \mid x) - \varpi(\cdot \mid x)\|_{\mathcal{L}^2}^2 \quad (\text{Lemma S3}) \\ &= o_P(r_{\varpi}^2),\end{aligned}$$

which directly yields  $\|P[\{\hat{\Gamma}(X) - \Gamma(X)\}\{\hat{\Gamma}(X) - \Gamma(X)\}^T]\|_2^{1/2} = o_P(r_{\varpi})$ . Second, by the property of Kronecker product (Schacke, 2004), we have

$$\begin{aligned}\|\hat{\Gamma} - \Gamma\|_{\mathbb{X}}^2 &= \sup_{x \in \mathbb{X}} \left\| \int_{\mathbb{T}} \Psi(x, t) \{\hat{\omega}(t \mid x) - \varpi(t \mid x)\} dt \right\|^2 \\ &\leq \|\Psi\|_{\mathbb{X} \times \mathbb{T}}^2 \cdot \sup_{x \in \mathbb{X}} \int_{\mathbb{T}} \{\hat{\omega}(t \mid x) - \varpi(t \mid x)\}^2 dt \\ &= o_P(K r_{\varpi}^2),\end{aligned}$$

where the last equality is because that by Lemma S3, we have  $\|\Psi\|_{\mathbb{X} \times \mathbb{T}}^2 \lesssim K$ . We thus show  $\|\hat{\Gamma} - \Gamma\|_{\mathbb{X}}/\sqrt{K} = o_P(r_{\varpi})$ .  $\square$

635

## S5.7. Proof of Theorem ??

For fixed  $(x_0, t_0) \in \mathbb{X} \times \mathbb{T}$ , we decompose

$$\begin{aligned}
 & |\hat{\tau}(x_0, t_0) - \tau(x_0, t_0)| \\
 &= \left| \left\{ \Psi(x_0, t_0) - \Psi(x_0, 0) \right\}^\top (\hat{\phi} - \phi^*) + \left\{ \Psi(x_0, t_0) - \Psi(x_0, 0) \right\}^\top \phi^* - \tau(x_0, t_0) \right| \\
 &\leq \left| \left\{ \Psi(x_0, t_0) - \Psi(x_0, 0) \right\}^\top (\hat{\phi} - \phi^*) \right| + \left| \left\{ \Psi(x_0, t_0) - \Psi(x_0, 0) \right\}^\top \phi^* - \tau(x_0, t_0) \right| \\
 &= T_1 + T_2.
 \end{aligned} \tag{S85}$$

The second term is the bias term, which can be bounded by Proposition S1. In particular, recalling Theorem ?? that  $\tau(x_0, t_0) = \tilde{\tau}(x_0, t_0) - \tilde{\tau}(x_0, 0)$ , we have

$$\begin{aligned}
 T_2 &\leq \left| \Psi^\top(x_0, t_0) \phi^* - \tilde{\tau}(x_0, t_0) \right| + \left| \Psi^\top(x_0, 0) \phi^* - \tilde{\tau}(x_0, 0) \right| \\
 &\leq 2 \|(\phi^*)^\top \Psi - \tilde{\tau}\|_{\mathbb{X} \times \mathbb{T}} \\
 &\lesssim K^{-p/(d+1)}
 \end{aligned} \tag{S86}$$

640 by Proposition S1.

Next we bound the term  $T_1$ . Since  $UU^\top + U_\perp U_\perp^\top = I$ , we observe that

$$\begin{aligned}
 T_1 &= \left\{ \Psi(x_0, t_0) - \Psi(x_0, 0) \right\}^\top (\hat{\phi} - \phi^*) \\
 &= \left\{ \Psi(x_0, t_0) - \Psi(x_0, 0) \right\}^\top (UU^\top + U_\perp U_\perp^\top) (\hat{\phi} - \phi^*) \\
 &= \left\{ \Psi^\top(x_0, t_0) U - \Psi^\top(x_0, 0) U \right\} U^\top (\hat{\phi} - \phi^*) + \left\{ \Psi^\top(x_0, t_0) U_\perp - \Psi^\top(x_0, 0) U_\perp \right\} U_\perp^\top (\hat{\phi} - \phi^*) \\
 &= \left\{ \Psi^\top(x_0, t_0) U - \Psi^\top(x_0, 0) U \right\} U^\top (\hat{\phi} - \phi^*) \\
 &= v_n^\top U^\top (\hat{\phi} - \phi^*),
 \end{aligned} \tag{S87}$$

where we denote  $v_n = U^\top \Psi(x_0, t_0) - U^\top \Psi(x_0, 0)$  for simplicity, and thus

$$\|v_n\| \leq \|U\|_2 \{ \|\Psi(x_0, t_0)\| + \|\Psi(x_0, 0)\| \} \lesssim \sqrt{K}, \tag{S88}$$

by Lemma S3. The second equality of (S87) is because that by Lemma S4,  $\Psi^\top(x, t) U_\perp$  are functions free of  $t$  and thus  $\Psi^\top(x_0, t) U_\perp$  is the same for all  $t \in \mathbb{T}$ , which implies that

$$\begin{aligned}
 \Psi^\top(x_0, t_0) U_\perp - \Psi^\top(x_0, 0) U_\perp &= \Psi^\top(x_0, 0) U_\perp - \Psi^\top(x_0, 0) U_\perp \\
 &= 0.
 \end{aligned}$$

645 Now we focus on bounding  $|v_n^\top U^\top (\hat{\phi} - \phi^*)|$ . Recall the form of  $\hat{\phi}$  in (??) and the simplifying setting of training nuisance functions by a single separate dataset (§S5.1). We then have

$$\begin{aligned}
 T_1 &= v_n^\top U^\top (\hat{\phi} - \phi^*) \\
 &= v_n^\top U^\top \hat{G}_n^{-1} \left[ P_n \left[ \{Y - \hat{m}(X)\} \{\Psi(X, T) - \hat{\Gamma}(X)\} \right] - \hat{G}_n \phi^* \right] \\
 &= v_n^\top U^\top \hat{G}_n^{-1} P_n \left[ \left[ Y - \hat{m}(X) - \{\Psi(X, T) - \hat{\Gamma}(X)\}^\top \phi^* \right] \{\Psi(X, T) - \hat{\Gamma}(X)\} \right] \\
 &\quad + v_n^\top U^\top \hat{G}_n^{-1} (-\rho \hat{Q}_n \phi^*) \\
 &= v_n^\top U^\top \hat{G}_n^{-1} \Delta_1 + v_n^\top U^\top \hat{G}_n^{-1} \Delta_2.
 \end{aligned} \tag{S89}$$

In the following, we bound  $|v_n^T U^T \hat{G}_n^{-1} \Delta_1|$  and  $|v_n^T U^T \hat{G}_n^{-1} \Delta_2|$ , respectively. By Lemma S8, we know wpa1,  $\hat{G}_n$  and  $G_n$  are full-rank and their inverse have the singular value decomposition,

$$\begin{aligned}\hat{G}_n^{-1} &= (\hat{U} \ \hat{U}_\perp) \begin{pmatrix} \hat{\Sigma}^{-1} & \\ & \hat{\Sigma}_\perp^{-1} \end{pmatrix} \begin{pmatrix} \hat{U}^T \\ \hat{U}_\perp^T \end{pmatrix}, \\ G_n^{-1} &= (\tilde{U} \ \tilde{U}_\perp) \begin{pmatrix} \tilde{\Sigma}^{-1} & \\ & \tilde{\Sigma}_\perp^{-1} \end{pmatrix} \begin{pmatrix} \tilde{U}^T \\ \tilde{U}_\perp^T \end{pmatrix}.\end{aligned}\tag{S90}$$

Bound of  $|v_n^T U^T \hat{G}_n^{-1} \Delta_1|$  We first bound  $|v_n^T U^T \hat{G}_n^{-1} \Delta_1|$ . With straightforward algebra, we further write the following decomposition of  $\Delta_1$ ,

$$\begin{aligned}\Delta_1 &= P_n \left[ [Y - m(X) - \tau(X, T) + E\{\tau(X, T) \mid X\}] \{\Psi(X, T) - \Gamma(X)\} \right] \\ &\quad + P_n \left[ [\tau(X, T) - E\{\tau(X, T) \mid X\} - \{\Psi(X, T) - \Gamma(X)\}^T \phi^*] \{\Psi(X, T) - \Gamma(X)\} \right] \\ &\quad + P_n \left[ [Y - m(X) - \{\Psi(X, T) - \Gamma(X)\}^T \phi^*] \{\Gamma(X) - \hat{\Gamma}(X)\} \right] \\ &\quad + P_n \left[ [m(X) - \hat{m}(X) - \{\Gamma(X) - \hat{\Gamma}(X)\}^T \phi^*] \{\Psi(X, T) - \Gamma(X)\} \right] \\ &\quad + P_n \left[ [m(X) - \hat{m}(X) - \{\Gamma(X) - \hat{\Gamma}(X)\}^T \phi^*] \{\Gamma(X) - \hat{\Gamma}(X)\} \right] \\ &= \Delta_{1,1} + \Delta_{1,2} + \Delta_{1,3} + \Delta_{1,4} + \Delta_{1,5},\end{aligned}\tag{S91}$$

which further yields the decomposition,

$$v_n^T U^T \hat{G}_n^{-1} \Delta_1 = \sum_{j=1}^5 v_n^T U^T \hat{G}_n^{-1} \Delta_{1,j}.$$

We bound  $|v_n^T U^T \hat{G}_n^{-1} \Delta_1|$  by deriving the bounds of  $|v_n^T U^T \hat{G}_n^{-1} \Delta_{1,1}|$  through  $|v_n^T U^T \hat{G}_n^{-1} \Delta_{1,5}|$ .

- *Bounding  $|v_n^T U^T \hat{G}_n^{-1} \Delta_{1,1}|$ :* Recall  $\mu(x, t) = E(Y \mid X = x, T = t)$ . We first note  $\Delta_{1,1}$  can be further simplified to,

$$\Delta_{1,1} = P_n [\{Y - \mu(X, T)\} \{\Psi(X, T) - \Gamma(X)\}],\tag{S92}$$

as, by definition for any  $i = 1, \dots, n$ ,

$$\begin{aligned}Y_i - m(X_i) - \tau(T_i, X_i) + E\{\tau(X, T) \mid X = X_i\} \\ &= Y_i - E(Y \mid X_i) - \mu(X_i, T_i) + \mu(X_i, 0) + E\{\mu(X, T) - \mu(X, 0) \mid X = X_i\} \\ &= Y_i - E(Y \mid X_i) - \mu(X_i, T_i) + \mu(X_i, 0) + E(Y \mid X_i) - \mu(X_i, 0) \\ &= Y_i - \mu(X_i, T_i).\end{aligned}$$

Again by  $(U \ U_\perp) (U \ U_\perp)^T = I$ , we have

$$\Delta_{1,1} = (U \ U_\perp) \begin{pmatrix} U^T \\ U_\perp^T \end{pmatrix} \Delta_{1,1} = U U^T \Delta_{1,1},\tag{S93}$$

because,

$$\begin{aligned}U_\perp^T \Delta_{1,1} &= P_n \left[ [Y - m(X) - \{\Psi(X, T) - \Gamma(X)\}^T \phi^*] \cdot \{U_\perp^T \Psi(X, T) - U_\perp^T \Gamma(X)\} \right] \\ &= P_n \left[ [Y - m(X) - \{\Psi(X, T) - \Gamma(X)\}^T \phi^*] \cdot 0 \right] \\ &= 0.\end{aligned}\tag{S94}$$



The second equality above is due to that, by Lemma S4,  $U_{\perp}^T \Psi(X, T)$  is a vector of functions free of  $T$  and thus,

$$U_{\perp}^T \Gamma(x) = E[U_{\perp}^T \Psi(X, T) \mid X = x] = U_{\perp}^T \Psi(x, t), \quad (\text{S95})$$

for any  $(x, t) \in \mathbb{X} \times \mathbb{T}$ . Summarizing the results above, we have wpa1,

660

$$\begin{aligned} & v_n^T U^T \hat{G}_n^{-1} \Delta_{1,1} \\ &= v_n^T U^T G_n^{-1} \Delta_{1,1} + v_n^T U^T (\hat{G}_n^{-1} - G_n^{-1}) \Delta_{1,1} \\ &= v_n^T U^T G_n^{-1} \Delta_{1,1} + v_n^T U^T G_n^{-1} (G_n - \hat{G}_n) \hat{G}_n^{-1} \Delta_{1,1} \\ &= v_n^T U^T G_n^{-1} U U^T \Delta_{1,1} + v_n^T U^T G_n^{-1} (G_n - \hat{G}_n) \hat{G}_n^{-1} U U^T \Delta_{1,1} \\ &= v_n^T U^T \tilde{U} \tilde{\Sigma}^{-1} \tilde{U}^T U U^T \Delta_{1,1} + v_n^T U^T \tilde{U}_{\perp} \tilde{\Sigma}_{\perp}^{-1} \tilde{U}_{\perp}^T U U^T \Delta_{1,1} \\ &+ v_n^T U^T \tilde{U} \tilde{\Sigma}^{-1} \tilde{U}^T (G_n - \hat{G}_n) \hat{U} \hat{\Sigma}^{-1} \hat{U}^T U U^T \Delta_{1,1} + v_n^T U^T \tilde{U} \tilde{\Sigma}^{-1} \tilde{U}^T (G_n - \hat{G}_n) \hat{U}_{\perp} \hat{\Sigma}_{\perp}^{-1} \hat{U}_{\perp}^T U U^T \Delta_{1,1} \\ &+ v_n^T U^T \tilde{U}_{\perp} \tilde{\Sigma}_{\perp}^{-1} \tilde{U}_{\perp}^T (G_n - \hat{G}_n) \hat{U} \hat{\Sigma}^{-1} \hat{U}^T U U^T \Delta_{1,1} + v_n^T U^T \tilde{U}_{\perp} \tilde{\Sigma}_{\perp}^{-1} \tilde{U}_{\perp}^T (G_n - \hat{G}_n) \hat{U}_{\perp} \hat{\Sigma}_{\perp}^{-1} \hat{U}_{\perp}^T U U^T \Delta_{1,1} \\ &= \sum_{m=1}^6 \ell_{m,n}^T \Delta_{1,1}, \end{aligned} \quad (\text{S96})$$

where the third equality follows by (S93); the fourth equality follows by (S90); and we define

$$\begin{aligned} \ell_{1,n} &= (v_n^T U^T \tilde{U} \tilde{\Sigma}^{-1} \tilde{U}^T U U^T)^T, \\ \ell_{2,n} &= (v_n^T U^T \tilde{U}_{\perp} \tilde{\Sigma}_{\perp}^{-1} \tilde{U}_{\perp}^T U U^T)^T, \\ \ell_{3,n} &= \{v_n^T U^T \tilde{U} \tilde{\Sigma}^{-1} \tilde{U}^T (G_n - \hat{G}_n) \hat{U} \hat{\Sigma}^{-1} \hat{U}^T U U^T\}^T, \\ \ell_{4,n} &= \{v_n^T U^T \tilde{U} \tilde{\Sigma}^{-1} \tilde{U}^T (G_n - \hat{G}_n) \hat{U}_{\perp} \hat{\Sigma}_{\perp}^{-1} \hat{U}_{\perp}^T U U^T\}^T, \\ \ell_{5,n} &= \{v_n^T U^T \tilde{U}_{\perp} \tilde{\Sigma}_{\perp}^{-1} \tilde{U}_{\perp}^T (G_n - \hat{G}_n) \hat{U} \hat{\Sigma}^{-1} \hat{U}^T U U^T\}^T, \\ \ell_{6,n} &= \{v_n^T U^T \tilde{U}_{\perp} \tilde{\Sigma}_{\perp}^{-1} \tilde{U}_{\perp}^T (G_n - \hat{G}_n) \hat{U}_{\perp} \hat{\Sigma}_{\perp}^{-1} \hat{U}_{\perp}^T U U^T\}^T. \end{aligned}$$

We note  $\ell_{1,n}$  and  $\ell_{2,n}$  depend only on  $n$ , and  $\ell_{3,n}-\ell_{6,n}$  depend on both  $n$  and  $(X_1, T_1), \dots, (X_n, T_n)$  since the  $\hat{G}_n$  is involved. For each  $m = 1, \dots, 6$ , by taking  $\ell_n = \ell_{m,n}/\|\ell_{m,n}\|$  in Lemma S9 (i), we have

$$|\ell_{m,n}^T \Delta_{1,1}| = \mathcal{O}_P(\|\ell_{m,n}\|/\sqrt{n}). \quad (\text{S97})$$

665

We now bound  $\|\ell_{m,n}\|$  for each  $m = 1, \dots, 6$  as  $n \rightarrow +\infty$ , by Lemma S8,

$$\begin{aligned} \|\ell_{1,n}\| &\leq \|v_n\| \|U^T \tilde{U}\|_2 \|\tilde{\Sigma}^{-1}\|_2 \|\tilde{U}^T U U^T\|_2 = \mathcal{O}(\|v_n\| \beta_n^{-1}), \\ \|\ell_{2,n}\| &\leq \|v_n\| \|U^T \tilde{U}_{\perp}\|_2 \|\tilde{\Sigma}_{\perp}^{-1}\|_2 \|\tilde{U}_{\perp}^T U\|_2 \|U^T\|_2 = \mathcal{O}(\|v_n\| \rho \beta_n^{-2}), \\ \|\ell_{3,n}\| &\leq \|v_n\| \|U^T \tilde{U}\|_2 \|\tilde{\Sigma}^{-1}\|_2 \|\tilde{U}^T\|_2 \|G_n - \hat{G}_n\|_2 \|\hat{U}\|_2 \|\hat{\Sigma}^{-1}\|_2 \|\hat{U}^T U U^T\|_2 = \mathcal{O}_P(\|v_n\| \beta_n^{-2} \sqrt{K \log n/n}), \\ \|\ell_{4,n}\| &\leq \|v_n\| \|U^T \tilde{U}\|_2 \|\tilde{\Sigma}^{-1}\|_2 \|\tilde{U}^T\|_2 \|G_n - \hat{G}_n\|_2 \|\hat{U}_{\perp}\|_2 \|\hat{\Sigma}_{\perp}^{-1}\|_2 \|\hat{U}_{\perp}^T U\|_2 \|U^T\|_2 = \mathcal{O}_P(\|v_n\| \beta_n^{-2} \rho^{-1} K \log n/n), \\ \|\ell_{5,n}\| &\leq \|v_n\| \|U^T \tilde{U}_{\perp}\|_2 \|\tilde{\Sigma}_{\perp}^{-1}\|_2 \|\tilde{U}_{\perp}^T\|_2 \|G_n - \hat{G}_n\|_2 \|\hat{U}\|_2 \|\hat{\Sigma}^{-1}\|_2 \|\hat{U}^T U U^T\|_2 = \mathcal{O}_P(\|v_n\| \beta_n^{-2} \sqrt{K \log n/n}), \\ \|\ell_{6,n}\| &\leq \|v_n\| \|U^T \tilde{U}_{\perp}\|_2 \|\tilde{\Sigma}_{\perp}^{-1}\|_2 \|\tilde{U}_{\perp}^T\|_2 \|G_n - \hat{G}_n\|_2 \|\hat{U}_{\perp}\|_2 \|\hat{\Sigma}_{\perp}^{-1}\|_2 \|\hat{U}_{\perp}^T U\|_2 \|U^T\|_2 = \mathcal{O}_P(\|v_n\| \beta_n^{-2} \rho^{-1} K \log n/n). \end{aligned} \quad (\text{S98})$$

Combining (S96), (S97), and (S98), we conclude

$$\begin{aligned} |v_n^T U^T \hat{G}_n^{-1} \Delta_{1,1}| &= \mathcal{O}_P\left\{\|v_n\| n^{-1/2} \beta_n^{-1} (1 + \rho \beta_n^{-1} + \beta_n^{-1} \sqrt{K \log n/n} + \beta_n^{-1} \rho^{-1} K \log n/n)\right\} \\ &= \mathcal{O}_P\left\{\|v_n\| n^{-1/2} \beta_n^{-1} (1 + \beta_n^{-1} \rho^{-1} K \log n/n)\right\}, \end{aligned}$$

since  $\beta_n \succ \sqrt{K \log n/n} \succ \rho$  implies that  $1 \succ \rho \beta_n^{-1}$  and  $\beta_n^{-1} \rho^{-1} K \log n/n \succ \beta_n^{-1} \sqrt{K \log n/n}$ .

- *Bounding  $|v_n^T U^T \hat{G}_n^{-1} \Delta_{1,2}|$* : With the same derivations as (S93)–(S95), we have  $\Delta_{1,2} = U U^T \Delta_{1,2}$ . and thus similar to (S96),

$$v_n^T U^T \hat{G}_n^{-1} \Delta_{1,2} = \sum_{m=1}^6 \ell_{m,n}^T \Delta_{1,2}.$$

670 For  $m = 1, 2$ , we can apply Lemma S9 (ii) and bound

$$|\ell_{m,n}^T \Delta_{1,2}| = \|\ell_{m,n}\| |(\ell_{m,n}/\|\ell_{m,n}\|)^T \Delta_{1,2}| = \mathcal{O}_P(\|\ell_{m,n}\| K^{-p/(d+1)}),$$

since  $\ell_{1,n}/\|\ell_{1,n}\|$  and  $\ell_{2,n}/\|\ell_{2,n}\|$  depend only on  $n$ . For  $m = 3, \dots, 6$ , we have

$$|\ell_{m,n}^T \Delta_{1,2}| \leq \|\ell_{m,n}\| \|\Delta_{1,2}\| = \mathcal{O}_P(\|\ell_{m,n}\| K^{-p/(d+1)}).$$

Combining the above results with (S97), we conclude

$$|v_n^T U^T \hat{G}_n^{-1} \Delta_{1,2}| = \mathcal{O}_P \left\{ \|v_n\| \beta_n^{-1} n^{-1/2} K^{-p/(d+1)} (1 + \beta_n^{-1} \rho^{-1} K \log n/n) \right\}.$$

- *Bounding  $|v_n^T U^T \hat{G}_n^{-1} \Delta_{1,3}|$* : By Lemma S4 (iv), we have  $U_\perp^T \{\Gamma(x) - \hat{\Gamma}(x)\} = 0$  for any  $x \in \mathbb{X}$ , which implies

$$\begin{aligned} U_\perp^T \Delta_{1,3} &= P_n \left[ [Y - m(X) - \{\Psi(X, T) - \Gamma(X)\}^T \phi^*] \{U_\perp^T \Gamma(X) - U_\perp^T \hat{\Gamma}(X)\} \right] \\ &= 0. \end{aligned} \quad (\text{S99})$$

675 Then with similar derivations as (S93)–(S95), we have  $\Delta_{1,3} = U U^T \Delta_{1,3}$ . And thus similar to (S96),

$$v_n^T U^T \hat{G}_n^{-1} \Delta_{1,3} = \sum_{m=1}^6 \ell_{m,n}^T \Delta_{1,3}.$$

For  $m = 1, 2$ , we can apply Lemma S9 (iii) and bound

$$|\ell_{m,n}^T \Delta_{1,3}| = \|\ell_{m,n}\| |(\ell_{m,n}/\|\ell_{m,n}\|)^T \Delta_{1,3}| = o_P(\|\ell_{m,n}\| r_\gamma / \sqrt{n}),$$

since  $\ell_{1,n}/\|\ell_{1,n}\|$  and  $\ell_{2,n}/\|\ell_{2,n}\|$  depend only on  $n$ . For  $m = 3, \dots, 6$ , we have

$$|\ell_{m,n}^T \Delta_{1,3}| \leq \|\ell_{m,n}\| \|\Delta_{1,3}\| = o_P(\|\ell_{m,n}\| r'_\gamma \sqrt{K/n}).$$

Combining the above results with (S97), we conclude

$$|v_n^T U^T \hat{G}_n^{-1} \Delta_{1,3}| = o_P \left( \|v_n\| \beta_n^{-1} n^{-1/2} r_\gamma \right) + o_P \left\{ \|v_n\| \beta_n^{-2} (\log n) K^{3/2} n^{-3/2} r'_\gamma \rho^{-1} \right\}.$$

- *Bounding  $|v_n^T U^T \hat{G}_n^{-1} \Delta_{1,4}|$* : With the same derivations as (S93)–(S96), we have

$$v_n^T U^T \hat{G}_n^{-1} \Delta_{1,4} = \sum_{m=1}^6 \ell_{m,n}^T \Delta_{1,4}.$$

For  $m = 1, 2$ , we can apply Lemma S9 (iv) and bound

$$|\ell_{m,n}^T \Delta_{1,4}| = \|\ell_{m,n}\| |(\ell_{m,n}/\|\ell_{m,n}\|)^T \Delta_{1,4}| = o_P(\|\ell_{m,n}\| / \sqrt{n}),$$

since  $\ell_{1,n}/\|\ell_{1,n}\|$  and  $\ell_{2,n}/\|\ell_{2,n}\|$  depend only on  $n$ . For  $m = 3, \dots, 6$ , we have

$$|\ell_{m,n}^T \Delta_{1,4}| \leq \|\ell_{m,n}\| \|\Delta_{1,4}\| = o_P(r_m \|\ell_{m,n}\| \sqrt{K/n} + r_\gamma \|\ell_{m,n}\| \sqrt{K/n}).$$

Combining the above results with (S97), we conclude

$$|v_n^T U^T \hat{G}_n^{-1} \Delta_{1,4}| = o_P \left( \|v_n\| n^{-1/2} \beta_n^{-1} \right) + o_P \left\{ \|v_n\| \beta_n^{-2} (\log n) K^{3/2} n^{-3/2} \rho^{-1} (r_m + r_\gamma) \right\}.$$

- **Bounding  $|v_n^T U^T \hat{G}_n^{-1} \Delta_{1,5}|$ :** Similar to (S99), we have  $U_\perp^T \Delta_{1,5} = 0$  and thus with the same derivations as (S93)–(S96), we have

$$v_n^T U^T \hat{G}_n^{-1} \Delta_{1,5} = \sum_{m=1}^6 \ell_{m,n}^T \Delta_{1,5}.$$

For  $m = 1, 2$ , we can apply Lemma S9 (v) and bound

685

$$|\ell_{m,n}^T \Delta_{1,5}| = \|\ell_{m,n}\| |(\ell_{m,n}/\|\ell_{m,n}\|)^T \Delta_{1,5}| = o_P(r_\gamma \|\ell_{m,n}\|/\sqrt{n} + \|\ell_{m,n}\| r_m r_\gamma + \|\ell_{m,n}\| r_\gamma^2),$$

since  $\ell_{1,n}/\|\ell_{1,n}\|$  and  $\ell_{2,n}/\|\ell_{2,n}\|$  depend only on  $n$ . For  $m = 3, \dots, 6$ , we have

$$|\ell_{m,n}^T \Delta_{1,5}| \leq \|\ell_{m,n}\| \|\Delta_{1,5}\| = o_P(\|\ell_{m,n}\| r_m r_\gamma + \|\ell_{m,n}\| r_\gamma^2 + \|\ell_{m,n}\| r'_\gamma r_m \sqrt{K/n} + \|\ell_{m,n}\| r'_\gamma r_\gamma \sqrt{K/n}).$$

Combining the above results with (S97), we conclude

$$\begin{aligned} & |v_n^T U^T \hat{G}_n^{-1} \Delta_{1,5}| \\ &= o_P\left\{\|v_n\| \beta_n^{-1} (r_\gamma/\sqrt{n} + r_m r_\gamma + r_\gamma^2)\right\} \\ &+ o_P\left\{\|v_n\| \beta_n^{-2} (\log n) K n^{-1} \rho^{-1} (r_m r_\gamma + r_\gamma^2 + r'_\gamma r_m \sqrt{K/n} + r'_\gamma r_\gamma \sqrt{K/n})\right\}. \end{aligned}$$

After summarizing all bounds above and dropping some negligible terms, we conclude

$$\begin{aligned} |v_n^T U^T \hat{G}_n^{-1} \Delta_1| &= \mathcal{O}_P\left\{\|v_n\| \beta_n^{-1} (n^{-1/2} + K^{-p/(d+1)}) (1 + \beta_n^{-1} \rho^{-1} K \log n/n)\right\} \\ &+ o_P\left\{\|v_n\| \beta_n^{-2} (\log n) K^{3/2} n^{-3/2} \rho^{-1} (r'_\gamma + r_m + r_\gamma)\right\} \\ &+ o_P\left\{\|v_n\| \beta_n^{-1} (r_\gamma/\sqrt{n} + r_m r_\gamma + r_\gamma^2)\right\} \\ &+ o_P\left\{\|v_n\| \beta_n^{-2} (\log n) K n^{-1} \rho^{-1} (r_m r_\gamma + r_\gamma^2 + r'_\gamma r_m \sqrt{K/n} + r'_\gamma r_\gamma \sqrt{K/n})\right\} \quad (\text{S100}) \\ &= \mathcal{O}_P\left\{\|v_n\| \beta_n^{-1} (n^{-1/2} + K^{-p/(d+1)}) (1 + \beta_n^{-1} \rho^{-1} K \log n/n)\right\} \\ &+ o_P\left\{\|v_n\| \beta_n^{-2} (\log n) K^{3/2} n^{-3/2} \rho^{-1} (r'_\gamma + r_m + r_\gamma)\right\} \\ &+ o_P\left\{\|v_n\| \beta_n^{-1} (r_\gamma/\sqrt{n} + r_m r_\gamma + r_\gamma^2)\right\}, \end{aligned}$$

because  $\sqrt{K/n} \prec 1$  and  $r_m r_\gamma + r_\gamma^2 + r'_\gamma r_m \sqrt{K/n} + r'_\gamma r_\gamma \sqrt{K/n} \lesssim r'_\gamma + r_m + r_\gamma$ , due to Assumption S3 and  $r_m, r_\gamma, r'_\gamma \lesssim 1$ .

690

**Bound of  $|v_n^T U^T \hat{G}_n^{-1} \Delta_2|$**  We decompose

$$\begin{aligned} |v_n^T U^T \hat{G}_n^{-1} \Delta_2| &= \rho |v_n^T U^T \hat{G}_n^{-1} \hat{Q}_n \phi^*| \\ &\leq \rho |v_n^T U^T \hat{G}_n^{-1} (\hat{Q}_n - Q_n) \phi^*| + \rho |v_n^T U^T \hat{G}_n^{-1} Q_n \phi^*|. \end{aligned} \quad (\text{S101})$$

For the first term on the right-hand side, we have

$$\rho v_n^T U^T \hat{G}_n^{-1} (\hat{Q}_n - Q_n) \phi^* = \rho v_n^T U^T \hat{U} \hat{\Sigma}^{-1} \hat{U}^T (\hat{Q}_n - Q_n) \phi^* + \rho v_n^T U^T \hat{U}_\perp \hat{\Sigma}_\perp^{-1} \hat{U}_\perp^T (\hat{Q}_n - Q_n) \phi^*.$$

Then by Lemmas S5 and S8, we have,

$$\begin{aligned} |\rho v_n^T U^T \hat{U} \hat{\Sigma}^{-1} \hat{U}^T (\hat{Q}_n - Q_n) \phi^*| &\leq \rho \|v_n\| \|\hat{U}^T \hat{U}\|_2 \|\hat{\Sigma}^{-1}\|_2 \|\hat{U}^T\|_2 \|\hat{Q}_n - Q_n\|_2 \|\phi^*\|_2 \\ &= \mathcal{O}_P(\|v_n\| \rho \sqrt{K \log n/n} \beta_n^{-1}), \end{aligned} \quad (\text{S102})$$

and

$$\begin{aligned} |\rho v_n^T U^T \hat{U}_\perp \hat{\Sigma}_\perp^{-1} \hat{U}_\perp^T (\hat{Q}_n - Q_n) \phi^*| &\leq \rho \|v_n\| \|\hat{U}_\perp^T \hat{U}_\perp\|_2 \|\hat{\Sigma}_\perp^{-1}\|_2 \|\hat{U}_\perp^T\|_2 \|\hat{Q}_n - Q_n\|_2 \|\phi^*\|_2 \\ &= \mathcal{O}_P\{\|v_n\| (\log n) K n^{-1} \beta_n^{-1}\}, \end{aligned} \quad (\text{S103})$$

695 which together yield

$$|\rho v_n^T U^T \hat{G}_n^{-1} (\hat{Q}_n - Q_n) \phi^*| = \mathcal{O}_P\{\|v_n\| \sqrt{\log n} \rho K^{1/2} n^{-1/2} \beta_n^{-1} + \|v_n\| (\log n) K n^{-1} \beta_n^{-1}\}. \quad (\text{S104})$$

For the second term on the right-hand side of (S101), we have by (S4),

$$Q_n \phi^* = E\{\Psi(X, T) \tilde{\tau}(X, T)\}.$$

Since  $U_\perp^T \Psi(X, T)$  is a function only of  $X$ , by the law of total expectation,

$$\begin{aligned} U_\perp^T Q_n \phi^* &= E\{U_\perp^T \Psi(X, T) \tilde{\tau}(X, T)\} \\ &= E[U_\perp^T \Psi(X, T) E\{\tilde{\tau}(X, T) | X\}] \\ &= 0, \end{aligned}$$

as  $E\{\tilde{\tau}(X, T) | X = x\} = E\{\tau - E(\tau | X) | X = x\} = E(\tau | X = x) - E(\tau | X = x) = 0$ . Thus we have

$$Q_n \phi^* = U U^T Q_n \phi^* + U_\perp U_\perp^T Q_n \phi^* = U U^T Q_n \phi^*.$$

700 We then have

$$\begin{aligned} \rho v_n^T U^T \hat{G}_n^{-1} Q_n \phi^* &= \rho v_n^T U^T \hat{G}_n^{-1} U U^T Q_n \phi^* \\ &= \rho v_n^T U^T \hat{U} \hat{\Sigma}^{-1} \hat{U}^T U U^T Q_n \phi^* + \rho v_n^T U^T \hat{U}_\perp \hat{\Sigma}_\perp^{-1} \hat{U}_\perp^T U U^T Q_n \phi^*. \end{aligned}$$

Similar to (S102) and (S103), we have

$$\begin{aligned} |\rho v_n^T U^T \hat{U} \hat{\Sigma}^{-1} \hat{U}^T U U^T Q_n \phi^*| &= \mathcal{O}_P(\rho \|v_n\| \beta_n^{-1}) \\ |\rho v_n^T U^T \hat{U}_\perp \hat{\Sigma}_\perp^{-1} \hat{U}_\perp^T U U^T Q_n \phi^*| &= \mathcal{O}_P\{\|v_n\| (\log n) K n^{-1} \beta_n^{-2}\}, \end{aligned}$$

which yields  $|\rho v_n^T U^T \hat{G}_n^{-1} Q_n \phi^*| = \mathcal{O}_P\{\rho \|v_n\| \beta_n^{-1} + \|v_n\| (\log n) K n^{-1} \beta_n^{-2}\}$ . This combining with (S104) results that

$$\begin{aligned} |v_n^T U^T \hat{G}_n^{-1} \Delta_2| &= \mathcal{O}_P\{\|v_n\| \sqrt{\log n} \rho K^{1/2} n^{-1/2} \beta_n^{-1} + \|v_n\| (\log n) K n^{-1} \beta_n^{-1} + \|v_n\| \rho \beta_n^{-1} + \|v_n\| (\log n) K n^{-1} \beta_n^{-2}\} \\ &= \mathcal{O}_P\{\rho \|v_n\| \beta_n^{-1} + \|v_n\| \beta_n^{-2} (\log n) K n^{-1}\}, \end{aligned} \quad (\text{S105})$$

noting here we use the fact  $\sqrt{\log n} \rho K n^{-1/2} \beta_n^{-1} \prec \rho \sqrt{K} \beta_n^{-1}$  under Assumption S3.

Summary of convergence rates We now prove the convergence rate results in Theorem ???. Combining (S85), (S86), (S89), (S100), and (S105), we finally have 705

$$\begin{aligned} &|\hat{\tau}(x_0, t_0) - \tau(x_0, t_0)| \\ &\leq r(n, K, \beta_n, \rho, r_m, r_\gamma, r'_\gamma) \\ &= \mathcal{O}_P\left\{\|v_n\| \beta_n^{-1} (n^{-1/2} + K^{-p/(d+1)}) (1 + \beta_n^{-1} \rho^{-1} K \log n / n) + \|v_n\| \beta_n^{-1} \rho + \|v_n\| \beta_n^{-2} (\log n) K n^{-1}\right\} \\ &\quad + \mathcal{O}_P\left\{\|v_n\| \beta_n^{-1} (r_\gamma / \sqrt{n} + r_m r_\gamma + r_\gamma^2) + \|v_n\| \beta_n^{-2} (\log n) \rho^{-1} K^{3/2} n^{-3/2} (r'_\gamma + r_m + r_\gamma)\right\}. \end{aligned} \quad (\text{S106})$$

Here  $\|v_n\| \leq \|U\|_2 \|\Psi(x_0, t_0) - \Psi(x_0, 0)\| = \|\Psi(x_0, t_0) - \Psi(x_0, 0)\|$  depends on  $x_0$  and  $t_0$ , and it has a general bound (S88).

When  $\beta_n \asymp 1$ ,  $r_m, r_\gamma, r_{\gamma'} \lesssim n^{-1/4}$ , and  $p > d + 1$ , the above bound can be simplified to

$$\begin{aligned}
& |\hat{\tau}(x_0, t_0) - \tau(x_0, t_0)| \\
&= \mathcal{O}_P \left\{ \|v_n\| (n^{-1/2} + K^{-p/(d+1)}) (1 + \rho^{-1} K \log n/n) + \|v_n\| \rho + \|v_n\| (\log n) K n^{-1} \right\} \\
&+ o_P \left\{ \|v_n\| n^{-1/2} + \|v_n\| (\log n) \rho^{-1} K^{3/2} n^{-7/4} \right\} \\
&= \mathcal{O}_P \left( \|v_n\| n^{-1/2} \right) \\
&+ \mathcal{O}_P \left\{ \|v_n\| K^{-p/(d+1)} (1 + \rho^{-1} K \log n/n) + \|v_n\| \rho + \|v_n\| (\log n) K n^{-1} \right\} \\
&+ o_P \left\{ \|v_n\| (\log n) \rho^{-1} K^{3/2} n^{-7/4} \right\} \\
&= \mathcal{O}_P \left( \sqrt{K/n} + K^{1/2-p/(d+1)} \right) \\
&+ \mathcal{O}_P \left\{ (\sqrt{K/n} + K^{1/2-p/(d+1)}) (\rho^{-1} K \log n/n) + \rho K^{1/2} + (\log n) K^{3/2} n^{-1} \right\} \\
&+ o_P \left\{ (\log n) \rho^{-1} K^2 n^{-7/4} \right\},
\end{aligned} \tag{S107}$$

where the last equality is derived by  $\|v_n\| \lesssim \sqrt{K}$  by (S88). We first focus on the first term of (S107). In the following, we balance the rate of (S107) by selecting  $K \asymp n^{(d+1)/(2p)}$ , and then

$$\sqrt{K/n} + K^{1/2-p/(d+1)} \asymp n^{-1/2+(d+1)/(4p)}.$$

Now we show the second term in (S107) is negligible. When  $\rho \asymp n^{-1+(d+1)/(2p)} \log n$ , we have

$$\begin{aligned}
\rho^{-1} K \log n/n &\prec n^{1-(d+1)/(2p)} \cdot n^{(d+1)/(2p)} \cdot n^{-1} \\
&= 1.
\end{aligned}$$

This implies  $(\sqrt{K/n} + K^{1/2-p/(d+1)}) (\rho^{-1} K \log n/n) \prec (\sqrt{K/n} + K^{1/2-p/(d+1)})$ , which is negligible compared with the rate of the first term in (S107). On the other hand, since  $\rho \lesssim n^{-1/2}$ , we have

$$\rho K^{1/2} \lesssim \sqrt{K/n},$$

which implies that  $\rho K^{1/2}$  is also negligible compared with the first term in (S107). We also have

$$\begin{aligned}
(\log n) K^{3/2} n^{-1} &\asymp (\log n) n^{-1+(d+1)/(2p)} \\
&= (\log n) (n^{-1/2+(d+1)/(4p)})^2 \\
&\prec n^{(d+1)/(2p)} \cdot n^{-1} \\
&\asymp \sqrt{K/n} + K^{1/2-p/(d+1)},
\end{aligned}$$

where the inequality is because that  $n^{-1/2+(d+1)/(4p)}$  is polynomially decaying when  $p > d + 1$ . Summarizing the results above, we conclude

$$(\sqrt{K/n} + K^{1/2-p/(d+1)}) (\rho^{-1} K \log n/n) + \rho K^{1/2} + (\log n) K^{3/2} n^{-1} \prec \sqrt{K/n} + K^{1/2-p/(d+1)},$$

and thus the second term in (S107) is negligible. Finally

$$\begin{aligned}
(\log n) \rho^{-1} K^2 n^{-7/4} &\prec n^{1-(d+1)/2p} \cdot n^{(d+1)/p} \cdot n^{-7/4} \\
&= n^{-1/2+(d+1)/4p} \cdot n^{-1/4+(d+1)/4p} \\
&\prec n^{-1/2+(d+1)/4p},
\end{aligned} \tag{S108}$$

since  $-1/4 + (d+1)/(4p) < 0$  due to  $d+1 < p$ . Thus the third term in (S107) is also negligible compared with the first term in (S107). In summary, the first term in (S107) is optimized as  $\mathcal{O}_P(n^{-1/2+(d+1)/(4p)})$  when  $K \asymp n^{(d+1)/(2p)}$ . Moreover, when selecting  $n^{-1+(d+1)/(2p)} \log n \prec \rho \lesssim$

$n^{-1/2}$ , other terms than the first term in (S107) are negligible, and thus the whole rate is minimized to  $\mathcal{O}_P(n^{-1/2+(d+1)/(4p)})$ .

**Central limiting distribution** In this part, we show the central limiting theorem (CLT) result for our proposed estimator. In the previous parts, if carefully tracking the derivations, we can show by (S107) that

$$|\hat{\tau}(x_0, t_0) - \tau(x_0, t_0)| = v_n^T U^T \tilde{U} \tilde{\Sigma}^{-1} \tilde{U}^T U U^T \Delta_{1,1} + R_n, \quad (\text{S109})$$

where,

$$R_n = \mathcal{O}_P\{\|v_n\| K^{-p/(d+1)}(1 + \rho^{-1} K \log n/n) + \|v_n\| \rho + \|v_n\|(\log n) K n^{-1}\} + o_P\{\|v_n\|(\log n) \rho^{-1} K^{3/2} n^{-7/4}\}. \quad (\text{S110})$$

This is because only the term  $v_n^T U^T \tilde{U} \tilde{\Sigma}^{-1} \tilde{U}^T U U^T \Delta_{1,1}$  in (S96) produces the rate term  $\mathcal{O}_P\{\|v_n\| n^{-1/2}\}$ , on the right-hand side of the second equality in (S107). In the following, we will first show the limiting distribution of the first term  $v_n^T U^T \tilde{U} \tilde{\Sigma}^{-1} \tilde{U}^T U U^T \Delta_{1,1}$  on the right-hand side of (S109). We then show that the second term in (S109) is negligible. Finally, we will show the consistency of the our asymptotic variance estimator, which helps us to construct the confidence interval.

First we have

$$\begin{aligned} \sqrt{n} \tilde{\sigma}^{-1} v_n^T U^T \tilde{U} \tilde{\Sigma}^{-1} \tilde{U}^T U U^T \Delta_{1,1} &= \sqrt{n} \tilde{\sigma}^{-1} P_n \left[ \kappa_n(X, T) [Y - m(X) - \tau(X, T) + E\{\tau(X, T) | X\}] \right] \\ &= \sum_{i=1}^n \xi_n(X_i, T_i, Y_i), \end{aligned} \quad (\text{S111})$$

where we define

$$\begin{aligned} \tilde{\sigma} &= \sqrt{E[\kappa_n^2(X, T) \{Y - \mu(X, T)\}^2]} \\ \kappa_n(x, t) &= v_n^T U^T \tilde{U} \tilde{\Sigma}^{-1} \tilde{U}^T U U^T \{\Psi(x, t) - \Gamma(x)\} \\ \xi_n(x, t, y) &= \frac{1}{\sqrt{n} \tilde{\sigma}} \kappa_n(x, t) [y - m(x) - \tau(x, t) + E\{\tau(X, T) | X = x\}] \\ &= \frac{1}{\sqrt{n} \tilde{\sigma}} \kappa_n(x, t) [y - E(Y | X = x) - \mu(x, t) + \mu(x, 0) + E\{\mu(X, T) | X = x\} - E\{\mu(X, 0) | X = x\}] \\ &= \frac{1}{\sqrt{n} \tilde{\sigma}} \kappa_n(x, t) [y - E(Y | X = x) - \mu(x, t) + \mu(x, 0) + E(Y | X = x) - \mu(x, 0)] \\ &= \frac{1}{\sqrt{n} \tilde{\sigma}} \kappa_n(x, t) \{y - \mu(x, t)\}, \end{aligned} \quad (\text{S112})$$

recalling that  $\mu(x, t) = E(Y | X = x, T = t)$ . We now verify (S111) satisfies the Lindberg's condition for the CLT. We emphasize  $v_n^T U^T \tilde{U} \tilde{\Sigma}^{-1} \tilde{U}^T U U^T$  is a deterministic vector independent of samples. Therefore,  $\xi_n(X_i, T_i, Y_i)$  with  $i = 1, \dots, n$ , are i.i.d. samples with

$$\begin{aligned} E\{\xi_n(X, T, Y)\} &= \frac{1}{\sqrt{n} \tilde{\sigma}} E \left[ E[\kappa_n(X, T) \{Y - \mu(X, T)\} | X, T] \right] \\ &= \frac{1}{\sqrt{n} \tilde{\sigma}} E \left[ \kappa_n(X, T) E[Y - \mu(X, T) | X, T] \right] \\ &= 0. \end{aligned} \quad (\text{S113})$$

Therefore we have

$$\text{Var} \left\{ \sum_{i=1}^n \xi_n(X_i, T_i, Y_i) \right\} = \frac{1}{\tilde{\sigma}^2} \text{Var} \left[ \kappa_n(X, T) \{Y - \mu(X, T)\} \right] = 1. \quad (\text{S114})$$

Next we derive the lower bound of  $\tilde{\sigma}$ . By definition, we have

$$\begin{aligned} \tilde{\sigma}^2 &= v_n^\top U^\top \tilde{U} \tilde{\Sigma}^{-1} \tilde{U}^\top U U^\top E \left[ \left\{ \Psi(X, T) - \Gamma(X) \right\} \left\{ \Psi(X, T) - \Gamma(X) \right\}^\top \left\{ Y - \mu(X, T) \right\}^2 \right] U U^\top \tilde{U} \tilde{\Sigma}^{-1} \tilde{U}^\top U v_n. \end{aligned} \quad (\text{S115})$$

Observe that by the law of total expectation,

$$\begin{aligned} &E \left[ \left\{ \Psi(X, T) - \Gamma(X) \right\} \left\{ \Psi(X, T) - \Gamma(X) \right\}^\top \left\{ Y - \mu(X, T) \right\}^2 \right] \\ &= E \left[ \left\{ \Psi(X, T) - \Gamma(X) \right\} \left\{ \Psi(X, T) - \Gamma(X) \right\}^\top \text{Var}(Y \mid X, T) \right] \\ &\succeq c_1 E \left[ \left\{ \Psi(X, T) - \Gamma(X) \right\} \left\{ \Psi(X, T) - \Gamma(X) \right\}^\top \right] \\ &= c_1 R_n, \end{aligned} \quad (\text{S116})$$

740 since  $\text{Var}(Y \mid X, T)$  is uniformly lower bounded by some fixed  $c_1 > 0$  under Assumption S5. Combining (S115) and (S116), we have

$$\begin{aligned} \tilde{\sigma}^2 &\geq c_1 v_n^\top U^\top \tilde{U} \tilde{\Sigma}^{-1} \tilde{U}^\top U U^\top R_n U U^\top \tilde{U} \tilde{\Sigma}^{-1} \tilde{U}^\top U v_n \\ &= c_1 v_n^\top U^\top \tilde{U} \tilde{\Sigma}^{-1} \tilde{U}^\top U U^\top U \Sigma U^\top U U^\top \tilde{U} \tilde{\Sigma}^{-1} \tilde{U}^\top U v_n \\ &= c_1 v_n^\top M_{clt} v_n, \end{aligned} \quad (\text{S117})$$

where  $M_{clt} = U^\top \tilde{U} \tilde{\Sigma}^{-1} \tilde{U}^\top U U^\top U \Sigma U^\top U U^\top \tilde{U} \tilde{\Sigma}^{-1} \tilde{U}^\top U$  is a  $\zeta \times \zeta$  matrix. Its smallest singular value can be bounded by Lemma S8,

$$\begin{aligned} \sigma_{\min}(M_{clt}) &\geq \sigma_{\min}(U^\top \tilde{U}) \sigma_{\min}(\tilde{\Sigma}^{-1} \tilde{U}^\top U U^\top U \Sigma U^\top U U^\top \tilde{U} \tilde{\Sigma}^{-1} \tilde{U}^\top U) \\ &\geq \sigma_{\min}(U^\top \tilde{U}) \sigma_{\min}(\tilde{\Sigma}^{-1}) \sigma_{\min}(\tilde{U}^\top U U^\top U \Sigma U^\top U U^\top \tilde{U} \tilde{\Sigma}^{-1} \tilde{U}^\top U) \\ &\geq \dots \\ &\geq \sigma_{\min}(U^\top \tilde{U}) \sigma_{\min}(\tilde{\Sigma}^{-1}) \sigma_{\min}(\tilde{U}^\top U) \sigma_{\min}(U^\top U) \sigma_{\min}(\Sigma) \sigma_{\min}(U^\top U) \sigma_{\min}(U^\top \tilde{U}) \sigma_{\min}(\tilde{\Sigma}^{-1}) \sigma_{\min}(\tilde{U}^\top U) \\ &\gtrsim 1. \end{aligned} \quad (\text{S118})$$

In (S118), we treat  $M_{clt}$  as the multiplication of nine  $\zeta \times \zeta$  matrices  $U^\top \tilde{U}, \tilde{\Sigma}^{-1}, \dots, \tilde{U}^\top U$ , where each of them is full-rank with smallest singular values bounded away from 0; see Lemma S8 and note  $U^\top U = I_\zeta$ . Then the first three inequalities in (S118) follow by repeatedly using the fact that

$$\sigma_{\min}(AB) \geq \sigma_{\min}(A) \sigma_{\min}(B),$$

745 for two full-rank and square matrices  $A$  and  $B$ ; see, e.g., Bhatia (2013, Problem III.6.14). Combining (S117) and (S118), we conclude that

$$\begin{aligned} \tilde{\sigma}^2 &\geq \|v_n\|^2 \cdot c_1 (v_n / \|v_n\|)^\top M_{clt} (v_n / \|v_n\|) \\ &\geq \|v_n\|^2 \sigma_{\min}(M_{clt}) \\ &\gtrsim \|v_n\|^2. \end{aligned} \quad (\text{S119})$$

We thus derive the lower bound  $\tilde{\sigma} \gtrsim \|v_n\|$ . On the other hand, we aim at deriving

$$\sum_{i=1}^n E \left[ \left| \xi_n(X_i, T_i, Y_i) \right|^2 1_{\left\{ \left| \xi_n(X_i, T_i, Y_i) \right| > \delta \right\}} \right] \rightarrow 0, \quad (\text{S120})$$

to verify the Lindberg's condition. By Hölder's inequality for fixed  $c_0 > 0$  and any  $\delta > 0$ ,

$$\begin{aligned} & E\left[|\xi_n(X, T, Y)|^2 1\{|\xi_n(X, T, Y)| > \delta\}\right] \\ & \leq \left[E\left\{|\xi_n(X, T, Y)|^{2 \cdot (2+c_0)/2}\right\}\right]^{2/(2+c_0)} \left[E\left[1\{|\xi_n(X, T, Y)| > \delta\}\right]\right]^{1-2/(2+c_0)} \\ & = \left[E\left\{|\xi_n(X, T, Y)|^{2+c_0}\right\}\right]^{2/(2+c_0)} \left[\text{pr}\{|\xi_n(X, T, Y)| > \delta\}\right]^{1-2/(2+c_0)}. \end{aligned} \quad (\text{S121})$$

For the first factor on the right-hand side of (S121), we have

$$\begin{aligned} & E\left\{|\xi_n(X, T, Y)|^{2+c_0}\right\} \\ & = n^{-(2+c_0)/2} \tilde{\sigma}^{-(2+c_0)} E\left[\kappa_n^{2+c_0}(X, T) |Y - \mu(X, T)|^{2+c_0}\right] \\ & \leq n^{-(2+c_0)/2} \tilde{\sigma}^{-(2+c_0)} \cdot \left|\sup_{(x,t) \in \mathbb{X} \times \mathbb{T}} \kappa_n(x, t)\right|^{c_0} \cdot E\left[\kappa_n^2(X, T) |Y - \mu(X, T)|^{2+c_0}\right] \\ & \lesssim n^{-(2+c_0)/2} K^{c_0/2}, \end{aligned} \quad (\text{S122})$$

where the last inequality follows by  $\tilde{\sigma} \gtrsim \|v_n\|$  and the following bounds.

- 750 • By Lemmas S3 and S6, we have

$$\begin{aligned} \sup_{(x,t) \in \mathbb{X} \times \mathbb{T}} \kappa_n(x, t) & \leq \sup_{(x,t) \in \mathbb{X} \times \mathbb{T}} |v_n^T U^T \tilde{U} \tilde{\Sigma}^{-1} \tilde{U}^T U U^T \{\Psi(x, t) - \Gamma(x)\}| \\ & \leq \|v_n\| \|U\|_2 \|\tilde{U}\|_2 \|\tilde{\Sigma}^{-1}\|_2 \|\tilde{U}\|_2 \|U\|_2^2 (\|\Psi\|_{\mathbb{X} \times \mathbb{T}} + \|\Gamma\|_{\mathbb{X}}) \\ & \lesssim \sqrt{K} \|v_n\|. \end{aligned} \quad (\text{S123})$$

- Similar to (S115), we have

$$\begin{aligned} & E\left\{\kappa_n^2(X, T) |Y - \mu(X, T)|^{2+c_0}\right\} \\ & = v_n^T U^T \tilde{U} \tilde{\Sigma}^{-1} \tilde{U}^T U U^T E\left[\{\Psi(X, T) - \Gamma(X)\} \{\Psi(X, T) - \Gamma(X)\}^T \{Y - \mu(X, T)\}^{2+c_0}\right] U U^T \tilde{U} \tilde{\Sigma}^{-1} \tilde{U}^T U v_n \\ & = v_n^T U^T \tilde{U} \tilde{\Sigma}^{-1} \tilde{U}^T U U^T E\left[\{\Psi(X, T) - \Gamma(X)\} \{\Psi(X, T) - \Gamma(X)\}^T E\left[\{Y - \mu(X, T)\}^{2+c_0} \mid X, T\right]\right] U U^T \tilde{U} \tilde{\Sigma}^{-1} \tilde{U}^T U v_n \\ & \lesssim v_n^T U^T \tilde{U} \tilde{\Sigma}^{-1} \tilde{U}^T U U^T E\left[\{\Psi(X, T) - \Gamma(X)\} \{\Psi(X, T) - \Gamma(X)\}^T\right] U U^T \tilde{U} \tilde{\Sigma}^{-1} \tilde{U}^T U v_n \\ & = v_n^T U^T \tilde{U} \tilde{\Sigma}^{-1} \tilde{U}^T U U^T R_n U U^T \tilde{U} \tilde{\Sigma}^{-1} \tilde{U}^T U v_n \\ & \leq \|v_n\| \|U\|_2 \cdots \|v_n\| \\ & \lesssim \|v_n\|^2, \end{aligned}$$

where the second equality follows by the law of total expectation, the first inequality follows by (??), and the last inequality is similar to (S123).

We note the bound (S122) actually holds for not only  $c_0$  but also all  $c \in [0, c_0]$  with similar arguments. Thus when  $c = 0$ , one has  $E|\xi_n(X, T, Y)|^2 \lesssim n^{-1}$ . Then for the second factor on the right-hand side of (S121), by Chebyshev's inequality, 755

$$\text{pr}\{|\xi_n(X, T, Y)| > \delta\} \leq \frac{E|\xi_n(X, T, Y)|^2}{\delta^2} \lesssim n^{-1}, \quad (\text{S124})$$

with fixed  $\delta > 0$ . Combining (S121), (S122), and (S124), we conclude

$$\begin{aligned} \sum_{i=1}^n E\left[|\xi_n(X, T, Y)|^2 1\{|\xi_n(X, T, Y)| > \delta\}\right] & \lesssim n \cdot (n)^{-1} \cdot K^{c_0/(2+c_0)} \cdot n^{-1+2/(2+c_0)} \\ & = (K/n)^{c_0/(2+c_0)} \\ & \rightarrow 0, \end{aligned} \quad (\text{S125})$$



under Assumption S3. Thus (S120) is verified. By (S113), (S114), and (S125), the conditions of the Lindeberg-Feller CLT are verified. Thus we have

$$\sqrt{n}\tilde{\sigma}^{-1}v_n^T U^T \tilde{U} \tilde{\Sigma}^{-1} \tilde{U}^T U U^T \Delta_{1,1} \rightsquigarrow \mathcal{N}(0, 1). \quad (\text{S126})$$

By (S110) and (S119),  $K \asymp n^{\epsilon_{clt} + (d+1)/2p}$  with  $\epsilon_{clt} < 1/2 - (d+1)/(ep)$  and  $\rho \asymp n^{-1}$ , we have

$$\begin{aligned} & \sqrt{n}\tilde{\sigma}^{-1}R_n \\ &= \mathcal{O}_P\{\sqrt{n}K^{-p/(d+1)}(1 + \rho^{-1}K \log n/n) + \rho\sqrt{n} + (\log n)Kn^{-1/2}\} \\ &+ o_P\{(\log n)\rho^{-1}K^{3/2}n^{-5/4}\} \\ &= o_P(1), \end{aligned} \quad (\text{S127})$$

with similar rate comparison arguments as (S107)–(S108). For example, the rate term  $\rho^{-1}K \log n/n = (\log n)n^{-1/2+(d+1)/(2p)+\epsilon_{clt}} \rightarrow 0$  as  $\epsilon_{clt} < 1/2 - (d+1)/(2p)$ . Other terms can be bounded similarly. Finally combining (S109), (S126), (S127), and applying the Slutsky's theorem leads to (??).

**Confidence interval** We finally prove the confidence interval part of Theorem ?? . First we simplify  $\sigma_n^2$ . From (S87), we have

$$v_n^T U^T = \Psi^T(x_0, t_0) - \Psi^T(x_0, 0). \quad (\text{S128})$$

On the other hand, by Lemma S4 (i), we have  $U_\perp^T \{\Psi(x, t) - \Gamma(x)\} = 0$  and thus

$$\begin{aligned} & E\left[\{\Psi(X, T) - \Gamma(X)\}\{\Psi(X, T) - \Gamma(X)\}^T \{Y - \mu(X, T)\}^2\right] \\ &= UU^T E\left[\{\Psi(X, T) - \Gamma(X)\}\{\Psi(X, T) - \Gamma(X)\}^T \{Y - \mu(X, T)\}^2\right] UU^T \\ &+ U_\perp U_\perp^T E\left[\{\Psi(X, T) - \Gamma(X)\}\{\Psi(X, T) - \Gamma(X)\}^T \{Y - \mu(X, T)\}^2\right] U_\perp U_\perp^T \\ &= UU^T E\left[\{\Psi(X, T) - \Gamma(X)\}\{\Psi(X, T) - \Gamma(X)\}^T \{Y - \mu(X, T)\}^2\right] UU^T \\ &+ U_\perp U_\perp^T E\left[\underbrace{\{U_\perp^T \{\Psi(X, T) - \Gamma(X)\}\}_{=0}}_{=0} \underbrace{\{\Psi(X, T) - \Gamma(X)\}^T U_\perp}_{=0} \{Y - \mu(X, T)\}^2\right] U_\perp U_\perp^T \\ &= UU^T E\left[\{\Psi(X, T) - \Gamma(X)\}\{\Psi(X, T) - \Gamma(X)\}^T \{Y - \mu(X, T)\}^2\right] UU^T. \end{aligned} \quad (\text{S129})$$

By (S115), (S128), and (S129),  $\tilde{\sigma}$  can be simplified to

$$\tilde{\sigma}^2 = \{\Psi(x_0, t_0) - \Psi(x_0, 0)\}^T A_n B_n A_n \{\Psi(x_0, t_0) - \Psi(x_0, 0)\},$$

where  $A_n = \tilde{U} \tilde{\Sigma}^{-1} \tilde{U}^T$  and  $B_n = E[\{\Psi(X, T) - \Gamma(X)\}\{\Psi(X, T) - \Gamma(X)\}^T \{Y - \mu(X, T)\}^2]$ . Recall that in Algorithm ??, our variance estimator is

$$\hat{\sigma}^2 = \tilde{v}_n^T \hat{A}_n \hat{B}_n \hat{A}_n \tilde{v}_n,$$

where we define,

$$\begin{aligned} \hat{A}_n &= \hat{U} \hat{\Sigma}^{-1} \hat{U}^T, \\ \hat{B}_n &= P_n[\{\Psi(X, T) - \hat{\Gamma}(X)\}\{\Psi(X, T) - \hat{\Gamma}(X)\}^T \{Y - \hat{\mu}(X, T)\}^2] \\ \tilde{v}_n &= \Psi(x_0, t_0) - \Psi(x_0, 0). \end{aligned}$$

We then decompose

$$\begin{aligned} \hat{\sigma}^2 - \tilde{\sigma}^2 &= \tilde{v}_n^T \hat{A}_n \hat{B}_n \hat{A}_n \tilde{v}_n - \tilde{v}_n^T A_n B_n A_n \tilde{v}_n \\ &= \tilde{v}_n^T (\hat{A}_n - A_n) \hat{B}_n \hat{A}_n \tilde{v}_n + \tilde{v}_n^T A_n (\hat{B}_n - B_n) \hat{A}_n \tilde{v}_n + \tilde{v}_n^T A_n B_n (\hat{A}_n - A_n) \tilde{v}_n. \end{aligned}$$

By Lemma S8 (v), we have the spectral norms of  $\hat{A}_n, A_n, \hat{B}_n, B_n$  are constantly bounded, while  $\|\hat{A}_n - A_n\|_2, \|\hat{B}_n - B_n\|_2 \rightarrow 0$  wpa1. We thus have wpa1,

$$\begin{aligned}
& |\hat{\sigma}^2 - \tilde{\sigma}^2| \\
& \leq \|\tilde{v}_n\|^2 \|\hat{A}_n - A_n\|_2 \|\hat{B}_n\|_2 \|\hat{A}_n\|_2 + \|\tilde{v}_n\|^2 \|A_n\|_2 \|\hat{B}_n - B_n\|_2 \|\hat{A}_n\|_2 + \|\tilde{v}_n\|^2 \|A_n\|_2 \|B_n\|_2 \|\hat{A}_n - A_n\|_2 \\
& \prec \|\Psi(x_0, t_0) - \Psi(x_0, 0)\|^2 \\
& = \{\Psi(x_0, t_0) - \Psi(x_0, 0)\}^T \{\Psi(x_0, t_0) - \Psi(x_0, 0)\} \\
& = \{\Psi(x_0, t_0) - \Psi(x_0, 0)\}^T U U^T \{\Psi(x_0, t_0) - \Psi(x_0, 0)\} + \{\Psi(x_0, t_0) - \Psi(x_0, 0)\}^T U_\perp U_\perp^T \{\Psi(x_0, t_0) - \Psi(x_0, 0)\} \\
& = \{\Psi(x_0, t_0) - \Psi(x_0, 0)\}^T U U^T \{\Psi(x_0, t_0) - \Psi(x_0, 0)\} \\
& = \|v_n\|^2,
\end{aligned} \tag{S130}$$

where the second and third equalities can be derived similar to (S87). With (S119) and (S130), we have wpa1,

$$\frac{\hat{\sigma}^2}{\tilde{\sigma}^2} = 1 + \frac{\hat{\sigma}^2 - \tilde{\sigma}^2}{\tilde{\sigma}^2} \rightarrow 1,$$

and thus  $\hat{\sigma}^{-1} \tilde{\sigma} \rightarrow 1$  wpa1. Then by (??) and Slutsky's theorem, we finally have

$$\begin{aligned}
\sqrt{n} \hat{\sigma}^{-1} \{\hat{\tau}(x_0, t_0) - \tau(x_0, t_0)\} &= \hat{\sigma}^{-1} \tilde{\sigma} \cdot \sqrt{n} \tilde{\sigma}^{-1} \{\hat{\tau}(x_0, t_0) - \tau(x_0, t_0)\} \\
&\rightsquigarrow \mathcal{N}(0, 1).
\end{aligned}$$

□

## REFERENCES

- BELLONI, A., CHERNOZHUKOV, V., CHETVERIKOV, D. & FERNÁNDEZ-VAL, I. (2019). Conditional quantile processes based on series or many regressors. *J. Econom.* **213**, 4–29.
- BELLONI, A., CHERNOZHUKOV, V., CHETVERIKOV, D. & KATO, K. (2015). Some new asymptotic theory for least squares series: Pointwise and uniform results. *J. Econom.* **186**, 345–366.
- BHATIA, R. (2013). *Matrix Analysis*, vol. 169. Springer Science & Business Media.
- CAI, T. T. & ZHANG, A. (2018). Rate-optimal perturbation bounds for singular subspaces with applications to high-dimensional statistics. *Ann. Stat.* **46**, 60–89.
- CHEN, X. & CHRISTENSEN, T. M. (2015). Optimal uniform convergence rates and asymptotic normality for series estimators under weak dependence and weak conditions. *J. Econom.* **188**, 447–465.
- CUI, Y., PU, H., SHI, X., MIAO, W. & TCHETGEN, E. T. (2020). Semiparametric proximal causal inference. *arXiv:2011.08411*.
- DAVIS, C. & KAHAN, W. M. (1970). The rotation of eigenvectors by a perturbation. iii. *SIAM J. Numer. Anal.* **7**, 1–46.
- DOUGLAS, J., DUPONT, T. & WAHLBIN, L. (1975). Optimal  $l_\infty$  error estimates for galerkin approximations to solutions of two-point boundary value problems. *Math. Comput.* **29**, 475–483.
- ECKART, C. & YOUNG, G. (1936). The approximation of one matrix by another of lower rank. *Psychometrika* **1**, 211–218.
- GOLUB, G. H., HEATH, M. & WAHBA, G. (1979). Generalized cross-validation as a method for choosing a good ridge parameter. *Technometrics* **21**, 215–223.
- GOLUB, G. H. & VAN LOAN, C. F. (2013). *Matrix Computations*, vol. 3. JHU Press.
- HANSEN, B. E. (2014). Nonparametric sieve regression: Least squares, averaging least squares, and cross-validation. *Handbook of Applied Nonparametric and Semiparametric Econometrics and Statistics*, 215–248.
- HORN, R. A. & JOHNSON, C. R. (1991). *Topics in Matrix Analysis*. Cambridge University Press.
- HUANG, J. Z. et al. (2003). Local asymptotics for polynomial spline regression. *Ann. Stat.* **31**, 1600–1635.
- ICHIMURA, H. & TODD, P. E. (2007). Implementing nonparametric and semiparametric estimators. *Handb. Econom.* **6**, 5369–5468.
- KENNEDY, E. H. (2020). Optimal doubly robust estimation of heterogeneous causal effects. *arXiv:2004.14497*.
- KENNEDY, E. H., BALAKRISHNAN, S. & G'SELL, M. (2020). Sharp instruments for classifying compliers and generalizing causal effects. *Ann. Stat.* **48**, 2008–2030.
- KENNEDY, E. H., MA, Z., MCHUGH, M. D. & SMALL, D. S. (2017). Non-parametric methods for doubly robust estimation of continuous treatment effects. *J. R. Stat. Soc. Ser. B* **79**, 1229–1245.

- KUNOTH, A., LYCHE, T., SANGALLI, G. & SERRA-CAPIZZANO, S. (2018). *Splines and PDEs: from Approximation Theory to Numerical Linear Algebra*. Springer. 810
- KÜNZEL, S. R., SEKHON, J. S., BICKEL, P. J. & YU, B. (2019). Metalearners for estimating heterogeneous treatment effects using machine learning. *Proc. Natl. Acad. Sci. U.S.A.* **116**, 4156–4165.
- NEWBY, W. K. (1997). Convergence rates and asymptotic normality for series estimators. *J. Econom.* **79**, 147–168.
- NIE, X. & WAGER, S. (2021). Quasi-oracle estimation of heterogeneous treatment effects. *Biometrika* **108**, 299–319. 815
- RUDELSON, M. (1999). Random vectors in the isotropic position. *J. Funct. Anal.* **164**, 60–72.
- RUDIN, W. (1991). *Functional Analysis*. McGraw-Hill Science/Engineering/Math.
- SCHACKE, K. (2004). *On the Kronecker Product*. Master’s thesis.
- SHI, C., ZHANG, S., LU, W. & SONG, R. (2020). Statistical inference of the value function for reinforcement learning in infinite horizon settings. *arXiv:2001.04515*. 820
- TIKHONOV, A. N., GONCHARSKY, A., STEPANOV, V. & YAGOLA, A. G. (1995). *Numerical Methods for the Solution of Ill-posed Problems*, vol. 328. Springer Science & Business Media.
- VAN DER LAAN, M. J., POLLEY, E. C. & HUBBARD, A. E. (2007). Super learner. *Stat. Appl. Genet. Mol. Biol.* **6**.
- WASSERMAN, L. (2006). *All of Nonparametric Statistics*. Springer Science & Business Media.
- WEYL, H. (1912). Das asymptotische verteilungsgesetz der eigenwerte linearer partieller differentialgleichungen (mit einer anwendung auf die theorie der hohlraumstrahlung). *Math. Ann.* **71**, 441–479. 825
- ZEIDLER, E. (2013). *Nonlinear Functional Analysis and Its Applications: III: Variational Methods and Optimization*. Springer Science & Business Media.

[Received on 2 January 2017. Editorial decision on 8 June 2021]
